# Supplementary material for: Phase transition modelling of relapse in major depressive disorder: Developing and reflecting on an interdisciplinary conceptual translation
Source: arXiv:2302.13895 ancillary file (2023-02-27)

S1 Fig. All considered items

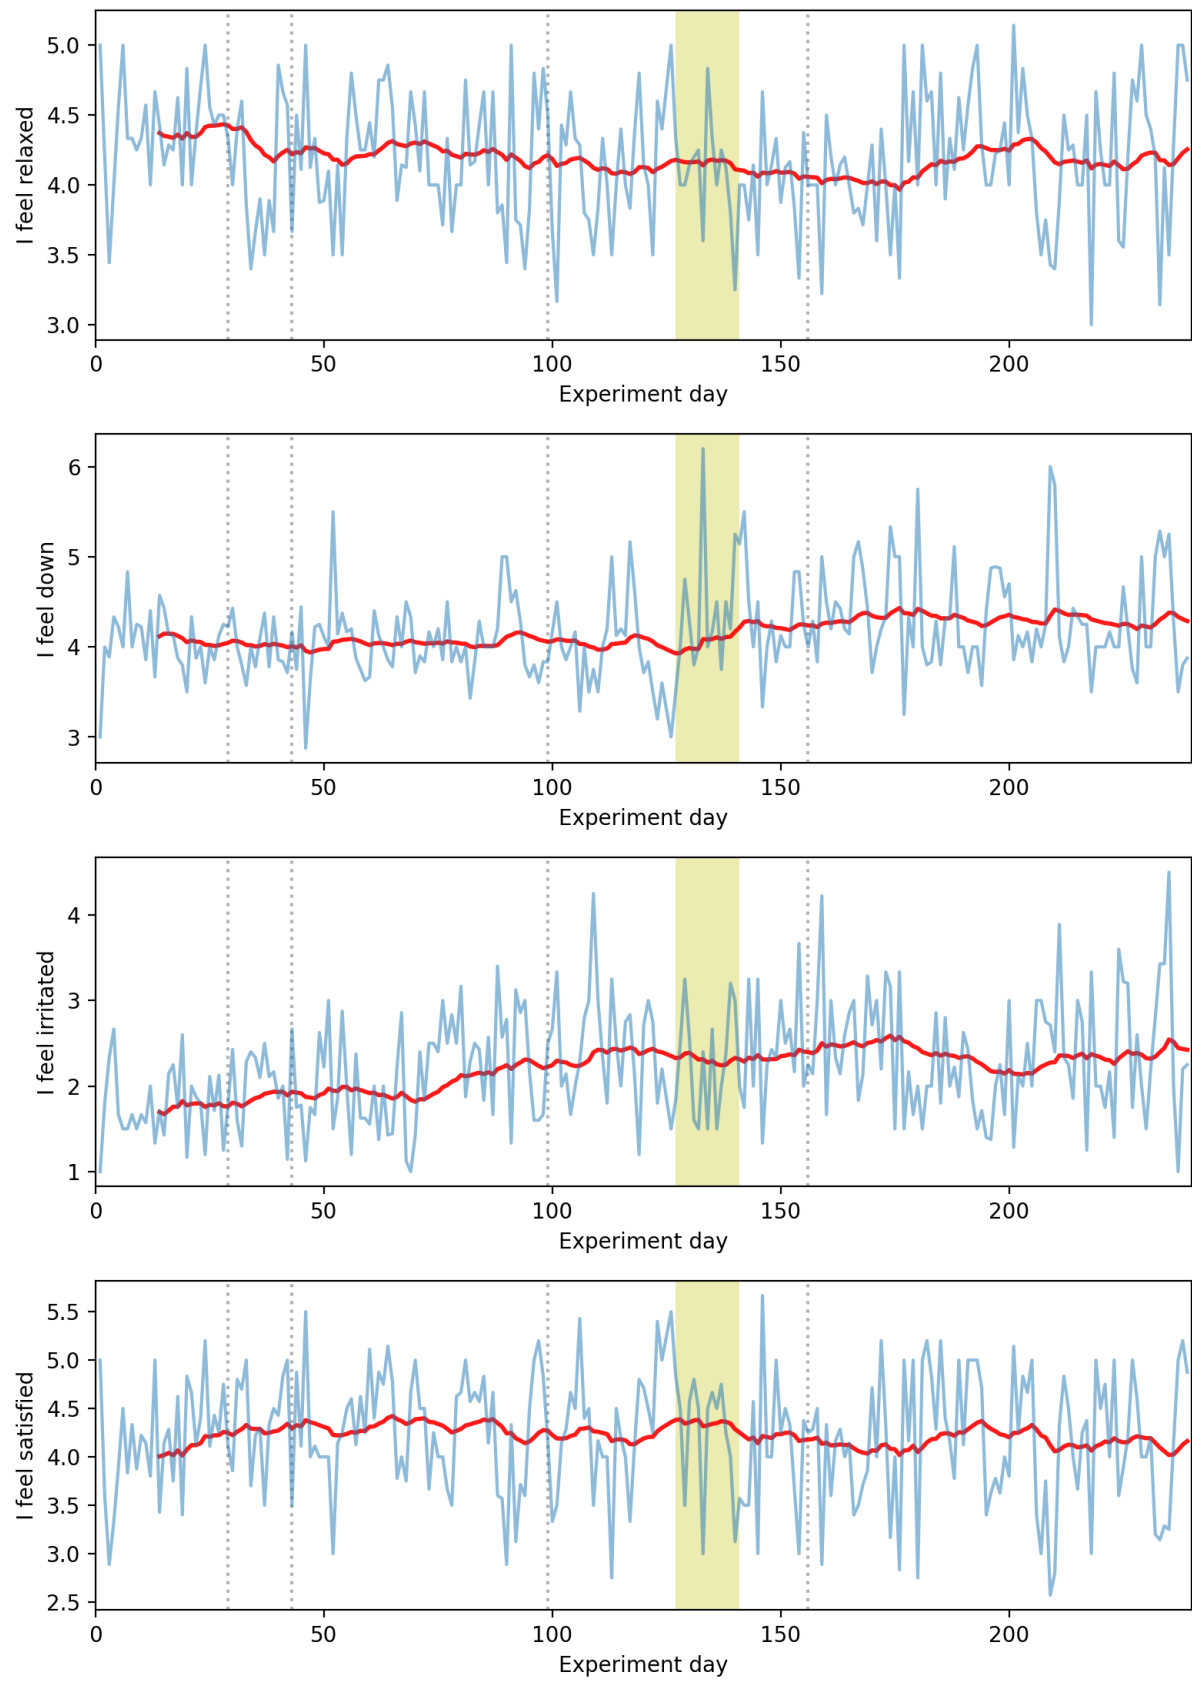

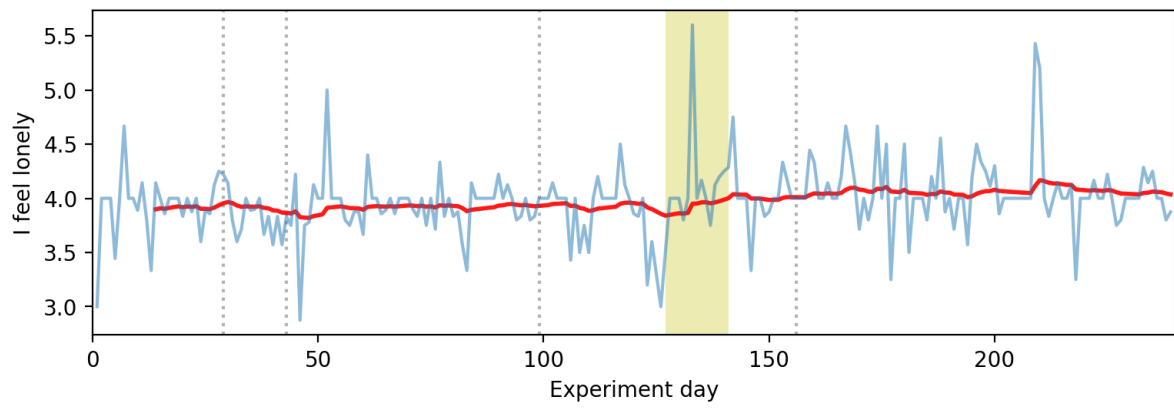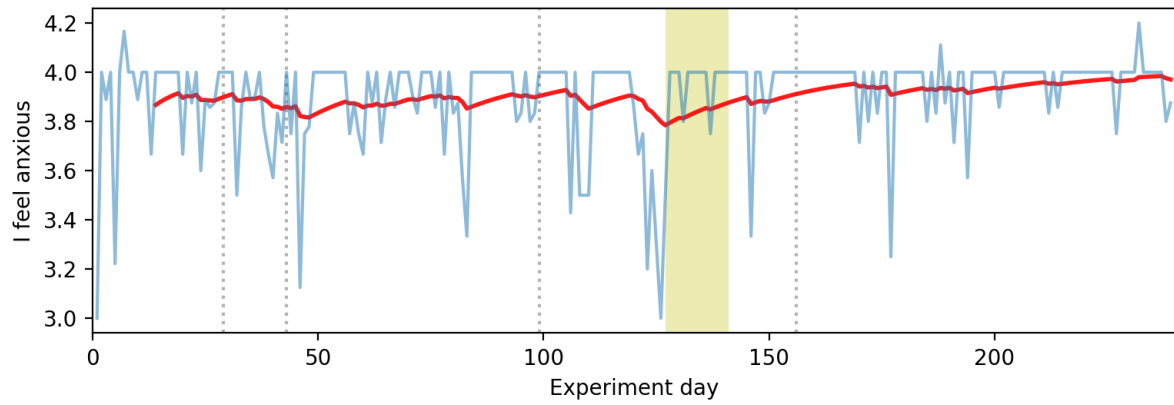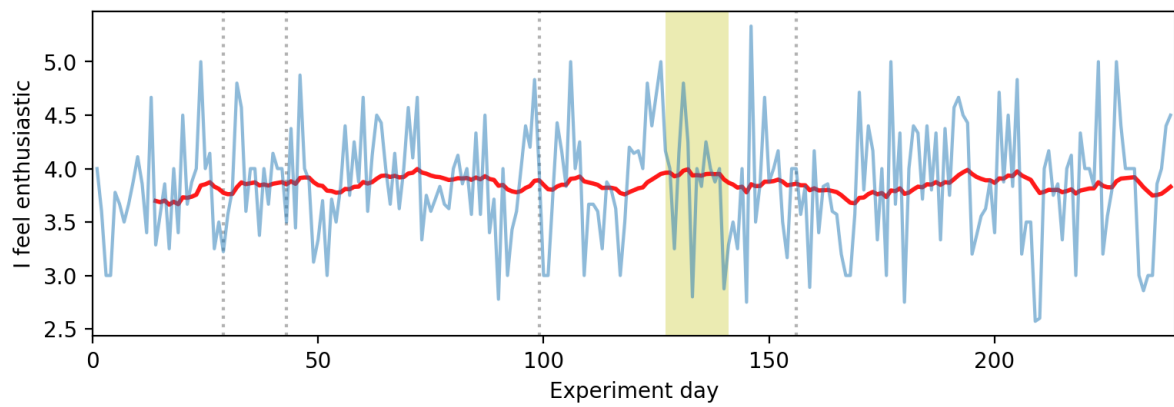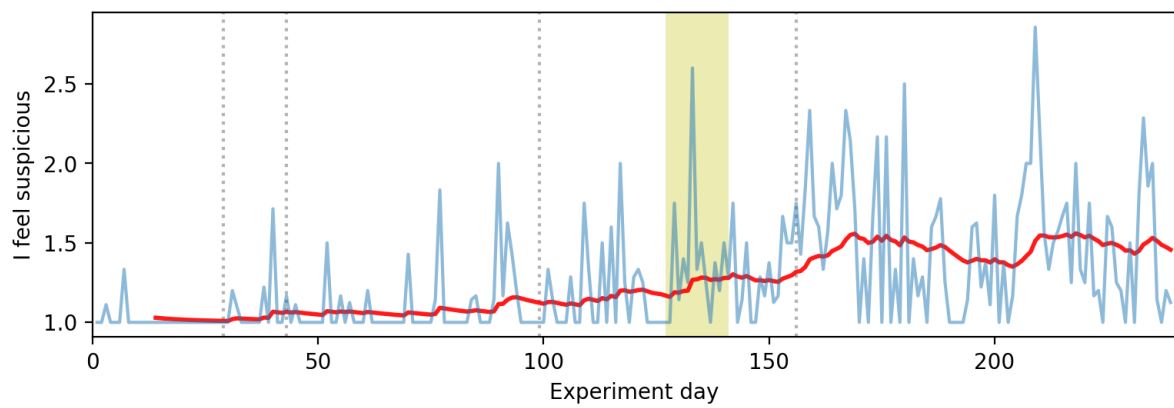

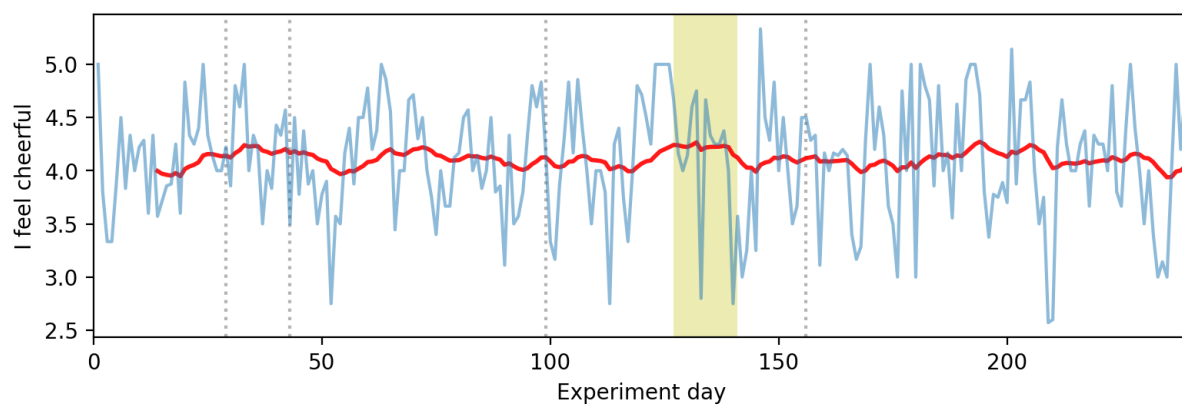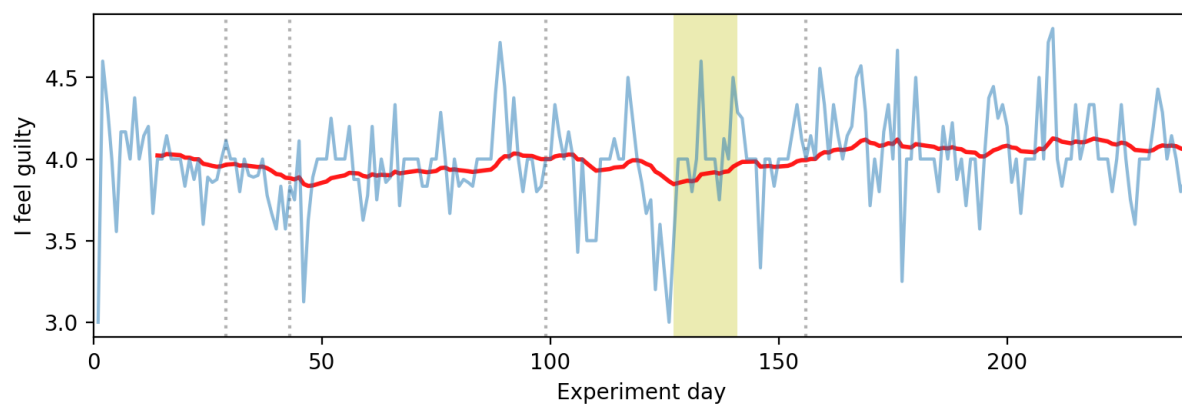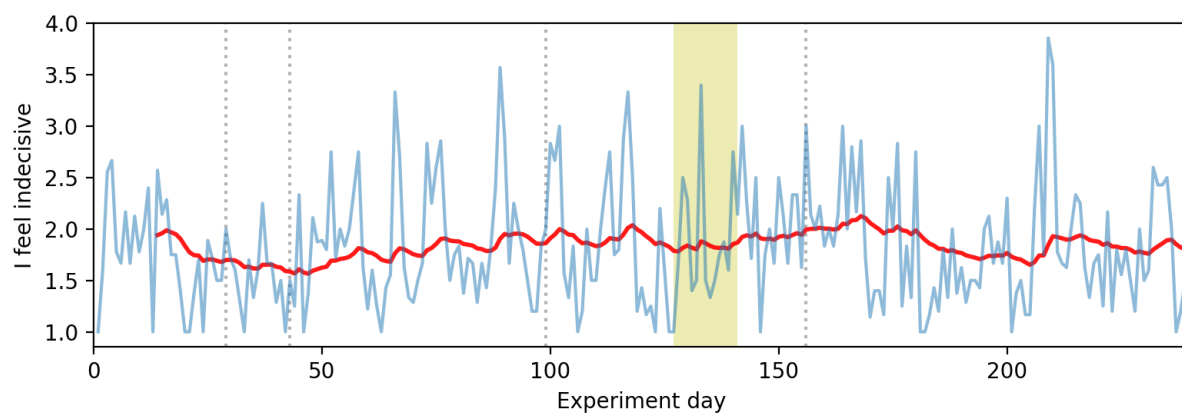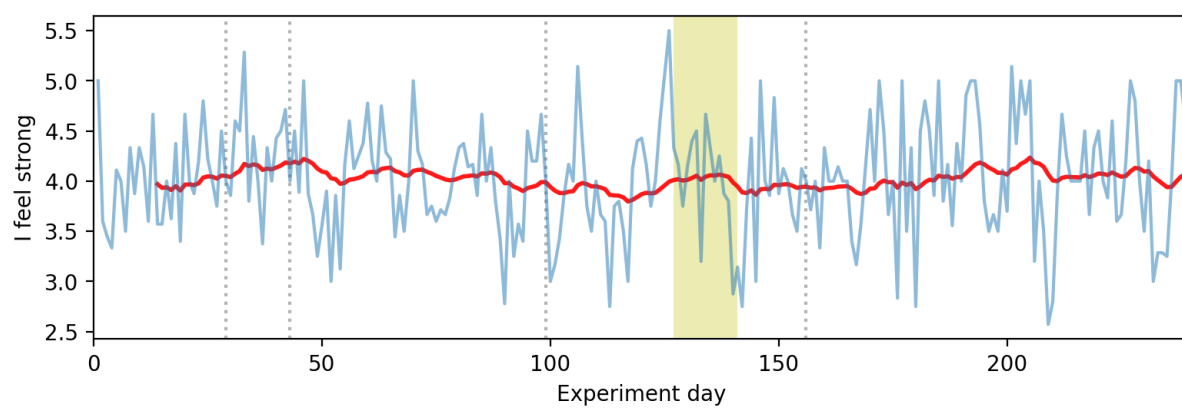

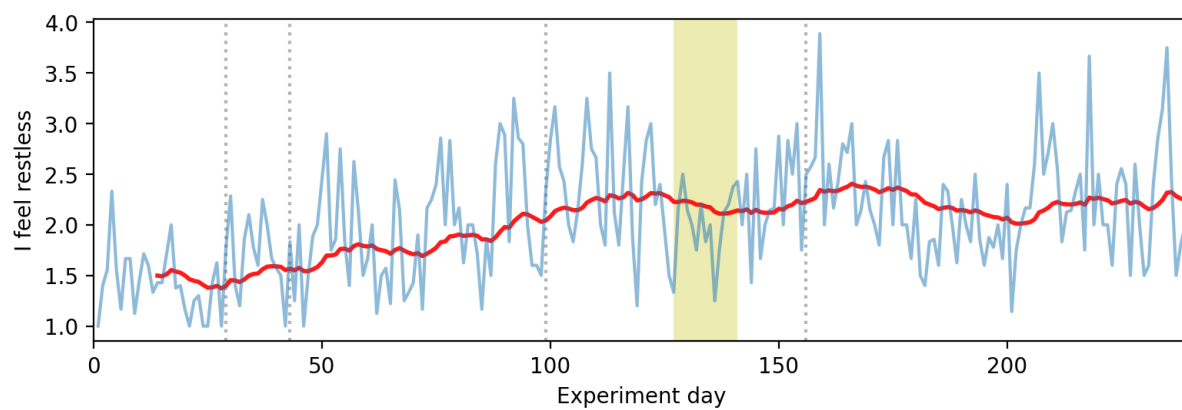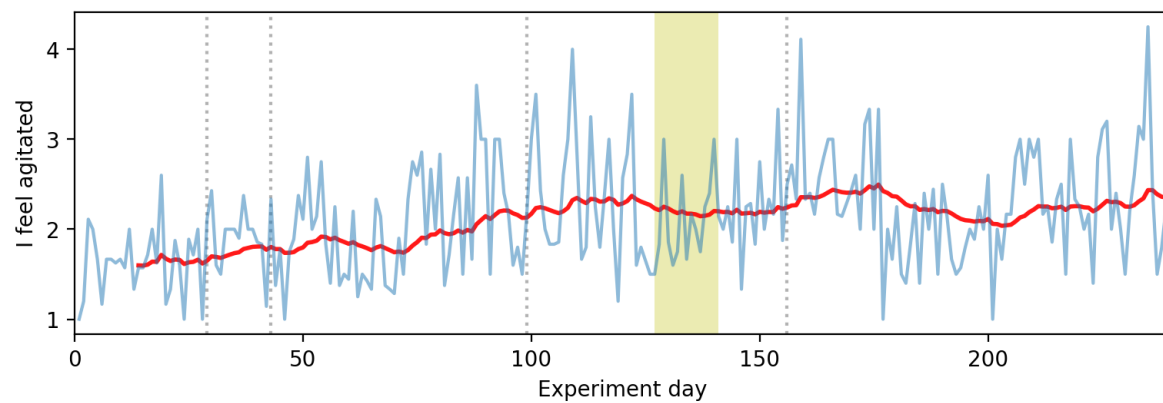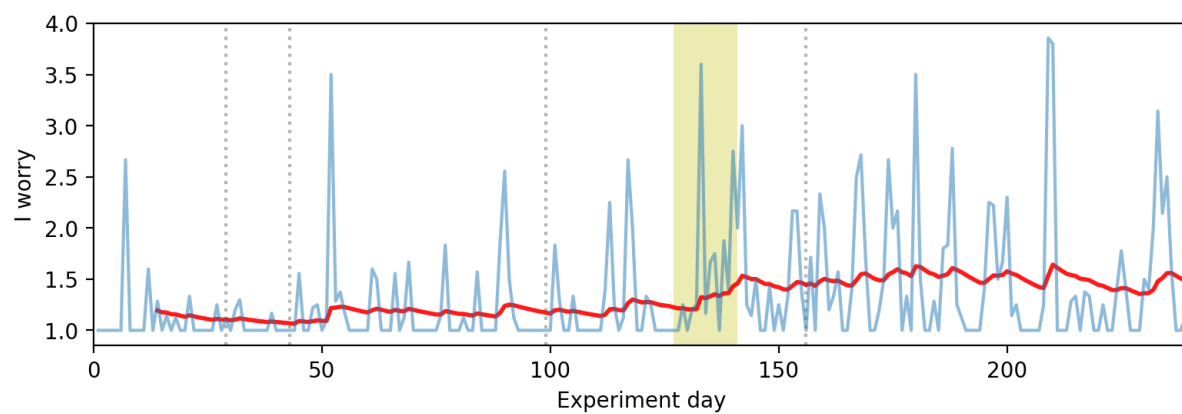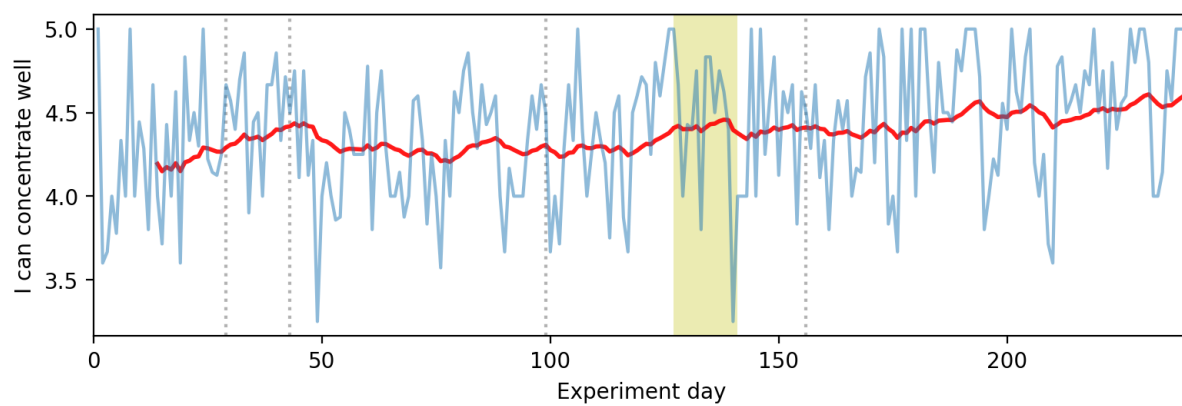

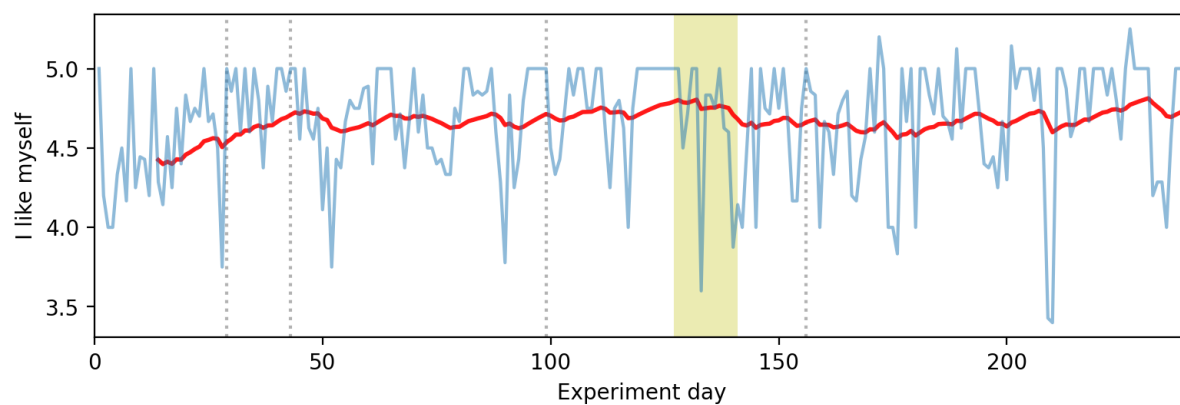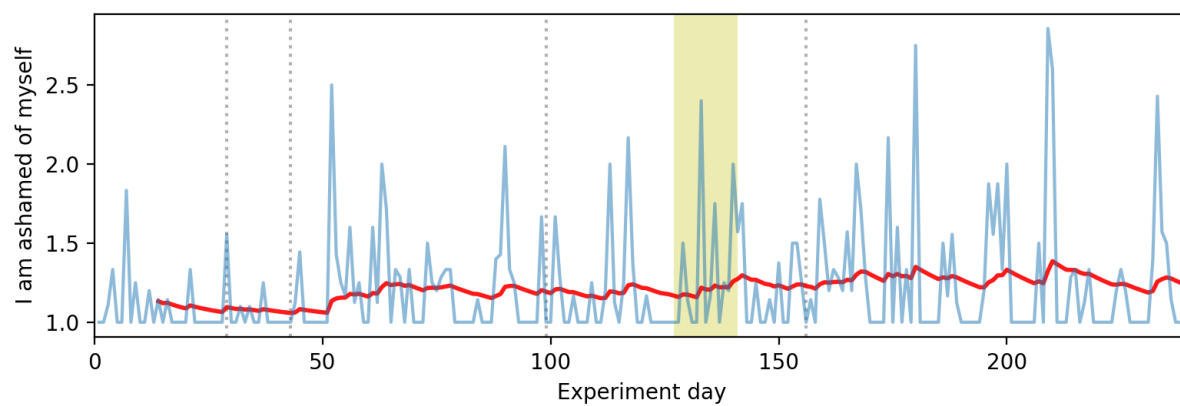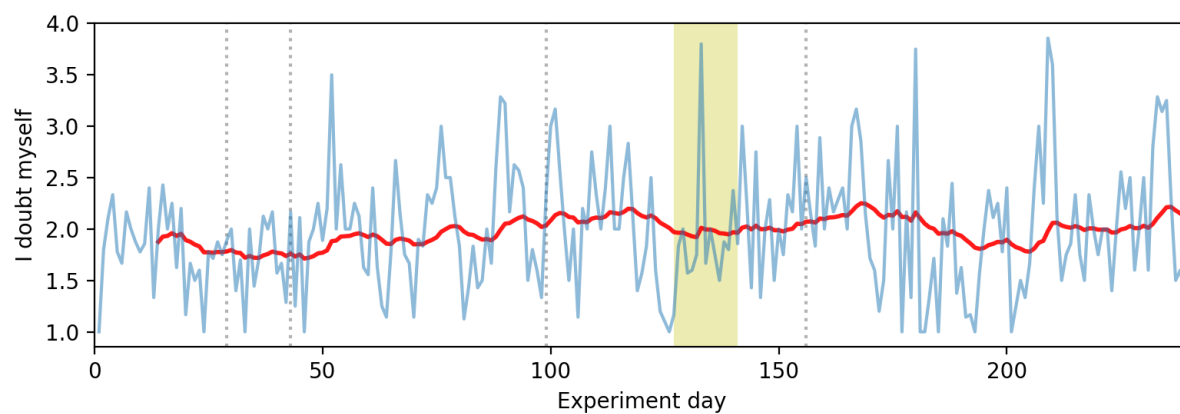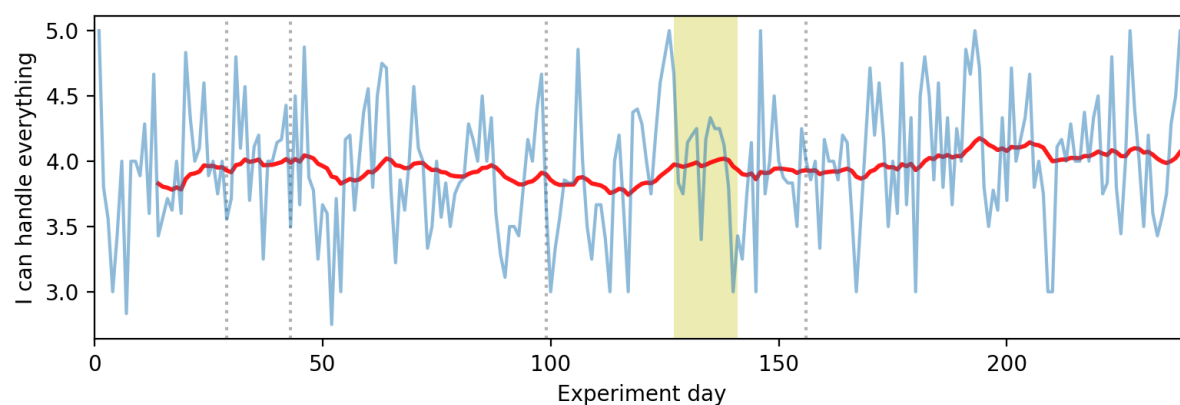

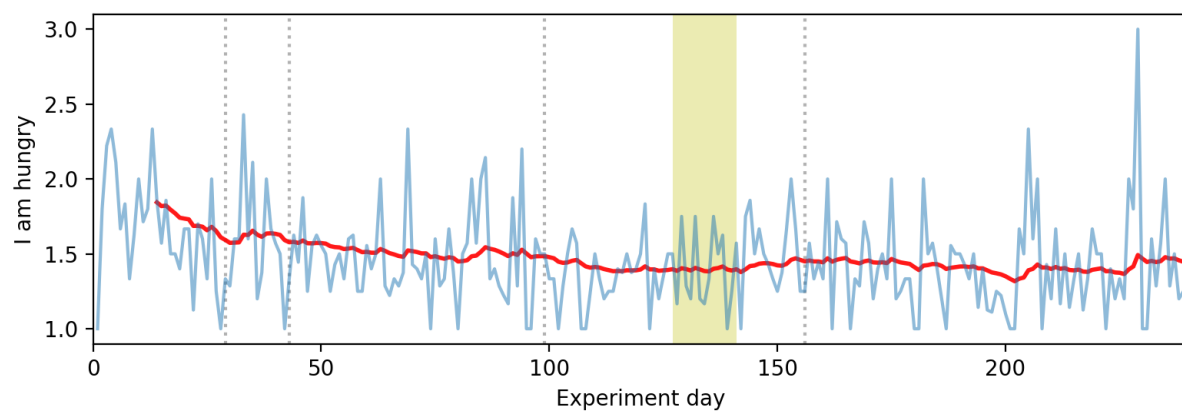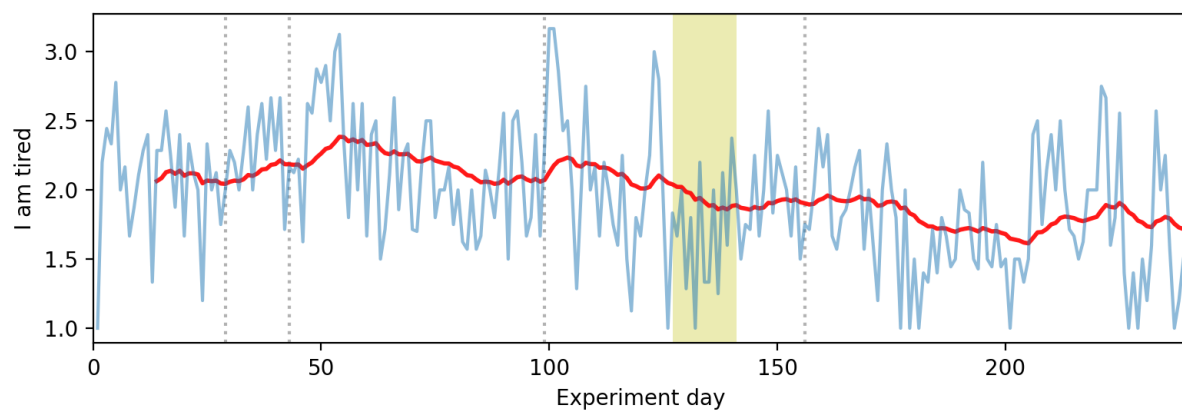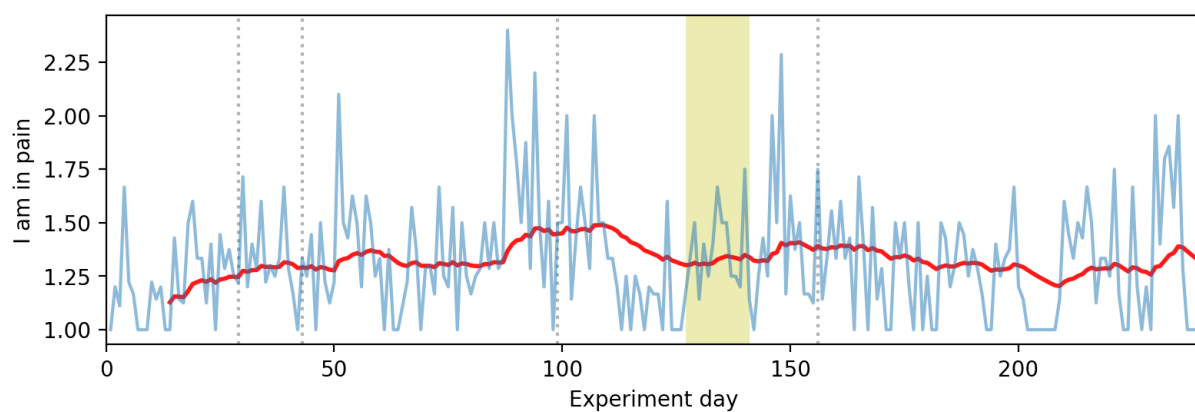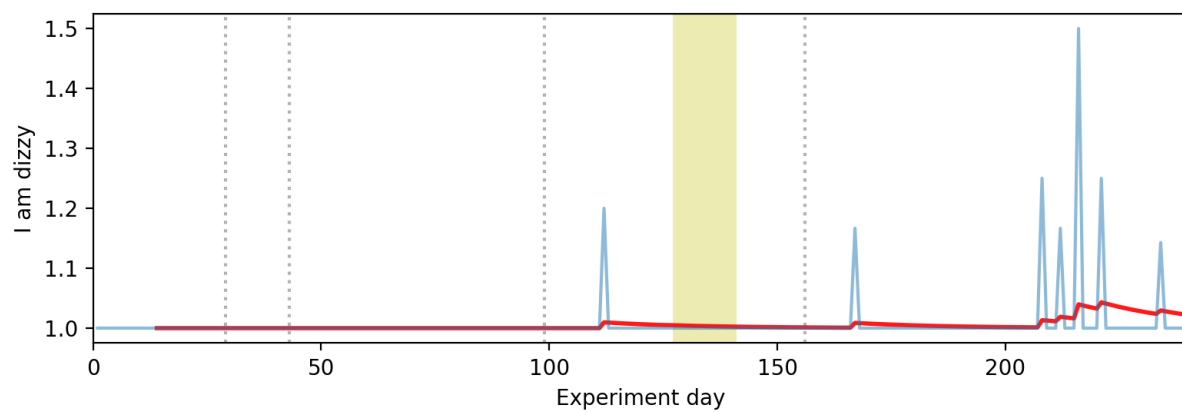

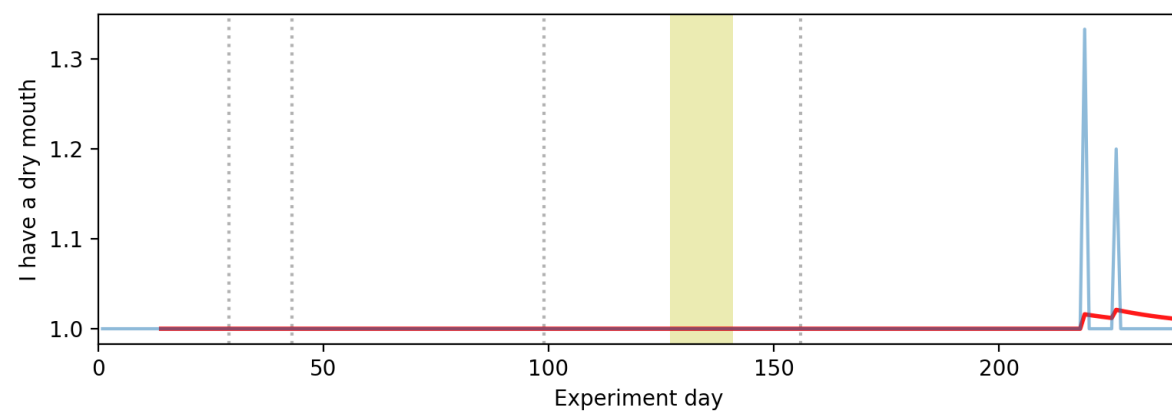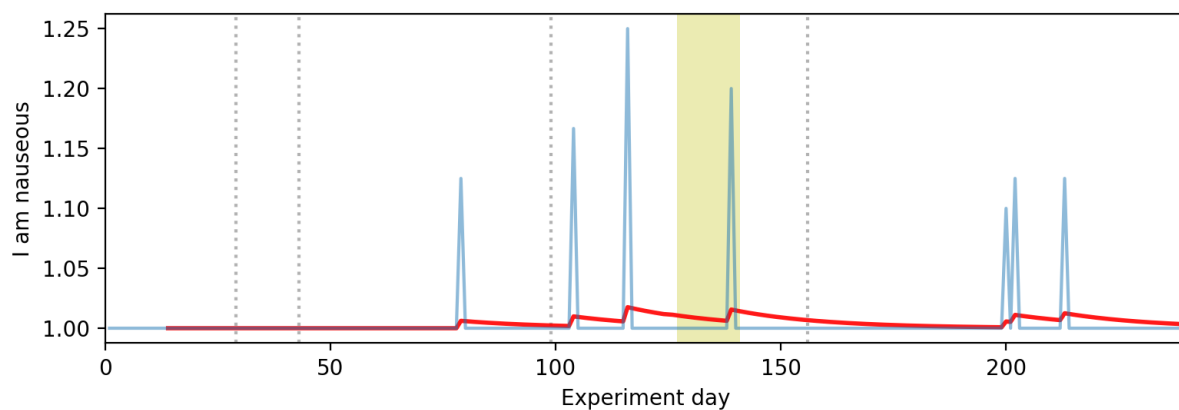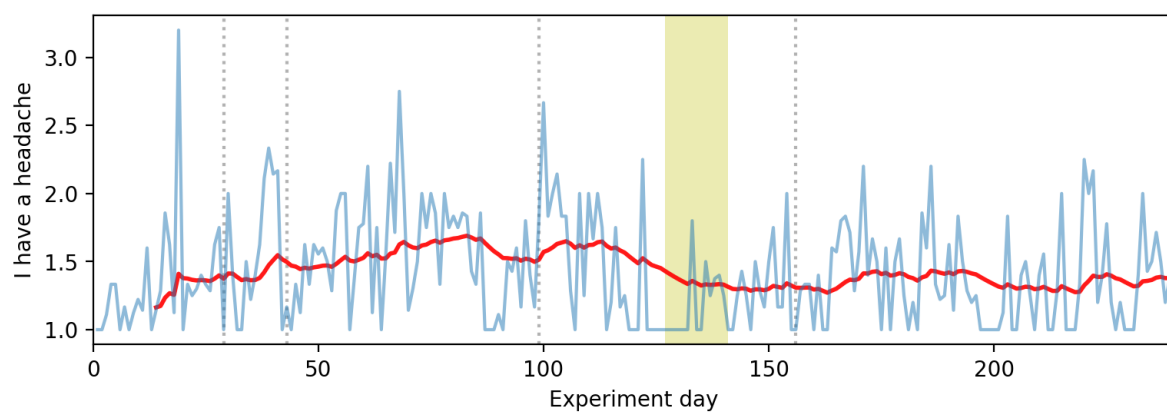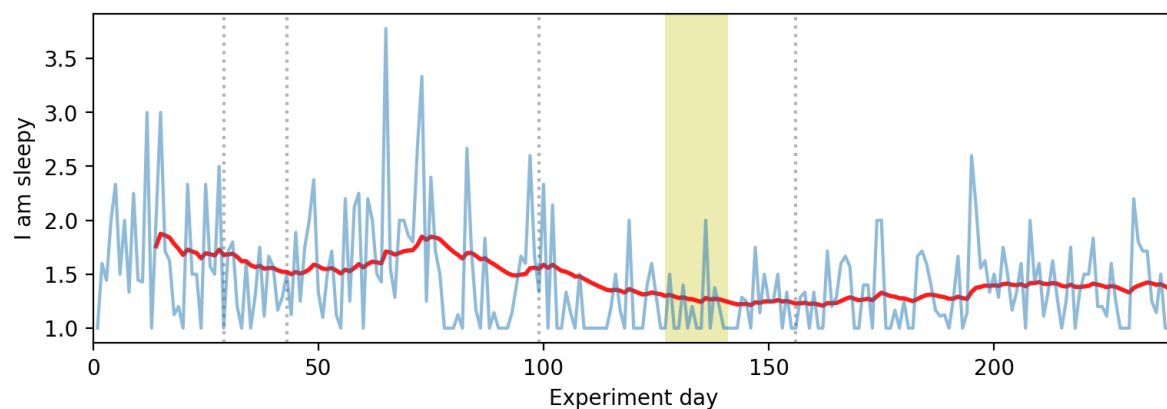

Supplement: Supplementary file 2 [file S1_fig.pdf]
