# Supplementary material for: Phase transition modelling of relapse in major depressive disorder: Developing and reflecting on an interdisciplinary conceptual translation
Source: arXiv:2302.13895 ancillary file (2023-02-27)
Supplement: Supplementary file 3 [file S1_text.pdf]

## S1 Text. Interview guide

The interviews were divided into four main sections (excluding the closing statement), the order of which was partly based on the interviewee's responses. The interview guide is written in Dutch.

---

### Introductie

Als korte introductie zou ik u eerst graag wat willen vragen over uw onderzoek in het algemeen.

- Als u in een paar zinnen moest beschrijven waar uw onderzoek over gaat aan een wetenschappelijk opgeleide collega die geen expertise heeft in de psychologie/medische wetenschap, wat zou u dan zeggen?

### Interdisciplinaire methodiek

Ik heb begrepen dat u werkt vanuit het perspectief van complexe systeemtheorie, klopt dat? Ik ben geïnteresseerd in de methodiek die u toepast om uw onderzoeksvragen te beantwoorden. Denk bijvoorbeeld eens terug aan een onderzoekslijn of -project waar u de afgelopen jaren aan gewerkt heeft.

- Welke technieken en methoden heeft u in dit onderzoek ingezet om uw onderzoeksvragen te beantwoorden?
- Welke theoretische uitgangspunten lagen ten grondslag aan deze methoden?
- In hoeverre onderscheidt de door u gehanteerde aanpak zich van de manier van onderzoek doen die het meest gangbaar is in de psychologie/medische wetenschap?
  - Wat zijn de belangrijkste verschillen tussen de door u gebruikte methodiek en deze gangbare methodiek?
  - Hoe bent u erbij gekomen om deze methode toe te passen, in plaats van de gangbare methodiek?
- Maakte u in uw onderzoek wel eens gebruik van technieken of ideeën die afkomstig zijn uit een ander vakgebied dan de psychologie/medische wetenschap?
  - Welke technieken of ideeën zijn dit?
  - Op wat voor manier integreert u deze technieken of ideeën in de methodiek van uw vakgebied?
  - In hoeverre heeft u daarbij moeilijkheden ervaren als het gaat om het vertalen van deze technieken of ideeën naar uw eigen onderzoek?
- Heeft u voor uw onderzoek ook wel eens samengewerkt met wetenschappers buiten de psychologie/medische wetenschap?

*Zo ja:*

- Welke achtergrond had(den) diegene(n)?
- Als u terugdenkt aan uw meest recente samenwerking, hoe waren de rollen toen verdeeld? Hoe zag de samenwerking er concreet uit?
- Is er wel eens sprake geweest van communicatieproblemen of zelfs misverstanden tussen de vakgebieden in de samenwerking, en zo ja, hoe zag dat eruit?
- In hoeverre heeft die samenwerking resultaten opgeleverd die niet behaald hadden kunnen worden door puur binnen de psychologie/medische wetenschap te blijven?

*Zo nee:*

- Wat zijn de redenen dat zo'n samenwerking niet is voorgekomen?

## Het concept complexiteit

*Integreren in voorgaande wanneer kandidaat complexiteit of gerelateerd begrip noemt.*

Ik hoorde u net het woord complexity/complexiteit/etc. gebruiken. 'Complexity science' is natuurlijk een brede term, die vaak heel verschillend wordt opgevat.

- Wat verstaat u precies onder het begrip 'complexity'?
- Hoe groot is de rol van het begrip complexiteit in uw eigen onderzoek?

*Indien niet natuurlijk aan bod gekomen:*

Het valt me op dat u het woord complexiteit niet gebruikt.

- Hoe komt dat?
- (vervolg als hierboven)

## Relevantie en praktijk

Tot slot wil ik het graag hebben over de relatie van uw onderzoek met de klinische praktijk. Sommige vormen van wetenschap zijn heel toepassingsgericht en staan in direct verband met de praktijk, terwijl ander onderzoek juist heel fundamenteel is en nog ver weg is van een concrete toepassing.

- Waar in dit spectrum zou u uw eigen onderzoek plaatsen?

Stelt u zich eens een ideaal toekomstbeeld voor van uw onderzoeksveld over een paar decennia. Uw onderzoek heeft grote vooruitgang mogelijk gemaakt en wordt nu op dagelijkse basis toegepast in de klinische praktijk.

- Voor welk praktisch doel zou uw onderzoek in dit geval worden ingezet?
- Welke technieken worden er op dit moment gehanteerd in de klinische praktijk voor dit doeleinde, als die er zijn?
- Op welke manier zou het resultaat van uw onderzoek deze huidige technieken aanvullen of vervangen?
- *(indien van toepassing)* Welke rol zou de eerder genoemde interdisciplinaire methodiek hebben gespeeld in deze bijdrage?

## Afsluiting

Dan zijn we nu wat mij betreft bij het einde van het interview aangekomen.

- Is er iets wat u nog zou willen toevoegen wat nog niet ter sprake is gekomen?
