# Supplementary material for: Phase transition modelling of relapse in major depressive disorder: Developing and reflecting on an interdisciplinary conceptual translation
Source: arXiv:2302.13895 ancillary file (2023-02-27)
Supplement: Supplementary file 4 [file S2_table.pdf]

**S2 Table. Codebook**

| Code name                                      | Comment                                                                                                        | No. |
|------------------------------------------------|----------------------------------------------------------------------------------------------------------------|-----|
| Descriptive information                        |                                                                                                                |     |
| Research topic                                 | Describes the topic of their research.                                                                         | 7   |
| Methods                                        | Describes a method used in their research.                                                                     | 22  |
| Collaborations                                 | Describes an interdisciplinary collaboration or origin of concepts/methods.                                    | 26  |
| Elements of complexity                         |                                                                                                                |     |
| Non-linearity                                  | Effects of inputs on outcomes are not proportional.                                                            | 10  |
| Stability domains                              | Existence of multiple stable states, which can change as the context evolved.                                  | 5   |
| Tipping points                                 | Occurrence of a sudden shift in behaviour past a certain threshold.                                            | 7   |
| Change over time                               | Intrinsic development and change over time.                                                                    | 11  |
| Unpredictability                               | Forecasting impossibility and inability to collect all information.                                            | 5   |
| Unknowns                                       | Unknown factors that can influence the system, leading to indirect effects.                                    | 2   |
| Multiple scales and levels                     | Interactions in the system occur across multiple scales and levels, study required from multiple perspectives. | 2   |
| Path dependency                                | The state of the system depends on its history or path to its current state.                                   | 1   |
| Strong interactions                            | Components within a system strongly interact.                                                                  | 11  |
| Similarities with other systems                | Complex systems can show similarities with completely different systems.                                       | 8   |
| Individuality                                  | Focus on the individual and personalisation.                                                                   | 8   |
| Multicausality                                 | Phenomena cannot be explained by singular causal relations.                                                    | 11  |
| Emergence                                      | Interactions between components in the system can lead to emergence of new higher level behaviour.             | 1   |
| Quantitative versus qualitative implementation | Highlighting a contrast between quantitative and qualitative implementation of complexity.                     | 16  |
| Integration of complexity in research          |                                                                                                                |     |
| General role of complexity in research         | Describes the general role of the notion of complexity in their research.                                      | 13  |
| Research question                              | The complexity perspective is reflected in the research questions that are posed.                              | 14  |
| Concepts and theory                            | The complexity perspective is reflected in the concepts and theory behind the research.                        | 14  |
| Study design                                   | The complexity perspective is reflected in the design of the study.                                            | 11  |
| Methods                                        | The complexity perspective is reflected in the methods used to collect data.                                   | 23  |
| Analysis techniques                            | The complexity perspective is reflected in the techniques used for data analysis.                              | 5   |
| Motivations for complexity perspective         |                                                                                                                |     |

| Code name                                  | Comment                                                                                                       | No. |
|--------------------------------------------|---------------------------------------------------------------------------------------------------------------|-----|
| Shortcomings of other methods              | Mentioning shortcomings of and differences to non-complexity oriented science.                                | 32  |
| Better fits practice                       | The complexity perspective better suits the daily reality or practice of the object of study.                 | 20  |
| Yields new insights                        | The complexity perspective can yield different insights compared to other methods.                            | 9   |
| Developing applications                    | The complexity perspective can help develop practical applications.                                           | 4   |
| Monetary gains                             | The complexity perspective can help obtain monetary gains.                                                    | 3   |
| Personally interesting                     | Studying complex subjects is interesting and exciting.                                                        | 4   |
| Increased interest                         | Mentions growing traction of or increasing general interest in complexity science.                            | 8   |
| Challenges to complexity perspective       |                                                                                                               |     |
| Uncertainty in effectiveness               | The effectiveness of complexity methods in research is often still unknown and can disappoint.                | 16  |
| Differences in definition                  | The notion of complexity can be interpreted differently by different actors.                                  | 16  |
| Acceptance by other areas of science       | The complexity perspective is not always easily accepted by other areas of science.                           | 21  |
| Misunderstanding by other areas of science | The complexity perspective can be misunderstood or misinterpreted by other areas of science.                  | 9   |
| Unjustified application                    | The complexity perspective can sometimes be applied too easily or loosely without proper justification.       | 4   |
| No access to required data                 | Research from a complexity perspective requires a specific type of data that may not be available everywhere. | 5   |
| Requires more effort                       | Working from the complexity perspective requires more effort.                                                 | 5   |
| Facilitators                               | Approaches or circumstances that help overcome or alleviate challenges in complexity science.                 | 19  |
| Motivations for interdisciplinarity        |                                                                                                               |     |
| Yields new insights                        | Interdisciplinary work can yield insights that would not have been discovered otherwise.                      | 11  |
| Necessity                                  | It is necessary to work interdisciplinarily in this field.                                                    | 3   |
| Personal inspiration                       | Working with other disciplines is personally inspiring.                                                       | 2   |
| Access to extra expertise                  | Interdisciplinary work give access to extra expertise that is not available otherwise.                        | 9   |
| Better fits practice                       | An interdisciplinary approach better fits the daily practice related to the object of study.                  | 4   |
| Challenges to interdisciplinarity          |                                                                                                               |     |
| Differences in approach                    | Members of an interdisciplinary collaboration can have different approaches or paradigms.                     | 24  |

| Code name                                  | Comment                                                                                                     | No. |
|--------------------------------------------|-------------------------------------------------------------------------------------------------------------|-----|
| Translation                                | Concepts or methods can be difficult to translate between disciplines.                                      | 9   |
| Understanding                              | It can be difficult to understand input from other disciplines.                                             | 12  |
| Miscommunication                           | Interdisciplinary work can lead to miscommunication or language barriers between participants.              | 20  |
| Slower progress                            | Interdisciplinary collaboration can delay research and lead to slower progress.                             | 7   |
| Facilitators                               | Approaches or circumstances that help overcome or alleviate challenges in interdisciplinary collaborations. | 20  |
| Practical relevance                        |                                                                                                             |     |
| Application in practice                    | Mentions a possible practical application of the outcomes of their research.                                | 34  |
| Added value of complexity                  | Mentions an added value of the complexity perspective in practice.                                          | 12  |
| Added value of interdisciplinarity         | Mentions an added value of interdisciplinary work in practice.                                              | 4   |
| Challenges to practical implementation     | Mentions challenges in transferring their research to clinical practice.                                    | 5   |
| Requirements for successful implementation | Mentions requirements for successful implementation of their research outcomes in practice.                 | 12  |
