# Supplementary material for: Phase transition modelling of relapse in major depressive disorder: Developing and reflecting on an interdisciplinary conceptual translation
Source: arXiv:2302.13895 ancillary file (2023-02-27)
Supplement: Supplementary file 5 [file S3_text.pdf]

## S3 Text. Full interview transcripts

**MG** = Marieke Glazenburg

**PX** = Participant X

[...] = inaudible on recording

*The language of the interviews is Dutch.*

### **Participant 1**

**MG:** Yes, dus nu staat hij aan. Nog heel kort over de verwerking en zo van de data, ik ga het interview dus transcriberen, wat ik net zei, en die transcripten en opnames ga ik bewaren, die zijn alleen toegankelijk voor mijzelf en voor de mensen die mij supervisen. Nou, voor de verwerking kan ik alles wat u zegt, of wat jij zegt, anonimiseren en zorgen dat het op zo'n manier in het eindproduct terechtkomt dat het niet herleid kan worden tot jou, maar als je dat goed vindt zou ik ook wel gebruik willen maken van de mogelijkheid om wel jouw naam en achtergrond te noemen als dat relevant is voor het stuk wat ik schrijf. Zou dat oké zijn, of heb je liever dat het anoniem blijft?

**P1:** Ja, dat ligt er een beetje aan wat er in staat.

**MG:** Ja. Ik ben van plan om aan het eind een soort interpretatie, samenvatting te schrijven, en die sowieso nog door te sturen. Eventueel kun je dan afhankelijk daarvan bekijken of dat informatie is die je, ja, die je anoniem wil hebben of niet.

**P1:** Ja. Oké, laat ik me, dat is helemaal prima.

**MG:** Goed, dan zal ik daar voor nu nog niet vanuit gaan. Oké. Ja, dan kunnen we beginnen denk ik. Als korte introductie graag, zou ik eerst even wat willen vragen over uw onderzoek in het algemeen. Als je nou in een paar zinnen zou moeten beschrijven waar je onderzoek over gaat aan een collega die wel wetenschappelijk is opgeleid maar die geen achtergrond heeft in de psychologie, wat zou je dan tegen zo'n iemand zeggen?

**P1:** Nou, dat ik probeer te begrijpen hoe het kan dat de één een veelvoorkomende psychische aandoening ontwikkelt terwijl de ander dat eigenlijk niet ontwikkelt, en ik probeer ook te begrijpen waarom het bij de één eigenlijk niet meer zo vanzelf weggaat en bij de ander wel, en daarbij is denk een centrale uit, het centrale uitgangspunt is dat bij het ontwikkelen van psychische aandoeningen dat er, nou, geen enkelvoudige causale factoren zijn, dus dat er heel veel factoren zijn die een rol spelen, biologische factoren, psychologische factoren, omgevingsfactoren, soms zelfs macrofactoren, bijvoorbeeld beleid in een land kan een rol spelen, en die factoren die werken allemaal op elkaar in, en die factoren worden ook nog eens beïnvloed door het hebben van psychische problemen of psychische symptomen, bijvoorbeeld als je heel somber bent dan kan dat van invloed zijn op je cortisolniveau, dus het stresshormoon, en dat kan weer van invloed zijn op de instandhouding van je

depressieve klachten, terwijl cortisol mogelijk ook een rol speelt bij de, bij het ontstaan van die depressieve symptomen. Dus waarmee ik wil zeggen, uitgangspunt is dat er eigenlijk heel veel verschillende factoren zijn en de manier waarop die factoren op elkaar inwerken die van invloed zijn op het ontstaan en de instandhouden van psychische problematiek, en daarbij, wat we proberen te doen, en daarbij is één van de benaderingen heel zinvol, is we proberen eigenlijk het systeem als geheel te gaan onderzoeken en daarbij ook begrijpelijk te maken hoe die verschillende factoren over tijd op elkaar inwerken, en ons belangrijkste doel, of mijn belangrijkste doel is daarbij om te kijken of je, ja, nieuwe aangrijpingspunten weet te vinden voor interventies, waardoor we een grotere kans hebben om de aandoening te voorkomen ofwel te zorgen dat die minder lang bestaat.

**MG:** Ja. Oké. Ja, en als ik het goed begrijp dan werk je vanuit het perspectief van complexiteitstheorie, klopt dat?

**P1:** Ja, ik heb, jij bent natuurkundige, en ik ben klinisch psycholoog en ook clinicus, dus ik werk vanuit een heel ander perspectief namelijk dat er heel veel mensen zijn die heel intens psychisch lijden, en, dus ik werk, dus dat is, en ik wil begrijpelijk maken waarom dat zo is en wat je daaraan kan doen. En ik denk dat complexe systemen of complexe systeemtheorie mogelijk ons dat, daar chocola van kunnen maken. Maar mijn uitgangspunt is, dat zijn de mensen die ofwel een hoog risico hebben om ernstig psychisch te lijden of die daar al aan lijden, en daar wil ik wat mee doen en daarbij denk ik dat complex systeemdenken zou, ik zie dat als een verrijking eigenlijk van een soort empirische cyclus om begrijpelijk te maken hoe al die verschillende factoren op elkaar inwerken, en, ja, mogelijk dat ons dat nieuwe inzichten geeft hoe je dat het beste kan aangrijpen.

**MG:** Ja.

**P1:** Dus voor mij is het niets meer dan een verrijking van een empirische cyclus om te komen waar ik wil komen, namelijk het vinden van effectievere preventieve interventies en curatieve interventies.

**MG:** Ja. Ja, want...

**P1:** En dat is natuurlijk een hypothese, dat dit een manier zou kunnen zijn die dat zou kunnen opleveren.

**MG:** Ja. Nou ja, daar wil ik straks ook nog wel even op terugkomen. Maar misschien eerst, want het, complexe systeemtheorie wat versta je daar precies onder?

**P1:** Ja, dat is een... Wat versta ik daar precies onder... Nou ja, ik denk dat het ook een verzamelwoord is voor heel veel verschillende fenomenen die in de natuur voorkomen en mogelijk dus ook bij de mens, en dat zijn er heel veel, bijvoorbeeld dat er zoiets als, iets is wat bijvoorbeeld kritische transities, dat het zo kan zijn dat je je bijvoorbeeld heel lang heel goed voelt, maar dan gebeurt er eigenlijk iets kleins en bam boem, het gaat helemaal mis met je en je komt in een full-blown depressie bijvoorbeeld, hè, dat is een voorbeeld ervan. Maar er zijn natuurlijk ook heel veel andere voorbeeld, hè, bijvoorbeeld dat bepaalde processen zich heel langzaam en gradueel over tijd ontwikkelen, terwijl andere processen eigenlijk exponentieel zich gedragen, bijvoorbeeld ik noem even een voorbeeld van de

invloed van trauma, dat je iets heel traumatisch meemaakt, kan heel lang helemaal geen impact hebben op jouw psychische welzijn, terwijl het dan op een gegeven moment, nadat het er eigenlijk al twintig, dertig jaar is, toch je hele welzijn, zeg maar kan weghalen, zoals bijvoorbeeld bij een PTSS, een posttraumatische stressstoornis. Nou, dit zijn maar een aantal voorbeelden.

**MG:** Ja. Ja, merk je ook wel eens dat er verschil is in de manier waarop jij complexiteit en complexe systeemtheorie interpreteert en hoe onderzoekers misschien uit andere velden dat doen?

**P1:** Nou ja, ik ben geen expert op het gebied van complexe systemen, ik ben het, een expert op het gebied van veelvoorkomende psychische aandoeningen, en ik denk dat daar veel fenomenen, misschien moet ik het zo, het is mogelijk dat daar fenomenen plaatsvinden zoals ook in andere velden, zoals bijvoorbeeld in de economie, of in de ecologie, die, of misschien wel in, weet ik veel, in de verspreiding van ik noem maar wat, coronavirus, die, nou ja, die zeg maar een soort, nou ja die, en, waarvan dezelfde fenomenen voor, mogelijk voor een deel ook voorkomen wanneer het gaat over het menselijk welzijn en psychisch lijden en aandoeningen. Maar een deel daarvan is nog natuurlijk nog helemaal niet zeker, dat zijn we, dat is nou net wat we aan het onderzoeken zijn. En de interpretatie daarvan, ik denk zeker dat die heel verschillend kan zijn, maar ja, dat is ook een deel van het onderzoek wat je met elkaar doet, of ze op eenzelfde manier, of die systeem, of, alsof die, of die fenomenen ik noem maar even bijvoorbeeld critical transitions, of die op eenzelfde manier, of die überhaupt plaatsvinden, om te verklaren waarom de één een psychische aandoening op een bepaald moment krijgt en niet. Nou dat, ik, dat zie ik eigenlijk nog deel, een deel als het onderzoek wat we nu aan het doen zijn. Dus ik zou het nog niet, ik denk dat we nog niet zo ver zijn dat we kunnen zeggen dat we nou een dispuut hebben met andere velden waarbij het totaal anders ligt, zo ver zijn wij nog niet.

**MG:** Oké. Ja. Ja want...

**P1:** Ja. Daarvoor zijn wij eigenlijk nog veel meer in een soort, we zijn een soort, we zijn bezig om allerlei complexe systemen, om te kijken, kan het zo zijn dat die systemen ook van toepassing zijn op het gebied van, die, van psychische klachten en aandoeningen, en zou je dat systeem, als je dat nou ergens in het systeem beïnvloedt, bijvoorbeeld in een netwerk van allerlei symptomen, en je identificeert bijvoorbeeld een aantal centrale symptomen in zo'n netwerk, hè met een netwerkanalyse, zou het dan verschil uitmaken als je je daar al je behandelingen op richt, in plaats van op het systeem als geheel dus op alle symptomen. Nou, dit zijn de dingen die zijn wij nou nu net met zijn allen nog aan het uitzoeken. Dus ik denk dat het nog te vroeg is om te kunnen zeggen van hé, daar hebben wij een hele verschillende, ja, daar hebben we misschien een hele verschillende invullingen. Wat me wel opvalt, dat er heel veel, bijvoorbeeld je hebt een groep bij ons, zij, onder leiding van Denny Borsboom, die houdt zich bezig met de netwerkanalyse op het gebied van psychopathologie, het valt me wel op dat die groep bijvoorbeeld weer een hele andere invulling daarvan heeft, dan bijvoorbeeld netwerkanalyses die worden gedaan als onderdeel van agent based modelling bijvoorbeeld, bij de groep die, onder Peter Sloot bijvoorbeeld. En dat zie zelfs nog de grootste moeite hebben om bij elkaar te komen, zullen we maar zeggen. Ik bedoel niet bij

elkaar te komen, maar om, hele verschillende opvattingen hebben over hoe je dat dan zou moeten doen.

**MG:** En waar zit dat dan in?

**P1:** Heb ik werkelijk geen idee van, ik kijk er al jaren met grote verbazing naar.

**MG:** Oké.

**P1:** Nou, dat zit erin dat ze, zeg maar, opgeleid zijn met hele verschillende paradigma's.

**MG:** Ja.

**P1:** Daar zit het hem in, denk ik.

**MG:** Maar dat heb jijzelf nog niet zo direct kunnen ervaren?

**P1:** Jawel, dat ervaar ik wel...

**MG:** Oké.

**P1:** ...maar, je weet pas waar dat in zit als je het hebt opgelost. En het is nog niet opgelost.

**MG:** Ja. Want op wat voor manier ervaar je dat soort verschillen dan nu al wel?

**P1:** Nou, bijvoorbeeld, ik breng die groepen bij elkaar, want ik ben ook directeur van, samen met Reinout Wiers, van het centrum voor Urban Mental Health, daar zitten drie faculteiten in, waaronder de science faculteit, hè daar valt natuurkunde onder, en daar zit ook het IAS in hè, dat is het complexiteitsinstituut van de universiteit van Amsterdam, en je merkt gewoon, dus ik breng die mensen bij elkaar, om te bespreken, hé welke methode gebruik jij en welke gebruik jij en waarom kan dat nou niet bij elkaar komen. En wat zijn daar de grote verschillen, en je ziet dat daar hele grote paradigma, bijvoorbeeld ze gebruiken verschillende modellerprogramma's, daar begint het bijvoorbeeld al mee, ze gaan uit van andere uitgangspunten, je zou, ja. Dus. Waardoor het heel moeilijk voor hen is om te kijken van, doe jij nou hetzelfde wat ik doe.

**MG:** Ja.

**P1:** Dat is een hele interessante, dus ik ben heel veel bezig met dit soort, vanuit mijn rol in de directie ook, in het vertalen van die verschillende paradigma's en [...] naar elkaar toe en uit te zoeken van hé, hoe zit dat nou, want netwerktheorie en netwerkmodellen is toch ook een onderdeel van een complex systeem, en hoe kan het dan dat er, hè, dat dat niet automatisch bij elkaar komt. Dat komt omdat dat dan weer met andere programma's gedaan wordt, maar daaronder ligt ook weer net een ander paradigma.

**MG:** Ja.

**P1:** Lastig is dat. Nou, lastig, nee, dat is niet lastig, dat is gewoon, dat is uitdagend aan interdisciplinair werken. Dus in die zin, als jij vraagt van hé, zie je daar verschillen in, ik zie inderdaad wel verschillen. En die verschillen die zijn heel erg goed dat ze er zijn, maar dat is dan wel heel erg belangrijk dat die verschillende groepen allemaal met elkaar blijven

communiceren, maar dat houdt ook een beetje op voor die groepen, snap je, dat vertraagt ook een beetje, want die willen door.

**MG:** Ja. Ja.

**P1:** Maar, ondertussen, wij hebben ook als taak om die groepen juist bij elkaar te zetten, dus, en dat gebeurt nu ook wel.

**MG:** En vanuit jouw eigen ervaring, werk je veel samen met wetenschappers buiten de psychologie?

**P1:** Ja, en dat is eigenlijk wel de kern van waar ik mee bezig ben. Dus ik leid het interdisciplinair centrum voor Urban Mental Health, moet je maar even kijken ook op, we hebben ook een website van de Universiteit van Amsterdam, en dat leid ik samen met Reinout Wiers, en daar zitten drie faculteiten in, dus daar zit de science faculteit, daar zit bijvoorbeeld natuurkunde, wiskunde, complex systems afdeling van Peter Sloot zit daarin, maar daar zit ook bijvoorbeeld psychologie, sociologie communicatiewetenschappen, dus faculteit gedrags- en maatschappijwetenschappen zit erin, en daar zit de faculteit geneeskunde in, bijvoorbeeld sociale geneeskunde, psychiatrie, dus dat is, en daar zit het Institute of Advanced Study in, en dat is een studie, een centrum wat zich specialiseert op complex systems, geleid door Peter Sloot. Nou, en dat, wij doen eigenlijk niks anders dan elke week al die verschillende disciplines bij elkaar brengen en hen met elkaar te laten communiceren. En onze backbone, onze ruggengraat, dat, waarmee we dus begrijpelijk willen maken waarom de ene floreert in de stad en de ander vastloopt en angststoornis of depressie of verslaving krijgt, en daarbij gebruiken we als ruggengraat om dit begrijpelijk te maken complex systems. Dus dat is wat we in dat centrum doen. Dus ik heb eigenlijk twee dingen, ik heb mijn eigen onderzoekslijn, en daarnaast leid ik dat, samen met Reinout Wiers, dat complexiteitscentrum voor Urban Mental Health en we, ik doe dus niks anders dan de hele tijd al die, met al die disciplines bij elkaar komen.

**MG:** Ja.

**P1:** En een model maken om dat te gaan onderzoeken.

**MG:** Ja. En, op wat voor manier bij zo'n hele interdisciplinaire samenwerking, dat er echt mensen uit volledig verschillende velden bij elkaar komen, hoe zijn de rollen dan verdeeld op zo'n moment, hoe ziet dat er concreet uit?

**P1:** En wat bedoel je, ja, nou ja, goed, wij hebben een centrum dat wordt geleid door directie, dat is iemand van de faculteit geneeskunde, dat ben ik, en iemand van faculteit gedrags- en maatschappijwetenschappen, dat is Reinout Wiers, en daarnaast hebben wij, een zeg maar financieel houderschap, dat ligt bij de science faculty, en dan hebben we nog een bestuur, dat is ook volledig multidisciplinair, dus daarmee bepalen we de strategische lijnen en onderwerpen, en verder hebben wij, even kijken iets van tien PhD, interdisciplinaire PhD-projecten gefinancierd, die worden allemaal, die, alle PhDs worden begeleid door minimaal twee faculteiten, dus supervisors van twee faculteiten, vaak nog drie, en die PhD-projecten, met elkaar zijn wij bezig om eigenlijk een nieuw framework en ook een theoretisch model te maken op grond waarvan we begrijpelijk maken waarom de ene floreert en de ander

vastloopt in een urbane omgeving, met als doel om nieuwe aangrijpingspunten voor interventies te vinden, zowel op individu als op beleidsniveau, en dat doen we dus met die tien interdisciplinaire PhD-projecten, maar daar hebben wij bijvoorbeeld ook wekelijkse meetings mee, en ook die PhD-studenten zijn ook allemaal van verschillende disciplines. Dus we hebben wekelijkse meetings, en we hebben maandelijkse PI-meetings, dat zijn dan de PI uit die drie faculteiten, dus die hebben per definitie allemaal, en het IAS, en we hebben natuurlijk ook nog een lezingencyclus, nou ja goed, en wat wij gebruiken is eigenlijk een framework wat eigenlijk een complex systeem is, dus je zou een framework waarin we het hele systeem definiëren, en waarin wij van micro tot macroniveau kijken naar allerlei factoren die bijdragen en hoe ze interacteren, en dat framework ofwel dat theoretisch model wat in ontwikkeling is, dat is eigenlijk het centrale motto op grond waarvan wij ons onderzoek invullen. En, bijvoorbeeld nu, zij, hebben wij wekelijkse modelleersessies met allerlei complex systems experts, waarin we aan het kijken zijn, hé, wat, welk deel van het theoretisch model gaan wij modelleren om eigenlijk een stuk toetsing te doen van het model.

**MG:** Ja.

**P1:** Nou, en, nou, gaan bijvoorbeeld de discussies van nou, op welke manier gaan we een critical transition modelleren, of willen we dat, willen we een agent based model gaan doen, of, nou ja, dat soort, of gaan we een netwerkbenadering doen, bijvoorbeeld, hè, waarin wij nu aan het bekijken zijn hoe we de invloed van sociale cohesie binnen de stad op en de invloed daarvan op mentale gezondheid, hoe we dat zeg maar kunnen, dus, nou ja, op die manier geven we dat vorm.

**MG:** Ja.

**P1:** En daarnaast zijn dus allerlei PI's aangesteld, dus dat zijn mensen minimaal op postdoc niveau, die voor een deel ook gefinancierd worden vanuit ons centrum, om ook weer te werken aan dat overall model wat begrijpelijk moet maken waarom de één floreert en de ander vastloopt. En een deel van de PI's zijn weer bijvoorbeeld complex systems modelleers.

**MG:** En wat voor achtergrond hebben die dan bijvoorbeeld?

**P1:** Ja, die zijn dan, in de, experts op het gebied van complex systems.

**MG:** Oké. Dus niet vanuit een specifieke richting?

**P1:** Nee. Ja, wat is een specifieke richting, van complex systems?

**MG:** Nou ja, dan bijvoorbeeld, psychologische complex systems, ecologische...

**P1:** Nee, nee. Nee, nee, dat niet, nee. Dus, die PI's, nou, in de meeste gevallen zijn zij, dat is een goeie vraag, zijn zij niet zozeer vanuit de inhoud gedreven, bijvoorbeeld een psychologisch, die hebben we ook, die zitten bij psychological methods, dus daar zit een aantal mensen die heel veel ervaring hebben met netwerkanalyses, gericht op psychologische, psychopathologie zoals wij dat noemen, maar wij hebben ook complex systems PI's die echt vanuit de complex systems komen zonder dat daar echt een onderwerp aan vast zit. En dat is ook wel bewust, want dan willen we kijken of ze bijvoorbeeld iets wat ze

ontwikkeld hebben op het gebied van inflammatie willen we kijken wat nou als we die modellen nou eens gaan toepassen op psychisch lijden.

**MG:** Ja.

**P1:** Hè, is dat te vertalen daar naartoe of niet, en op grond waarvan dan, en wat leert ons dat.

**MG:** Ja.

**P1:** Dus voor een deel wel, en voor een deel niet. Dat is eigenlijk het antwoord. En dat is ook best wel weer ingewikkeld, want voor elke keuze is wat te zeggen hè. Want dat betekent ook dat je als je dat niet hebt, dan moet je die mensen voortdurend meenemen in het onderwerp, want die weten dan heel weinig van het specifieke onderwerp af, maar het heeft wel weer als voordeel dat je misschien dingen kan ontdekken die je anders niet zou ontdekken. Maar het heeft als nadeel dat je soms ook wel weer heel lang bezig bent om mensen ook een beetje mee te nemen in expertise op dit gebied.

**MG:** Ja, want merk je daar wel eens moeilijkheden in, misschien kun je daar wat...

*P1 verlaat de Zoommeeting en komt 45 seconden later weer binnen.*

**P1:** Hai. Sorry.

**MG:** Ja.

**P1:** Hij deed het even niet, ik probeer het even opnieuw weer.

**MG:** Ja.

**P1:** Ja. Lukt het zo?

**MG:** Ja, ik denk het wel.

**P1:** Oké super. Jij had, wilde me net vragen, heb, merk je daar wel eens moeilijkheden mee.

**MG:** Ja, die had je nog meegekregen, ja.

**P1:** Nou, moeilijkheden, het zijn uitdagingen. Die, je moet eigenlijk als je dit op deze manier werkt, ten eerst, je moet niet teveel haast hebben. Want je bent eigenlijk heel veel, je bent heel veel tijd kwijt, één om het vinden van een gemeenschappelijke taal, hè om, je moet elkaars taal praten, dat merk je al aan ons, weet je, ik praat een andere taal dan jij praat, als jij zegt van, ja, wat is dan, hè, jouw primaire focus, nou mijn primaire focus is de inhoud, dus voor mij is complex systems niks anders om, een tool om iets anders op te lossen wat gewoon flauwekul is want het is geen tool, dus ik snap dat het geen tool is, maar zo denk ik terwijl iemand die een expert is op het gebied van, ik zeg maar wat, agent based modelling, die denkt, ja, wat jij mij nu zegt, daar kan ik niks mee, snap je, dus je bent ten eerste ben je de hele tijd bezig om een gemeenschappelijke taal te vinden. En doordat wij hebben gekozen voor het algemene uitgangspunt dat alles op van alles van invloed is en dat het niet zozeer gaat om een, wat op één moment van A tot B leidt, maar dat je eigenlijk moet opgeven dat je dat gaat vinden en dat je, hè, wat dat betreft een totaal andere benadering aanneemt, en dat wij complexe systemen als gemeenschappelijke taal nemen, dus iedereen die aankomt zegt

van, oh, ik heb nu wat gevonden, inflammatie veroorzaakt alle psychische aandoeningen dus we moeten iedereen met antibiotica behandelen. Dat is wel degelijk een interessante gedachte die helaas ook alweer verlaten is inmiddels, maar daar, op die, op dat schip gaan wij niet, nou wij gaan niet, daar gaan wij niet als primaire focus, want dan zeggen we van, nou oké, dat hebben we in de afgelopen honderd jaar gedaan, dat laten wij achter ons, het kan wel degelijk relevant om te zijn om dit te bekijken, als je in staat bent om te identificeren voor wie dit misschien mogelijk wel een causale factor en wie voor wie niet. Maar om, wij, het is heel onwaarschijnlijk dat wij dat dan weer gaan omarmen. Dus, kortom, die gemeenschappelijkheid in paradigma is denk ik wel heel erg belangrijk om dat te omarmen want dan is het ook te doen om met elkaar voortdurend die vertaalslag te maken, maar dat neemt niet weg, het kost je wel een hoop tijd. En het is soms ook heel erg vermoeiend, want heel veel disciplines die hierin werken die denken, hè, wat een onzin, weten ze dan niet dat dit echt state of the art is in dit veld, dus daar hoeven we echt niet naartoe, daar worden dus ook heel veel dingen bedacht waarvan we inmiddels wel weten dat dat echt een gepasseerd station is, dat daar echt voldoende bewijs is dat dat niet zinvol is om op door te gaan. En dat zijn soms vermoeiende paden, en daarvoor is het soms wel nodig om een direct, om goed een leiding te nemen. Je moet aan de ene kant open staan voor totale nieuwe ideeën, of dat je misschien dingen die je al heel lang geleden in de bureaula zijn verschenen, of in de bureaula zijn gekomen omdat men dacht, ja dat heeft geen zin maar, die moet je weer ook de ruimte geven om ook naar boven te komen hè, en tegelijkertijd, ja, moet je ook af en toe, ja, toch ook wel de leiding nemen om te kunnen kijken met elkaar van nou, dit is gewoon geen vruchtbare weg, dit moeten we met zijn allen verlaten, want anders dan zijn we heel veel tijd kwijt aan dood spoor. En tegelijkertijd moet je ook de ruimte nemen, en dat is denk ik wel cruciaal en dat is misschien binnen de natuurkunde veel vanzelfsprekender in ons, dan in ons werk, je moet ook de tijd kunnen nemen om doodloop, om het risico te nemen dat je een doodlopend spoor in gaat.

**MG:** Want heeft u...

**P1:** Je moet, dus ook, ja.

**MG:** ...heb je een voorbeeld misschien van zo'n doodlopend spoor?

**P1:** Nou ja, wij zijn nog niet zo lang bezig dat we al kunnen zeggen, dat is een doodlopend spoor. Maar je kan je wel voorstellen dat je, nou ja, dat die nog wel gaan komen, dat uiteindelijk toch blijkt dat we, weet ik veel, met zijn allen gingen kijken naar, nou, eigenlijk een voorbeeld is misschien wel, in de netwerktheorie en netwerkmodellen van psychopathologie leek het een tijdje zo dat het met name belangrijk is op die centrale symptomen te , hè, dat het daarom ging, want die, als dus een symptoom tussen allerlei symptomen heel centraal was, dan was dat misschien wel een hele karakteristiek voor psychopathologie, voor iemand met, dus daar moest je misschien wel op interveniëren. Nu, inmiddels, lijkt het zo te zijn dat die centraliteit eigenlijk helemaal niet zo karakteristiek is voor psychopathologie, maar misschien gaat het veel meer over de densiteit van zo'n netwerk. Ook dat is niet helemaal zeker, want je vindt ook wel weer dat mensen heel, die heel gezond zijn een heel dense netwerk hebben. Dus je zou je kunnen voorstellen, misschien als we dan met zijn allen op die centrale symptoom of die densiteit gaan zitten, om daarop te



intervenieren, ja misschien is dat eigenlijk wel een zinloze weg, omdat we misschien eerst moet kijken van ja, welk karakteristiek van die architectuur van zo'n netwerk is nou eigenlijk geassocieerd met een slechte prognose, en dat je dan pas moet gaan kijken, van oké, waar moet je dan op intervenieren. Dus je zou je kunnen voorstellen dat we misschien iets voorzichtiger moeten zijn met het, nou, hypothetiseren op waar je moet intervenieren. En dan kan je zeggen van ja, hypothetiseren, wat maakt dat nou uit, dat mag toch wel, maar in mijn wereld, hè omdat ik ook clinicus ben, dan maakt het echt uit, want dan ga je dus in een, bijvoorbeeld in een experimentele, dan ga je mensen een experimentele behandeling aandoen, en ja, als dat eigenlijk een te wilde hypothese is, ja, dan onthoud je mensen wel een andere actieve behandeling. Dus dat weegt wel zwaar, want dat kan soms letterlijk over leven of dood gaan, bijvoorbeeld bij verslaving kan het om leven of dood, maar ook bij depressie kan je je voorstellen ja, het komt nogal eens voor dat iemand zich suïcideert, hè dus, waarmee ik wil zeggen, ja, het weegt best wel zwaar als je dan vervolgens daar ook een behandeling ontwikkelt en dat ook experimenteel gaat onderzoeken, dan moet je best wel beslagen ten ijs komen.

**MG:** Ja.

**P1:** Nou, ik wil niet zeggen dat we dat niet doen, maar ik ben zelf dus een scientist practitioner hè, dus ik ben zowel als clinicus werkzaam en ook wetenschapper, en ik voel mij ook heel regelmatig wel een beetje soort het geweten van de onderzoekers, waarin ik continu weer zeg van ja, maar we moeten eerst kijken of deze factoren überhaupt samenhangen met bijvoorbeeld prognose, want anders is het misschien niet zo heel logisch dat je nou per se daarop moet gaan intervenieren.

**MG:** Ja.

*P1 verlaat de Zoommeeting en komt 10 seconden later weer binnen.*

**P1:** Daar ben ik weer.

**MG:** Ja, hij doet het weer.

**P1:** Hé, sorry. Hoor jij mij zo?

**MG:** Ja.

**P1:** Anders doe ik hem eventjes zo, misschien als ik hem, ik denk dat mijn telef-, mijn oor, ja, je hoort me zo wel hè? Ja.

**MG:** Ja, goed te verstaan.

**P1:** Doen we het zo.

**MG:** Goed. Ja, ja ik was wel verder nog wel benieuwd eigenlijk, want je noemt net al bijvoorbeeld netwerkanalyse als een methode...

**P1:** Ja.

**MG:** ...maar zijn er meer van dat soort methodes die je gebruikt die niet direct typisch zijn voor onderzoek binnen de psychologie?

**P1:** Nou ja, netwerktheorieën, of netwerkanalyses, dat is eigenlijk in de afgelopen jaren heel veel gedaan, het heeft ook best wel veel stof op doen waaien, en heeft ook bijvoorbeeld het idee ge-, zeg maar dat symptomen kunnen, dat het ene symptoom de andere symptoom kan triggeren en dat dat zo een heleboel andere kan triggeren en dat dat vervolgens ook kan leiden tot een echt een, bijvoorbeeld een depressieve stoornis of verslaving of zo, dat idee heeft zeg maar steeds meer plek gekregen, al heeft dat ook weer heel veel vragen opgeroepen, ja maar waarom is het dan zo dat het bij de één heel veel andere symptomen triggert en bij de ander niet, waarom, hoe kan dat dan, hoe verklaar je dat dan, en is dit dan eigenlijk wel verklarend model, want niet iedereen krijgt heel veel verschillende symptomen, hè hoe kan dat dan, waarom stopt het bij de één en de ander niet. Maar er zijn binnen ons veld ook, er is ook wel onderzoek gedaan bijvoorbeeld naar die kritische transities en bijvoorbeeld die early warning signs, signals noem, heten ze volgens mij in jullie veld, waarin gekeken is, hè of je op basis van die transities een, nou, vroeg signaal kan krijgen dat iemand bijvoorbeeld een depressie krijgt of een depressieve terugval, daar ben ik bijvoorbeeld veel mee bezig geweest, nou wat nog meer, bijvoorbeeld er wordt ook nu zachtjes aan een beetje werk gemaakt van bijvoorbeeld agent based models, maar nogmaals, ik ben geen complex systems modelleur hè, dat ben ik niet. Dus ik verleid anderen om daarin de beste te zijn op het veld, op het meest fascinerende veld, naar mijn idee, wat ertoe doet in het leven, namelijk hoe je je voelt. Dus ik voel mij zelf regelmatig als een soort makelaar die dus hele goeie mensen op het gebied van complex systems verleidde om dit terrein als expertises op zich te nemen, omdat dit het meest essentiële is waar het over gaat in het leven. Als je je namelijk niet lekker in je vel zit, als je somber bent of verdrietig of angstig, dan doet niets er meer toe. Met name als het heel, als het je helemaal overneemt, als je daar helemaal geen grip meer op hebt, dan doet helemaal niets er meer toe, dan kan ook niets meer jou meer raken, en daarom heb ik uiteindelijk destijds besloten om psychologie te gaan studeren omdat ik dacht ja, volgens mij is dat wel het centrale wezen van ons zijn.

**MG:** Ja, ja.

**P1:** Ja.

**MG:** Ja en als je dan dat soort methoden, of dat soort resultaten die dan uit die analyses komt, of je die nou zelf doet of niet, ja, is, hoe moeilijk of hoe makkelijk gaat dat om dan vervolgens die resultaten echt weer te interpreteren binnen jouw focus van echt de psychologie?

**P1:** Nou ja, je moet wel echt, kijk ik ben nu al een heel aantal jaren mee bezig, en, je moet eigenlijk wel blijven lezen en inlezen en begrijpen en ook accepteren, want eigenlijk wat, wat denk ik, wat, even mijn vertaling, jij zou misschien als, vanuit jouw natuurkunde-expertise mijn uitlezen, maar vanuit mijn perspectief is het al, je moet eigenlijk een stap over om te zeggen van hé, er zijn bepaalde, je, zeg maar je moet een stap zetten waarin je moet accepteren dat er bepaalde wetmatigheden zijn van bepaalde fenomenen die misschien wel overall plaatsvinden. In de biologie van de mens, in de ecologie, in, misschien het economisch globale systeem, maar ook in hoe jij je voelt. En dat is best een, dat is best een hele grote stap, want meestal voelen wij, hebben wij het idee, en jij misschien ook, dat jij, jij bent je eigen persoon, en het maakt heel erg uit wat jij denkt en doet in hoe jij je voelt, in plaats van

dat jij eigenlijk niks meer bent als een soort natuurlijk fenomeen waarin jouw gevoelsleven je op een bepaalde manier ontwikkelt, net zoals bijvoorbeeld misschien een ecologisch systeem in een vijver. Dat is, snap je? Dat is een, dat is, dat is een, nou ja hoe noem je dat, misschien een paradigma toch wel, daar begint het al mee, je moet accepteren, stel nou dat er een bepaalde wetmatigheid is wat ook verklaart hoe je gevoelsleven je ontwikkelt, of hoe een psychische stoornis zich ontwikkelt of in stand houdt. Dat staat, ja, dat staat zeg maar echt in contrast met bijvoorbeeld, heel veel van de psychologische etiologische en psychiatrische etiologische theorieën, en ook over hoe we bijvoorbeeld psychotherapie doen, want daar ga je dan kijken van hé, hoe ben jij, hè, hoe, wat is jouw levensgeschiedenis, hoe heb je ontwikkeld, wat ben je tegengekomen, hoe ben jij zelf als temperament, wat, en hoe komt dit alles bij elkaar, wat voor een ellende heb je meegemaakt, om begrijpelijk te maken dat jij bent zoals jij bent en dat jij misschien wel psychische problemen of zelfs aandoeningen ontwikkelt, en we gaan dan met jouw unieke geschiedenis kijken hoe we daar wat aan kunnen doen. Snap je, dat is een heel ander verhaal dan te zeggen ja, je bent niks meer als een product van misschien wel een soort, begrijp je...

**MG:** Ja.

**P1:** ...systeem, of misschien wel een, nou. Dus waarom vertel ik dit hele verhaal, je hebt dus ook zelf, je moet een soort paradigmashift maken. En daar moet je toch weer geloven in wetmatigheden. Nou geloof ik wel in wetmatigheden, want in mijn veld hebben we ook wetmatigheden en bepaalde theorieën, bijvoorbeeld, je kent vast wel Pavlov.

**MG:** Ja.

**P1:** Ja. En dat is eigenlijk de basis van klassieke conditionering, hè, dat als je een belletje hoort dat je dan gaat speeksel, en het idee is dat dat, ook operante nou conditionering, dat was Skinner met de duiven en de boxjes, dat weet je misschien ook wel, nou, die basis hè, dat we namelijk leren en verwachtingsleer hebben, dat is ook een hele belangrijke basis voor bepaalde psychologische theorieën waarom mensen bijvoorbeeld psychische aandoeningen krijgen. Dus daar zitten ook wetmatigheden in, maar dat vinden heel veel mensen toch niet zo heel erg aantrekkelijk maar dat hebben we wel. Maar, kortom, om een heel lang verhaal kort te maken, dat betekent dat je je heel lang heel veel moet lezen en ook accepteren dat je een bepaalde uniciteit van mensen moet loslaten, en dat bepaalde, dat er bepaalde wetmatigheden zijn die misschien wel kunnen opgaan voor zwermen vogels, alsook voor hoe jij je voelt. En dat kost ook gewoon tijd, en tegelijkertijd, ik persoonlijk vind dat superopwindend, want dat is de kern, naar mijn idee, van wetenschap maar ook wel, naar mijn gevoel, waarom ik heel graag psycholoog wilde worden, omdat ik het heel erg fascinerend vond dat je iets wil gaan begrijpen wat je niet misschien allemaal exact kan meten en weten. En dat is van misschien wel wat ons bindt, want dat is de natuurkunde naar mijn idee ook. Hè de natuurkunde, dat vind ik heel grappig daaraan, die hebben eigenlijk veel meer al een soort acceptatie dat je nou niet eenmaal niet alles feitelijk kan meten, dus ga je bepaalde aannames doen en dat doe je bijvoorbeeld met formules, right? En die formules, dat geeft wel een soort zekerheid, maar het is voor een deel is het ook schijnzekerheid, want om de zoveel, weet ik veel, om de zoveel, nou ja decennia is te veel, maar om de paar eeuwen, zou je kunnen zeggen, komt men er toch achter dat het toch ergens een foutje in

die formule zat of dat je dat anders moet doen, waardoor er weer hele nieuwe inzichten komen. Dus dat daarin weet je het ook niet helemaal zeker. Nou ja, en die onbekendheid vind ik eigenlijk ook heel erg fascinerend, je weet het nooit helemaal zeker, dus je moet leven met dat je heel veel aannames moet doen. En ik denk dat dat misschien wel iets is wat ons zou kunnen binden. Maar goed, ik denk aan de andere kant om heel eerlijk te zijn dat er heel veel mensen zijn binnen het veld van de psychiatrie en psychologie, overigens ook daarbuiten, heel, er zijn heel veel velden die dit niet aan willen. Want je moet...

**MG:** Waarom...

**P1:** ...enorm investeren en blijven investeren om die brug te kunnen gaan maken. Ja.

**MG:** Ja. Ja, ik zit een beetje naar de tijd te kijken, ook voor jou, ik weet niet... Denk dat we richting [...]...

**P1:** Ik zal even kijken, ik zal even vragen, zal ik ietsje later... Oké. Ja, ik kan wel over, ik heb nog tien minuten.

**MG:** Oké. Ja. Ja, want dan zou ik nog heel eventjes terug willen naar die relatie echt met de klinische praktijk, omdat jij daar natuurlijk ook wel heel erg in geworteld bent.

**P1:** Ja.

**MG:** Want als je nou bijvoorbeeld kijkt naar zo'n methode als netwerkanalyse, of je had het net over bijvoorbeeld early warning signals en zo, wat voor, ja, wat is, wat voor meerwaardes hebben dat soort technieken in de klinische praktijk?

**P1:** Ja, dat weten we nog niet helemaal zeker. Ik ben heel erg empirisch hè, dus ik denk wel, waarom ben ik wetenschapper geworden, omdat ik heel slecht ben in geloof. En dat was ik al heel jong, want ik weet nog heel goed dat ik dan, uit gewoonte ging ik mee naar de kerk, destijds, en ik zat daar, toen was ik een jaar tien, elf, zat ik daar in die kerk, daar ging ik dan mee met mijn ouders, dat was ook de bedoeling, en dan keek ik die pastoor aan en dan dacht ik, wie zegt, jij zegt nu wel dat jij door God gezonden bent, maar dan keek ik om me heen naar die volwassenen en dan dacht ik van, is er dan helemaal niemand die zich afvraagt, wie bewijst nou dat dat daadwerkelijk zo is, want ja, kan net zo goed zijn dat je dat zelf bedenkt, omdat je dat wel zo goed uitkomt. En ik denk dat dit wel een soort centrale, en in die tijd waren natuurlijk al heel veel mensen, het was een tijd waarin die kritisch waren naar vanzelfsprekendheden als het geloof, dus ik wil me daar helemaal niet bijzonder in, maar het is wel kenmerkend voor mij dat ik wel altijd denk, van ja, maar wie bewijst nou dat dat zo is, dat was, later ging ik als clinicus werken, en, ja, die collega's van mij die werden knettergek van mij, want die, dan zei ik van ja maar hoe weet je nou dat dit, wat is nou het bewijs dat dit de beste methode is om aan te bieden voor deze patiënt, en het zou misschien heel goed zou je, er zouden ook andere methodes kunnen zijn, en op grond waarvan kunnen we nou zo goeie, best mogelijke beslissing maken of een best mogelijk advies geven aan een patiënt, dan moeten we toch naar de wetenschap toe. Nou die werden daar knettergek van, die dachten ja sorry, ik heb over een kwartier weer een volgende patiënt, toedelejokie. En ik wil ook gewoon, hè. Toen dacht ik al wel, oké, vrij snel, ik moet gewoon ook onderzoek gaan doen, want ik wil niet alleen de beste, het best mogelijke advies kunnen geven maar ik wil

ook begrijpen waarom dan, en wat zijn dan de werkingsmechanismen, hè, wat werkt dan het beste en als het werkt, waarom werkt het dan. Nou, was al vrij snel duidelijk dat ik, als je dat wil dan moet je natuurlijk ook de wetenschap in. Nou ja, nu kom ik terug op jouw vraag. We weten eigenlijk nog helemaal niet of behandelingen die zich baseren op bijvoorbeeld een symptoomnetwerk, want dat is het meeste gedaan, hè, of dat nou beter is dan wanneer je het niet doet. Ik doe daar overigens nu wel onderzoek naar, dus wij onderzoeken nu bij jongeren, daar maken we bij jongeren die al opgeknapt zijn van een depressie of een angststoornis, die pech hebben gehad, die dat al in een jonge leeftijd hebben meegemaakt, daarbij personaliseren we de interventies gebaseerd op een individueel netwerk van symptomen, die volgen we een paar weken lang met een appje waarin ze regelmatig aangeven hoe ze zich voelen, waar ze last van hebben, bla bla bla. En dan maak, vervolgens creëren we een individueel netwerk, die krijgen zij ook te zien, en dan gaan we kijken hé, wat staat nou het meest centraal, bijvoorbeeld stel nou slapen staat centraal, en het is ook, nou, en we hebben nog wat andere dingen die we vragen, ik ga de details ga ik je niet mee vermoeien, en dan gaan we vervolgens, krijgen zij op basis van dat individueel netwerk een advies om uit een supermarkt van apps om dan bijvoorbeeld als slaap centraal staat in jouw individuele netwerk, krijgt een advies, nou neem in ieder geval ook die slaapmodule mee, want dat wordt een app, en dat wordt ook begeleid door iemand. Hè, en dan hebben we een paar dingen die krijgen iedereen, maar een paar apps uit die supermarkt aan apps, die zijn, die worden echt uitgekozen, gebaseerd op wat bij jou het meest centraal staat. Dat wordt gedaan op basis van netwerkanalyse. En ons doel is met dit onderzoek om te kijken of we daarmee ook een effectievere terugvalpreventie-interventie hebben dan wanneer we het gewoon standaard hetzelfde aan iedereen geven. Nou, in dit geval, is iets ander verhaal, maar daar komt het eigenlijk op neer. Dus daarin onderzoeken we of het daadwerkelijk een klinische, of het gerechtvaardigd is om daar een klinische toepassing van te doen. Want mijn, en dan kom ik weer terug op mijn geloof, ik ben slecht in geloof en daar ben ik best wel trots op ook, ik ben slecht in geloof en ook vroeger dat ik dat het een handicap was, dan was ik een beetje somber van, dan denk ik ben ik nou de enige die twijfelt of het wel klopt dat die door God gezonden is, of ben ik nou de enige die twijfelt of dit nou wel het best bekende is voor deze patiënt die zo ernstig lijdt, en nu ben ik er eigenlijk wel trots op want ik denk, dat zijn de vragen die je moet stellen om, voordat je überhaupt iets aanbiedt. Dus ik vind dat er op dit moment helemaal nog niet op basis van netwerken interventies moeten worden toegepast in onze praktijk, voordat we weten, dat kan alleen nog maar experimenteel, voordat we weten of dat op zijn minst even effectief is als we hebben, maar het liefst effectiever. En daar worden wel meerdere studies al naar gedaan nu, maar wij zijn daar nu als één van de eerste ook aan het personaliseren en aan het kijken of we daarmee op zijn minst even effectief of effectiever zijn. Misschien is het wel veel minder goed. Dat kan hè. Dat weten we dus nog niet.

**MG:** Ja. Ja, mooi. Ja, misschien nog even als afsluiter, stel dat echt over een aantal, nou, decennia, echt dit soort complexe methoden heel effectief blijken te zijn en echt dagelijks worden toegepast in de klinische praktijk, wat voor rol zouden nou die interdisciplinaire samenwerkingen die jij aangaat hebben gespeeld in een bijdrage, ja, in zo'n ideale situatie?

**P1:** Nou ik denk dat het niet kan zonder een interdisciplinaire samenwerking, want bijvoorbeeld klinici of psychiaters of klinisch psychologen, ja die zullen nooit de experts worden op het gebied van bijvoorbeeld simulatie, want dat is nog een ander ding dat ik nog niet heb genoemd, zo kan je je ook voorstellen, als wij gaan simuleren, want dat is wat we nu willen gaan doen, gaan simuleren wat de impact is bijvoorbeeld van een verandering in beleidsmaatregel. Sorry, ik word de hele tijd gebeld dus ik moet ze even wegstippen. Maar als we dat gaan simuleren, dat soort modellen zouden bijvoorbeeld ons inzichten kunnen geven over, waar, op welke velden het misschien, op welke factoren het misschien echt geen zin heeft om te gaan inzetten, terwijl andere factoren misschien wel van belang zijn. Dus het zou zo kunnen zijn dat er bijvoorbeeld helemaal geen ruimte voor verbetering is als je, ik zeg maar wat, op toegang tot zorg verbetert, terwijl er wel ruimte voor verbetering zit als wij de terugkeer tot werk gigantisch gaan faciliteren, ik noem maar wat, dus dat is niet eens op individuniveau. Of als je, ik zeg maar wat, ik ga, even op jongeren gericht, als je bijvoorbeeld, nou, nu is het tijden van corona, we weten dat heel veel, veel meer jongeren dan normaal worstelen met psychische problemen, ook die jongeren die daar eigenlijk helemaal niet kwetsbaar voor waren, wat nou als je in plaats van de toegang tot zorg, tot jeugdzorg, rond GGZ, als je dat zou gaan simuleren wat gebeurt er dan, is, betekent dan dat je... En stel dat je zou vinden dat dat eigenlijk heel weinig added value heeft, terwijl als jij bijvoorbeeld iedereen, ik noem maar even wat, die nu op de middelbare zit en op voortgezet onderwijs, hè dus dan heb ik het over MBO tot en met universitair niveau, als je die allemaal twee jaar langer geeft, of drie jaar, als je dat gaat modelleren en gaat kijken wat de impact is op het ontwikkelen van mentale aandoeningen, ik noem iets volledig willekeurig, ik kan me voorstellen dat je dan een voor totaal ander aangrijpingspunt hebt. En dit kan heel belangrijk zijn, want stel dat je dan een veel, ik, echt volledig hypothetisch, dat je dan een veel grotere impact hebt, dan kan je met zo'n simulatiemodel en die resultaten, kijk wij kunnen dat niet eerst gaan uitvoeren, want we krijgen niet, we krijgen beleidsmakers echt niet mee dan, we krijgen het ministerie niet mee, maar met zo'n simulatiemodel kan ik me voorstellen, dan kan je misschien wel met ministerie, met verschillende ministeries om tafel, om te kijken van, en misschien wel met de bazen van de verschillende scholen en universiteiten na na na, om te kijken van hé luister eens even, wij hebben nu deze, dit simulatiemodel gemaakt, net zoals dat voortdurend wordt gedaan voor corona, en kijk nou eens, als wij investeren in die toegang tot GGZ dan komen we hieruit uit, maar als wij zeg maar alle jongeren nu drie jaar langer zouden geven, van middelbaar tot voortgezet, dan komen we hierop uit. Nou, tel uit je winst, wat zou je nou het beste kunnen doen. Dus dit zijn echt dingen, die kunnen wij, en waarom heb ik nu weer heel, weer een heel lang verhaal, maar dit zouden we onmogelijk voor elkaar krijgen zonder zo'n interdisciplinaire samenwerking. Ik weet niet of dit eruit gaat komen, maar ik denk wel dat dit iets, dat er een soort uniek momentum is waarin we elkaar vinden en waarin er ook belangstelling is, kijk nu wij praten met elkaar, jij bent natuurkundestudent en jij wil met mij praten, maar dat is niet alleen voor jou, dat is, er is ook, ik heb jarenlang op allerlei congressen van mensen die bezig zijn met AI en complex systems, heb ik als een soort verkoper, ik heb de hele tijd gezegd, omarm ons nou, als complex systems probleem, neem ons nou, wij zijn superinteressant, de prevalentie is heel hoog, en daar gaat er ook heel, gaat ook om heel veel geld, ik weet dat op andere gebieden is, banken, systemen, is ook heel veel geld te verdienen, maar op ons gebied ook. Er is heel veel

te verdienen als we dat slimmer gaan aanpakken. Hè, los nog van het feit dat je heel veel kan betekenen voor mensen persoonlijk, gigantisch veel, en niet alleen voor de persoon zelf, maar ook over generaties heen. En ik stond daar dan te praten en dan dacht ik, zie daar sta ik weer in Malta op één of ander internationaal congres buiten mijn veld, this was a complete waste of time, wat ben ik aan het doen. Maar nu is het anders, snap je, ik merk, er is een momentum, en je ziet dat er nu openheid is, zelfs van toppers, die komen dan van Princeton's en die denken ja, ik vind het best wel interessant om mij op dit gebied te gaan... Dus er is een momentum, en ik denk ook een momentum voor interdisciplinair werken en ik voel een ongelooflijke opwinding, ook al hebben we nog geen concrete resultaten, maar er is wel een momentum waarin verschillende velden bij elkaar komen en ik verwacht ook echt wel dat we op een soort, nou, ik verwacht dat we tot een soort doorbraak gaan komen die ik misschien nog wel zelfs ga meemaken. Nou.

**MG:** Dat lijkt me een hele mooie afsluiter.

**P1:** En ik ben altijd iemand van het glas halfleeg.

**MG:** Ja?

**P1:** Dus dat wil heel wat zeggen.

**MG:** Ja, ik ben door mijn onderwerpen heen.

**P1:** [...] klaar.

**MG:** Ik weet niet of er nog iets is wat je zou willen toevoegen, in dit kader?

**P1:** Nou, ja, ik ben natuurlijk heel benieuwd naar de uitkomst, van jouw geheel. En...

**MG:** Ja. Ja. Ik zet de opname eventjes stop dan.

**P1:** Ja.

## **Participant 2**

**MG:** Yes. Ja, voor we beginnen nog even iets over de verwerking van mijn data straks. Ik ga het interview dus transcriberen en de transcripten en de opnames die blijven bewaard, maar die zijn alleen beschikbaar voor mijzelf en voor mijn supervisors. Voor de verwerking uiteindelijk in het eindproduct, in mijn thesis, kan de inhoud zodanig worden geanonimiseerd dat het niet meer tot u te herleiden valt. Maar als u dat toestaat dan zou ik ook wel gebruik willen maken van de mogelijkheid om als het relevant is wel naar uw naam en uw achtergrond te verwijzen. Zou dat oké voor u zijn of heeft u liever dat het volledig anoniem blijft?

**P2:** Nee dat is prima hoor.

**MG:** Oké, prima. Ja, wat mij betreft kunnen we dan beginnen nu, als u verder geen vragen heeft.

**P2:** Nee.

**MG:** Helemaal goed. Nou, als korte introductie misschien eerst iets over uw onderzoek in het algemeen. Dus stel, u moet aan een collega die wetenschappelijk is opgeleid maar geen achtergrond heeft in, zeg, de medische wereld, in een paar zinnen beschrijven waar uw onderzoek over gaat, wat zou u tegen zo iemand zeggen?

**P2:** Ja. Dan zou ik zeggen dat ik, ik doe onderzoek naar de gezondheid van mensen met een verstandelijke beperking, en onze onderzoeksgroep is wat breder, die doet onderzoek naar geneeskunde en gezondheid van mensen met een verstandelijke beperking, maar ik kijk vooral naar de niet-medische kant van gezondheid, ik ben ook geen arts, en daarbij kijk ik dus naar allerlei andere aspecten van [...] gezondheid, waarbij context en omgeving een grote rol speelt, maar bijvoorbeeld ook communicatie, met artsen, hoe informatie op het juiste moment op de juiste plek komt, en vooral ook hoe we kunnen kijken hoe we in onderzoek goed aan kunnen sluiten bij de complexiteit van het dagelijkse werk, voor mensen die werken met mensen met een verstandelijke beperking.

**MG:** Ja. Oké. Ja, helder. Ja, ik hoor u net al het woord complex gebruiken, en ik begin natuurlijk ook vanuit de complexiteit...

**P2:** Ja.

**MG:** ...en dat is wel een begrip wat heel divers wordt opgevat door verschillende mensen. Dus wat verstaat u vanuit uw onder, achtergrond onder het begrip complexiteit?

**P2:** Ja. Ik denk dat voor mij het vooral is dat je breder kijkt dan alleen lineaire verbanden. Dus niet alleen maar A leidt tot B, maar dat je ook, dat je daar wat breder naar kijkt en welke processen daar dan een rol bij spelen, dat de tijd een belangrijke rol speelt hè, van wat, waarom zijn dingen zoals ze zijn, waarom gaan dingen zoals ze gaan. Ja, dus dat soort. Het is meer naar complexe relaties dan alleen de lineaire relaties. Ja ik denk dat dat voor mij wel een, ja, belangrijk kenmerk daarvoor is.



**MG:** Ja. En hoe groot is de rol van dat begrip complexiteit binnen uw eigen onderzoek op dit moment?

**P2:** Ja, ik heb er recent ook een paper over geschreven omdat er ook op zoveel verschillende manieren naar wordt gekeken. Ik ben zelf begonnen met het starten van een Europees netwerk rondom complexiteit in gezondheid, en ik merkte al van allerlei onderzoekers die er daaraan mee wilden doen dat die opvatting heel breed is, en dat er een heel groot gebied is dat vooral heel erg kijkt naar het modelleren, de mathematische complexiteit, en dat is net het stuk waar ik wat minder mee bezig ben. Dus ik zit echt meer op de complexiteit in processen, van hoe kun je daarmee sociale processen beter begrijpen, en hoe kan je verandering ondersteunen. Dus voor mij zit het meer in het stukje rondom systeemdenken, en systeeminnovaties, en minder als rondom het, ja, meer het wiskundige modelleren. Hoewel ik dat ook wel heel erg interessant vindt hoor.

**MG:** Want waar zit dat verschil dan in voor u?

**P2:** Nou, dat je dus wat minder rekent, dus op die, minder op die manier zichtbaar maakt, en meer gebruikt om processen tussen mensen te faciliteren of om te kijken wat daar dan speelt. En even een voorbeeld, even denken, als je zoiets hebt als overgewicht dan zou je natuurlijk kunnen gaan, daar zal je vast dingen op kunnen gaan berekenen, maar je kan ook heel goed, als je het heel lineair bekijkt, dan zeg je van nou, er komt teveel energie in en er gaat te weinig energie uit en dat leidt tot overgewicht, maar als je het complexer gaat bekijken dan is het meer de uitkomst van een serie van complexe processen, waarin heel veel verschillende systemen een rol spelen, en niet alleen maar het individuele systeem van energie in en energie uit, maar ook de omgeving, hoe is vervoer geregeld, dus het gaat alles met de auto of ben je makkelijk fietsen of met het openbaar vervoer, weet je, dat is ook weer een systeem op zich wat daaraan linkt, maar ook voeding, ja, is gezonde voeding makkelijk bereikbaar, dat soort dingen. Dus het gaat dan om interacties van systemen waaruit een bepaald iets ontstaat, dus bijvoorbeeld overgewicht, je hebt het bijvoorbeeld over de obesogene samenleving, zoals je het zou kunnen noemen, en, dus dat hoeft niet per se gekwantificeerd te worden en berekend te worden. Het kan ook een ander frame zijn om over een probleem na te denken, en dat is meer hoe ik het toepas op dit moment.

**MG:** Ja, want hoe vertaalt dat zich concreet dan naar onderzoeksmethoden, bijvoorbeeld in dit voorbeeld?

**P2:** Nou ja... Ja dat is eigenlijk al op meerdere vlakken hè, het begint al bij welke onderzoeksvraag wil je gaan beantwoorden. Ja ik zeg altijd van, het is doing different things and doing things differently, beetje op die twee manieren, en doing different things is dan dus ook dat je ander soort onderzoeksvragen gaat stellen, dus als je heel erg gericht bent op dat hele lineaire benadering, ja dan ga je je afvragen van hoe gaan we zorgen dat er minder energie in die mensen komt en dat er meer uitgaat, dus dan richt je je al heel snel op individuele voeding en beweging. Terwijl als je dus vanuit complexiteitsperspectief zou je daar andere vragen over gaan stellen, zo van wat maakt dat in deze situatie overgewicht ontstaat, of wat zijn elementen van zo'n obesogene samenleving en ook hoe is dit tot stand gekomen. Ja, dus dat, dan ga je dus meer kijken naar dynamiek over de tijd heen, in plaats

van een wat statischere lineaire situatie. Dus daar begint het al, met welke vraag ga je stellen. En op welke manier je die gaat beantwoorden dat is dan voor mij ook, dan is het ook passend om daar ruimte te geven voor die complexiteit, dus dat je ruimte geeft voor de dagelijkse praktijk om daarover mee te denken, dus dat je veel stakeholders daarbij gaat betrekken, en daar ook methoden voor gebruikt maar ook dus tijd en ruimte voor inplant, dat dat ook kan. Daar zijn ook allerlei tools voor hè, dat system dynamics modelling, dat kan je heel wiskundig benaderen als je het kan meten, als je de variabele hebt, maar je kan het ook als een soort gesprekstool gebruiken, waarin je gewoon met stakeholders ook in gesprek kan gaan van nou hoe ontstaat nou deze situatie, wat heeft daar nou een positief effect op en negatief effect op. Dus ja, een beetje op die manier. Beantwoordt dat je vraag een beetje?

**MG:** Jawel, ja, het mag vrij concreet van mij hoor, want u noemt nu dus vraagstelling inderdaad en dan stakeholdergesprekken en zo. Zijn er nog meer echt methoden die u toepast om echt die complexiteitsvisie te operationaliseren?

**P2:** Ja het is veel kwalitatief onderzoek wat wij doen, maar ook kwalitatief onderzoek kan je heel doelgericht inzetten, of veel breder inzetten, dus dat is, dat kan je, kwalitatief onderzoek kan nog steeds best wel een lineaire benadering zijn. Mensen denken vaak van, nou, als je kwalitatief onderzoek doet dan ben je al complex bezig, dat is ook op zich wel heel complex, maar dat is iets anders als dat je complexiteit daarin een plek geeft. Dus ook de manier waarop je je, ja, wie ook betreft bij je interviews en de manier waarop je het ook gaat analyseren, dat speelt daar ook wel een rol in. Dus dat nemen we dan wel mee in onze interviews, dus het is niet vaak zo dat wij één doelgroep specifiek interviewen, het is vaak dat we proberen een completer beeld te krijgen, dus niet alleen maar richten op mensen met een verstandelijke beperking maar ook op dat systeem eromheen, dus ook de dagelijkse begeleiders, ook andere gezondheidsprofessionals, verwanten, wie er ook maar betrokken zijn, om een zo breed perspectief te krijgen daarop. En daarna is het ook, hebben we ook vaak wel weer een soort terugkoppelingssessie, waarin we toch ook weer mensen uitnodigen om te reflecteren op wat we hebben gevonden, ja, om toch ook echt dat, hoe zit dat nou in de praktijk zichtbaar te krijgen. We doen veel inclusief onderzoek, dus dat is, ja, een manier van onderzoek waarin een doelgroep, bij ons dan mensen met een verstandelijke beperking actief betrokken zijn ook bij onderzoek, zodat zij ook echt mee kunnen denken over van, welke vraag gaan we nou beantwoorden en hoe gaan we dat aanpakken. Dus dat is voor mij ook wel een manier waarop we die complexiteit in een plek geven. Maar het begint voor mij wel echt bij die onderzoeksvraag, want heel veel methoden kan je zowel lineair als complex toepassen, en de onderzoeksvraag die maakt wat de insteek is.

**MG:** Ja.

**P2:** Dus dat is voor mij wel een belangrijk punt daarin. Ja. En daar zijn allerlei tools, zijn, systems thinking, rondom dat, ja dat system dynamics modelling, dat rich picture building, ook richting evaluatie dat je meer naar reflexieve monitoring gaat kijken als naar heel expliciete uitkomstmaten, dus die interventieonderzoeken kan dat zeker ook een plek hebben. Ja, dan is het ook de kunst om de goeie balans te vinden, als je echt een causaal verband aan wil tonen dan heb je daar gewoon, ja, geëigende onderzoeksmethoden voor

nodig. Maar het is dan heel fijn om die ook weer in context te kunnen plaatsen. Het is altijd een beetje zoeken naar de goede combinatie.

**MG:** Ja dus u maakt zelf ook gebruik van niet-complexiteitsmethodes?

**P2:** Jazeker, ja, ja. Ja, ik vind het vooral belangrijk dat je, ja, er goed bewust van bent wanneer je waarvoor gebruik maakt. Ja.

**MG:** En wat bepaalt voor u die keuze?

**P2:** Dat is, ja, de onderzoeksvraag is dan wel het uitgangspunt, wat wil je weten, en wat past daarbij. Als jij een effectiviteit van iets aan wil tonen dan past daar niet per se een complexe methode bij, maar als jij wil weten hoe je dat dan implementeert in een complexe omgeving, dan denk ik wel dat je heel veel misloopt als je daar niet ruimte voor geeft, om die complexiteit wel mee te nemen.

**MG:** En in hoeverre is die complexiteitsbenadering nou gangbaar in het veld waarin u uw onderzoek doet?

**P2:** Ja, ik doe onderzoek in gezondheids, ja, de gezondheidswereld, is het nog niet per se heel gangbaar. Het is, er is wel een fanatieke club mensen die er erg mee bezig is, en dat, daar zie je dat wel wat meer terug, maar de gouden standaard is nog steeds het randomised controlled trial onderzoek, wat heel erg lineair is van, ja oorsprong. Dus dat is nog wel echt een dominant perspectief. Ja. En dat zie je ook wel overal terug.

**MG:** En hoe komt dat denkt u?

**P2:** Ja, dat komt heel erg vanuit medicijnonderzoek. En dat is ook de manier om medicijnonderzoek te doen hoor, bijvoorbeeld, dat zal ik niet ontkennen. Maar inmiddels zijn onderzoeksvragen binnen gezondheidsonderzoek veel breder als dat geworden, en, ja, wordt de methode soms een beetje leidend aan de onderzoeksvraag, en dat is wel, wel jammer, gaat wel veel verloren, zeker voor een complexe doelgroep zoals mensen met een verstandelijke beperking. Ja.

**MG:** Want hoe bent u er zelf bij gekomen om dan richten die complexiteitsmethoden te stappen in plaats van die randomised controlled trials?

**P2:** Ja, dat is eigenlijk al tijdens mijn promotieonderzoek gebeurd, dat ging over hoe kunnen we ouder wordende mensen in gemeentes ondersteunen, meer gezondheidsbevorderingsgericht, en het zat al een beetje in het project waar ik mee ging beginnen omschreven hoor, dat ik op die insteek zou gaan werken, maar wat ik me nog heel goed kan herinneren is dat ik, toen was ik net begonnen met mijn promotieonderzoek, op een congres was waar iemand vertelde over een interventie voor oudere mensen, dat was een fitnessinterventie, dus die konden op de sportschool een aantal weken achter elkaar oefeningen komen doen, was een programma, en daarin zou dan gemeten worden of dat nou effect had op fitheid. En die had echt een ontzettend ingewikkeld design opgezet en de training helemaal uitgedacht en evaluatie opgezet waarin mensen dan voor die tijd en na die tijd allerlei oefeningen moesten doen, konden ze dan berekenen of ze fitter waren geworden. En daar kwam helemaal niks uit, in ieder geval er kwam niet uit dat daar een verschil in was,

in hoe fit mensen waren. Dat was echt heel zonde als je dat hoorde, het was echt een heel mooi goed opgezet onderzoek, maar het stomme was dat zij vertelde laat, vertelde tijdens de presentatie dat ze van, ja, eigenlijk uit de procesevaluatie kwam van dat ze heel veel brieven had gekregen van deelnemers die zeiden, ja, sinds ik meedoe aan de training pak ik ook vaker weer zelf de stofzuiger, of nu loop ik weer naar de supermarkt om mijn boodschappen te doen. En ik denk, ja dat zijn allemaal dingen die heel veel impact hebben op iemands dagelijks leven en die jij dus niet mee hebt genomen in jouw evaluatie, maar wat dus eigenlijk helemaal niet wil zeggen dat jouw interventie niet effectief was, want voor die mensen was dat dus heel erg wel. Dus als je een iets bredere bril had gehad, of misschien ja, daar dan, toen wist ik nog niet dat dat dan complexiteit of systeem, systems thinking zou heten, dan had je dit misschien wel zichtbaar kunnen maken, en dat had heel veel extra informatie opgeleverd over wat iets betekent in het dagelijks leven van mensen. En dat is waarom ik het heel waardevol, als heel waardevol perspectief ook ben gaan zien, dat is in ieder geval iets wat ik me echt kan herinneren van het hele begin dat ik dacht, oh dat is echt zonde als je dit alleen maar lineair aanvliegt, ja, dat kost iedereen heel veel tijd en energie en geld en het is net alsof er niks gebeurd is, terwijl er best wel wat is gebeurd.

**MG:** Ja. Ja, en u noemde net ook al dat u zelf wat minder naar de kwantitatieve complexiteitsmethodes trekt. Wat is daar de reden voor voor u?

**P2:** Ja, daar moet je ook wel echt andere skills voor hebben hoor, dan moet je statistisch en wiskundig ook wel heel sterk voor staan. En, ja, zo is het bij mij gewoon ook niet gelopen dat ik dat heb kunnen ontwikkelen, je moet daar ook de data voor hebben, en het onderzoek naar hebben dat je dat kan gaan doen. Dus ik vind het zeker heel erg interessant en ik zou het zeker heel leuk vinden om dat een keer wel op te gaan pakken, als de kans zich voordoet, maar dat is niet het type onderzoek wat wij op dit moment uit kunnen voeren.

**MG:** Ja, maar denkt u dat het zou passen bij uw onderzoekslijn?

**P2:** Ja...

**MG:** Het sluit elkaar niet uit per se?

**P2:** ...nee, dat denk ik niet, nee. We kijken ook, mensen met een verstandelijke beperking hebben ook veel multimorbiditeit, waar nu ook heel lineair eigenlijk naar wordt gekeken, dus dat is bijvoorbeeld, dat is nou typisch zo'n onderwerp waar het wel goed bij zou passen, de impact daarvan op hun gezondheid en ook medicatiegebruik, interacties tussen medicatie, ja, waarvan ik ook wel weet dat René en Marcel daar ook wel mee bezig zijn. Dat is een onderwerp wat heel interessant is, waar wij op dit moment misschien de data ook nog niet voor hebben om daar wat mee te kunnen doen, omdat de sector dat gewoon niet heeft, maar we zijn daar ook wel stappen in aan het zetten omdat [...] dat, misschien ook wel weer wat complexiteitlinken heeft, met machine learning en zo, om te kijken of we daar toch wel meer data over kunnen krijgen. Maar dat, dan heb je wel echt iets nodig waar je mee kan rekenen, en dat hebben we op het moment helaas niet.

**MG:** Ja. Even zien. Ja, u heeft, natuurlijk, even zien hoor. U noemde net al dat technieken die u gebruikt, zijn dit ook technieken die niet per se afkomstig zijn uit de gezondheidswetenschap, dat zijn meer kwalitatieve technieken, hè?

**P2:** Ja. Oeh, dat vind, dat zou ik zo niet weten hoor. Ja, dan zou je echt wel moeten weten, wat komt er wel en niet uit de gezondheidswetenschap. Nou ja, ik weet, ik werk veel met een concept van innovatiesystemen, dat komt uit landbouwwetenschap, dus daar kan ik heel duidelijk van zeggen dat dat heel ergens anders vandaan komt. Ik ben gepromoveerd in Wageningen, dus dat is natuurlijk landbouwuniversiteit, en ik heb, mijn promotie zat daar bij communicatiewetenschappen, bij innovatiestudies, en die werken al langer met dat soort ideeën, en dan gaat het ook heel erg rondom implementatie. Ja, landbouwwetenschappen heeft ook, die lopen daar voor mijn gevoel iets op voor, die hadden natuurlijk ook een hele ontwikkeling van nieuwe soorten zaden of landbouwbestrijdingsmiddelen en zo, die op een bepaalde manier gebruikt moesten worden en daar moesten boeren ook uitleg over krijgen, van hoe ze dan met hun land om moesten gaan en met die producten die eigenlijk ontwikkeld waren in Wageningen. En zij gingen daar eigenlijk over, van hoe gaan we nou die boeren zover krijgen dat ze dat gaan doen. En die kwamen dus ook heel erg op een wat complexere benadering, en dan vanuit het systems thinking en innovatiesysteem gezien. En ik heb dat eigenlijk al een beetje doorvertaald naar rond, naar gezondheidsbevordering, waar eigenlijk nog heel erg het idee leefde, dat is ook alweer een tijd geleden, vijftien jaar geleden nu, van ja, als we mensen vertellen dat ze twee ons groente moeten eten en dertig minuten moeten bewegen, dan snappen ze wel dat dat goed is en dan gaan ze dat wel doen. Nou daar weten we inmiddels wel dat dat niet zo werkt. Dus dat, dat je daar toch echt meer voor moet doen, meer moet kijken naar wat zit er dan in de omgeving wat ander gedrag wel of niet mogelijk maakt, wat zijn motivaties van mensen en hoe ga je daarmee om, en dan had je in eerste instantie dat theory of planned behaviour wat nog steeds wel heel lineair was, want dan zei je van nou, als je, als iemand een motivatie heeft en zijn vrienden vinden het belangrijk en hij heeft de juiste tools, dan gaat hij vanzelf dat gedrag vertonen. Nou, ook dat bleek niet helemaal zo te werken in de praktijk.

Dus en dan, kijk, kom je een beetje op die innovatiesysteembenadering die gaat kijken van nou, je hebt een bepaalde functie voor ogen, wat er moet gaan veranderen, wat zijn er, wat zijn dan de structuren die daaronder liggen die zo'n verandering helpen, vooruit helpen of niet. Dus dat is nog weer anders wat je veel in gezondheidsonderzoek, tenminste wat ik wel veel zie is dat het gaat over barriers en facilitators voor verandering, dat geeft ook een beetje het idee dat als je maar zoveel mogelijk facilitators hebt en zoveel mogelijk de barriers weghaalt dan komt het wel goed. Dat innovatiesysteem dat werkt meer vanuit het idee van, nou er zijn bepaalde mechanismes die verandering in de weg zitten, die het dus blokkeren, die de functie eigenlijk blokkeren, wat zijn dan de onderliggende structuren, dus je gaat dat op een andere manier in kaart brengen, van wat zijn nou structuren in dit systeem die een verandering faciliteren of tegenhouden. Ja, zodat je daar ofwel bewust van wordt of daar op in kan spelen. Het gaat dan ook heel erg in, over de interacties tussen al die blocking mechanisms, meer als zo het min mogelijk barriers en zo veel mogelijk facilitators hebben. Dus het, en ja dat komt heel erg vanuit, ja, de landbouwwetenschappen, ontwikkelingsstudies, [...] in Wageningen.

**MG:** Ja en hoe soepel of hoe moeilijk ging dat doorvertalen, naar...

**P2:** Oh dat gaat nog steeds heel moeilijk. En het blijft, ik vind het ook nog steeds ingewikkeld uit te leggen hoor, dat je bezig bent met complexity en systems thinking en wat daar dan de meerwaarde van is en waarom je dat zou moeten doen. Als iemand het begrijpt en er ook mee werkt dan praat je zo twee uur vol en dan weet je precies waar je het over hebt, als je het aan iemand uit moet leggen die vanuit een lineair perspectief komt, blijf ik blij dat heel ingewikkeld vinden. Ja.

**MG:** Want wat gebeurt er dan bijvoorbeeld?

**P2:** Ja, dan, de vraag kan komen van ja, maar dat is dan toch gewoon kwalitatief onderzoek, en wat is dan het verschil, of het is meer van ja, op die manier kan je nooit wat aantonen. Ja dat is misschien ook helemaal niet je doel, weet je, dat is, daar, dat zit, begint hem al in dat je andere onderzoeksvragen stelt en je inderdaad andere dingen interessant vindt. De manier van werken, nou ja, dat is ook zo'n systeemkenmerk natuurlijk hè van gezondheidszorg, dus dan heb je het alweer over, dan zit je alweer vanuit een complexity perspectief te kijken. Je hebt, ja je ontwikkelt iets in het lab en dan implementeer je het in de praktijk en dan evalueer je het, en dan werkt het of niet, en zo niet dan ga je weer door, dus dat is ook een heel lineair stapsgewijze manier van werken, dus het is, ja, dat staat best, het staat gewoon heel erg in uitgangspunten al heel ver van elkaar af. Ja, ik vind dat moeilijk. Wat mij nog het meeste daarbij heeft geholpen is die paper die ik recent heb geschreven van hoe ga je nou daarmee om en hoe ga je ook proberen om het een beetje te integreren dus niet altijd als of het één of het ander te zien. Het heeft ook wel heel erg tegenover elkaar gestaan hè, wat je ook tegenkomt dat mensen zeggen van ja, je moet het ook niet te, je moet het niet te complex willen maken, het is juist onze taak om het te versimpelen. Ja, dat was ook niet per se de bedoeling, maar complexiteit roept dan meteen het idee op van dat je iets heel ingewikkeld wil maken. Ja misschien in de gedachte daarachter, maar niet in hoe het in de praktijk moet gaan. Dus dat, dat soort dingen daar loop ik dan wel tegenaan, ja. Ja het past gewoon, het is, het past totaal niet bij medisch gedachtegoed.

**MG:** Ja. En hoe lost u dat dan op, of hoe gaat u daarmee om als u dat soort verschillen merkt?

**P2:** Ja, hoe los je dat op. Dat is best lastig, op te lossen. Het is heel fijn als je medestanders vindt, dat helpt. Ja. En, dat voor, en voorbeelden laten zien, daar, wel daarover blijven schrijven, meestal, ja het is echt een beetje, je vindt vaak wel mensen die daar wel daarin geïnteresseerd zijn en vanuit daar dan weer een stapje verder proberen te komen. Maar, ja, de kern zit denk ik voor mij wel vooral in wel aansluiting te blijven zoeken, en vragen te blijven stellen, ja.

**MG:** Ja. Want merkt u echt een tweedeling dan op dit moment?

**P2:** Het wordt wel minder hoor. Maar dat was wel heel erg zo, ja.

**MG:** Hoe zag dat er dan uit?

**P2:** Ja, wat ik net ook zei hè, dat, van ja, hoezo complex, het is al complex genoeg, we moeten het juist simpeler maken, en dat soort uitspraken, ja. Ja, en een beetje wat je ook wel, dat is wel langer geleden heb gehad, de tegenstelling tussen kwalitatief en kwantitatief onderzoek, ja, dat kwalitatief onderzoek ook niet als onderzoek wordt gezien, omdat onderzoek wordt gezien als iets waarmee je het effect van iets moet aantonen. Ja, dat hoeft natuurlijk niet, dat ligt heel erg aan je onderzoeksvraag. Dus, ja daar komt het voor mij dan ook wel steeds op terug, en je moet ook wel goed kijken van wat is dan de onderzoeksvraag, en wat is de passende manier om die te beantwoorden.

**MG:** Ja. Maar u zegt, u merkt dat het verbetert, die verbinding?

**P2:** Nou de, ik merk dat het wel, er is nu steeds meer aandacht voor, en dat maakt wel dat er wat ruimte voor ontstaat ook. Ik ben recent betrokken geweest bij een grote subsidieaanvraag binnen de nationale wetenschapsagenda, en die vroegen expliciet om een systeemaanpak voor het bestuderen van gezondheidsongelijkheid bij mensen in armoede, nou ja, daar was het dus echt de bedoeling dat je complexitybenaderingen toe ging passen. Dus dat, ja dat maakt wel dat ineens mensen wakker worden, zo van oh hier weten we helemaal niks van, dus ik werd ook van alle kanten ineens gemaïld van hé heb jij daar niet ooit eens iets over verteld en, kan jij niet met ons meedenken. Dus dat soort dingen dat helpt wel, dat daar ook weer wat meer aandacht voor komt. Je ziet ook af en toe wel weer eens, wel papers ook in Nederlandstalige bladen daarover verschijnen. Ja, nou ja, en het RICH-netwerk is daar natuurlijk ook een goed voorbeeld van.

**MG:** Ja.

**P2:** Hoewel die wel heel erg op het wiskundige zitten, onder [...]. Maar dan nog steeds is het uitgangspunt daarvan wel van, ja, dat je een ander type onderzoeksvraag wil gaan beantwoorden waarvoor je die complexe benadering nodig hebt, en dat blijf ik interessant vinden, ongeacht of je dat nou heel erg op het wiskundige toepast of meer op het kwalitatieve en het sociale. Dat uitgangspunt, die, dat ander type vragen, dat is wat ik, dat zijn de vragen die ik interessant vind, om onderzoek naar te doen. Dus ongeacht welk spoor van complexity-onderzoek daarin dan past.

**MG:** Ja. Ja, en binnen dat complexiteitsonderzoek, voor dit soort projecten, werkt u dan ook wel eens samen met mensen uit andere disciplines?

**P2:** Ja, ja. Dat is ook wel voor mij een kenmerk is dat het heel erg interdisciplinair is, om op deze manier, of op, ja, het soort vragen wat je dus krijgt vanuit zo'n complexiteitsperspectief die zijn gewoon heel erg interdisciplinair, dus in die zin, ja, zeker. Dus, en dan gaat het, gaat die samenwerking niet per se altijd over complexity hoor, dan is dus gewoon de onderzoeksvraag is dan vanuit, ja, complexiteitsperspectief ontstaan en dat maakt dat je gewoon meerdere disciplines nodig hebt. Dus en dat kan heel breed zijn hoor, met informatietechnologie, met Science in Society van, dus dat is, ja, van de technische faculteit van de Radboud, dus samen, maar ook met andere afdelingen in het ziekenhuis, ja, nu recent weer met tandheelkunde bijvoorbeeld, dan zijn we aan het kijken wat we op kunnen gaan pakken, dus dat soort dingen ontstaan er dan, communicatiewetenschappen bijvoorbeeld [...], nou ja, onderzoeksmethodologen, ja.

**MG:** Dus heel breed eigenlijk?

**P2:** Ja.

**MG:** En dan, als u nou naar zo'n samenwerking kijkt, hoe zijn de rollen dan verdeeld, hoe gaat dat concreet?

**P2:** Poeh. Ja, heel vaak zit zo'n samenwerking rondom een promotietraject, dus dan is het in een begeleidingsteam komen eigenlijk al die disciplines wel terug, en een promotietraject heeft meestal drie of vier onderzoeksprojecten die daar in zitten, en vaak zie je dan dat één van de expertises de nadruk krijgt in één van die onderzoeksprojecten, en dat daar dan dus ook meer op dat moment in dat, in zo'n project daar weer de nadruk op ligt en andere disciplines misschien daarbij mee kunnen denken. Nou ja, dat maakt het altijd wel heel interessant, vind ik. Dus dat is een beetje denk ik hoe die rolverdeling gaat.

**MG:** Heeft u een voorbeeld misschien, van zo'n promotietraject?

**P2:** Ja, even kijken hoor, wat een handige is. We hebben er eentje gehad over gezondheidsbevordering bij mensen met een verstandelijke beperking, en daar hadden we dan expertise in van een huisarts, van een fysiotherapeut, van een gezondheidswetenschapper, dat zat dan allemaal in het begeleidingsteam. En van de public health expert, dus dan ging het ook, dus dan zat er stukken in wat heel erg ging over hoe ervaren mensen met een verstandelijke beperking hun gezondheid en wat vinden ze daar belangrijk in, nou dat zat dan heel erg bij degene die kennis had over inclusief onderzoek en over mensen met een verstandelijke beperking. Maar er zat ook een heel stuk in van nou hoe gaan we nou kijken naar een interventie die bij kan dragen aan die punten die zij noemden, en hoe gaan we dat dan in de praktijk invoeren, daar zat wel veel meer inbreng weer in vanuit fysiotherapie van hoe dat eruit gaan zien, en veel uit public health perspectief werd ook weer heel erg gekeken van hoe gaan we dat dan evalueren en wat is daar dan belangrijk in. Ja. Nou ja, en één van de uitkomsten daarin was bijvoorbeeld dat mensen met een verstandelijke beperking heel goed kunnen oplepelen wat wordt verteld over gezond leven, maar als ze dat dan moeten doorvertalen naar hun eigen dagelijkse leven, dat dat heel moeilijk is, dus dat het helemaal geen zin heeft om te gaan zitten vertellen, wat er allemaal belangrijk is voor gezond leven, want ja, dat onthouden ze wel maar daar kunnen ze niks mee, dus dat we veel meer, dat we in die interventie dus vooral ruimte moesten creëren waarin mensen om hen heen naar hun zouden gaan luisteren, dus wel vragen zouden stellen van wat vind jij belangrijk, maar dan vooral ook zouden luisteren naar waar kwamen zijn dan mee, en dat dan ook door zouden gaan vertalen. En wij, dat is voor mij, voor mijn gevoel typisch iets wat niet naar voren was gekomen als we daar een heel lineair perspectief op hadden gehad, dan was je toch meer gaan kijken van nou, mensen bewegen te weinig, nou dan moeten we een beweeginterventie op gaan zetten, terwijl die, dat hele project nu eigenlijk is gegaan van hoe identificeren we dingen in het dagelijkse leven van mensen, dus zeker niet op projecten gericht, want projecten die starten en die stoppen en die zijn weg, maar juist, en juist doordat weer mensen met een verstandelijke beperking zelf ook daarover na gingen denken kwamen er allerlei tips naar voren die voor hun relevant waren en uitvoerbaar waren zo, en dat waren dingen waar wij eigenlijk nooit aan hadden kunnen



denken, omdat je hun perspectief daarvoor nodig had, zoals een halte eerder uit de bus stappen, of als je op visite gaat bij iemand die op de vierde verdieping woont dat je dan twee verdiepingen met de lift gaan en de rest de trap pakt. Ja, dat, allemaal van die kleine dingetjes, ja, die waren heel erg leuk, was heel leuk om zo op die manier aan een project te werken. Maar daar moest je dus echt ruimte creëren voor een ander perspectief, en dat is voor mij ook wat dat systems thinking wel heel erg brengt.

**MG:** Ja. Want hoeft heeft u, of hoe hebben jullie dan in dat project al die verschillende visies eigenlijk geïntegreerd tot één geheel?

**P2:** Ja dat zijn meerdere studies geweest. Dus, we zijn begonnen met die studie, een focusgroepstudie, rondom mensen met een verstandelijke beperking, maar ook in hoe die focusgroepstudie opgezet werd, moesten we al nadenken over hoe gaan we echt bij hun perspectief komen, want je kan natuurlijk ook gewoon vragen gaan stellen van nou, hoeveel beweeg je, waarom beweeg je niet meer, hoeveel zou je willen bewegen, maar we moesten ze echt aan het praten krijgen over hun dagelijkse ervaring van gezond leven. Dus daar ga je al bedenken dat je een ander type vragen moet gaan stellen. En er zijn ook gewoon studies geweest van wat is dan nu de situatie, hoe ziet die er nu uit, daarnaast zijn ook allerlei andere stakeholders geïnterviewd en wat zij denken dat hun rol is rondom dat, die levenssituatie van mensen met een verstandelijke beperking. En dat is uiteindelijk allemaal bij elkaar gelegd.

**MG:** Ja. En als u nou kijkt gewoon naar u, de samenwerkingen die u heeft gehad in het algemeen met wetenschappers uit andere disciplines, heeft u dan wel eens meegemaakt dat er begripsproblemen of communicatieproblemen voorkwamen?

**P2:** Ja, dat komt eigenlijk altijd wel voor denk ik. Ja, zeker. Ja. We zijn daarom ook gaan werken met een model voor interdisciplinair onderzoek, waarin je al begint bij de onderzoeksvragen, dat al, ja, op een goede manier te bespreken met elkaar van wat verstaan we hieronder en hoe gaan we dit aanvlagen, wat vinden we hierin belangrijk.

**MG:** Want heeft u een voorbeeld van een situatie waarin dat bijvoorbeeld misging met zo'n begrip bijvoorbeeld?

**P2:** Ja, moet ik heel even denken hoor. Dat vind ik wel lastiger... Ja dat, weet niet, wat me nu het snelste naar voren komt is vanuit mijn eigen promotieonderzoek nog, dus dat is wel langer geleden, waarbij we eigenlijk ook de combinatie moesten maken van meer epidemiologisch onderzoek en meer sociaal-wetenschappelijk onderzoek, en daarin was een groot bevolkingsonderzoek eigenlijk gedaan of een vragenlijstenonderzoek onder ouderen, om te kijken wat er, wat, nou, hoe het stond met de gezondheid, en daar kwam uit dat ik geloof negentig procent van de ouderen de eenzaam was, volgens een bepaalde schaal die je daarvoor kon gebruiken, en de gemeentes die waren zich helemaal de blubber geschrokken daarvan. Maar ja, die cijfers op zich die zeggen eigenlijk helemaal niet zoveel, dus ook, dus dat was, ja, dat vonden wij vanuit die sociaal-wetenschappelijke kant dan weer lastig want ja, wat zeggen die cijfers dan, die zeggen nog niks van hoe mensen dat nou in hun dagelijks leven ervaren. En waar dan de grootste wrijving in zat van ja, maar hoe mensen het ervaren dat kan je eigenlijk niet meten, of tenminste, dat hebben we gemeten met die schaal, maar dat, ja, dat, en vanuit sociaal-wetenschappelijk oogpunt vind je dat dan eigenlijk

niet genoeg zeggen, terwijl zij zoiets hebben van ja we hebben dat gemeten en nu is het zo. Dus dat was een beetje een, dat was in ieder geval een beetje een aanvaring waar we best wel druk mee zijn geweest om dat uit te puzzelen, ja, hoe ga je dan toch voor beide perspectieven ruimte geven.

**MG:** Want hoe bent u daar dan mee omgegaan uiteindelijk?

**P2:** Ja, dat moest echt op, we waren met vier promovendi, twee vanuit de ene hoek en twee vanuit de andere, en dat moesten we echt onderling moesten we dat bespreken, dat heeft best veel tijd gekost. Maar we merkten dat wij er nog wel makkelijk uitkwamen, maar dat bij onze begeleiders die dus, die echt al wat meer in één discipline geworteld zaten, dat het daar nog wel moeilijker was. En dan ook, hoe ga je, er moest dan natuurlijk een interventie komen tegen eenzaamheid, hoe ga je dat dan evalueren, en hoe zinvol, hoe zinvolle informatie levert dat op, dat was best ingewikkeld, nee dat kan ik me bijvoorbeeld goed herinneren.

**MG:** Ja. Kunt u iets meer vertellen over hoe die discussies dan gingen bijvoorbeeld?

**P2:** Ja dat je, als je het niet kan meten dat je het ook niet aan kan tonen, dus je wil dan een voormeting en een nameting doen rondom die eenzaamheid, en dan doen mensen eerst van tevoren een schaal invullen en dan weer achteraf, en dan wil je eigenlijk ook nog dat je gemeentes hebt waarin je die interventie gaat doen en gemeentes waarin je geen interventie gaat doen. Dat was heel erg, ja lineair epidemiologisch perspectief op hoe dat zou gaan werken, maar als je meer een public health perspectief hebt, mensen die blijven natuurlijk niet een aantal maanden alleen maar in hun gemeente, weet je, die komen ook in een andere gemeente, die zien daar ook, nou ja, alleen dat al die kunnen daar zien van die interventie hoe die er dan ook uitzag gezien wat daar loopt, dus je kan dat eigenlijk, je kan dat in de tijd dan eigenlijk niet meer controleren. Je kan wel doen alsof, maar ja, hoe zinnig is dat dan, weet je, dus dat waren dan gesprekken die we daarover gevoerd hebben, van ja, hoe gaan we dat dan aanpakken, want eigenlijk is het gewoon een combinatie geworden, van een heel uitgebreide procesevaluatie en een effectevaluatie. Nou ja, en zoiets hebben we ook wel gezien in onderzoek wat recenter rondom die gezondheidsbevordering heeft gelopen, dat niet, ja, beetje vanuit een meer lineair perspectief wilden ze graag gaan kijken met stappentellers of mensen nou ook echt meer gingen bewegen, ja dat kan je doen, weet je, dan ga je voordat je je interventie doet mensen met stappentellers drie dagen rond laten lopen en daarna, maar die stappentellers zijn dan helemaal niet echt gevalideerd voor de doelgroep, en die worden niet allemaal goed gebruikt en, ja, dat is, je haalt je een boel ellende op de hals en uiteindelijk levert het helemaal geen goeie kwaliteit data op. Dus dan heb ik liever dat we van te voren er iets langer over nadenken over wat is nou, zijn er voorwaardes om dit goed te kunnen evalueren, ja, wat moeten we daar wel of niet bij meenemen. Dus eig-, dus ja, heel concreet terug naar jouw vraag, anders heb je er ook niet zoveel aan, ik denk dat ik veel van die misverstanden of wrijvingen, spraakverwarring heb gehad rondom evaluatiedesigns, want als je iets wil evalueren dan wil je dat ook op een goeie manier doen en dan moet je inderdaad wel met een soort gecontroleerde experimentsetting werken, maar je moet wel weten wat je mee wil nemen, en op welke manier je dat wil gaan doen en daar speelt die context wel een heel belangrijke rol in, dus het staat wat minder, ik ben absoluut voor om dingen op die lineaire manier te evalueren maar

wel op het juiste moment, en op de juiste manier. Ja, en daar moet je wel met elkaar uitkomen. Ja.

**MG:** Ja. Ja, u noemde net ook dat model voor interdisciplinaire samenwerking, klopt dat?

**P2:** Ja.

**MG:** Kunt u daar iets meer over vertellen misschien?

**P2:** Ja dat is, ja het MIR-framework heet het, dat weet ik even zo gauw, Multi, ik weet eigenlijk niet waar het voor staat, zal het even op moeten zoeken, en dat gaat, dat laat eigenlijk een heel onderzoeksproces zien, en we gebruiken het nu veel in kwalitatief onderzoek ook om het kwalitatief onderzoeksproces wat transparanter te maken, daar wil nog wel eens wat mysterieuze toestand eromheen hangen en dat wil je eigenlijk ook niet, dat helpt niemand. Maar het kan ook voor kwantitatief onderzoek gebruikt worden, en het laat eigenlijk vooral zien bij iedere stap in je onderzoek vanaf je formuleren van je onderzoeksvraag maar eigenlijk daarvoor al, van wat is nou je probleemsituatie of waar wil je wat aan gaan doen, naar je onderzoeksvraag, naar je methode helemaal uitgewerkt, en wat wil je hier bespreken, en waar hebben we het precies over en hoe gaan we dat vormgeven. Maar ook het synthesestukje waar je ook net naar vroeg, van hoe breng je nou al die verschillende dingen dan bij elkaar, dat heeft daar ook een plek in. Dus het is meer iets wat je gedurende zo'n heel onderzoek mee kan laten lopen om met elkaar te, goed te kijken van oh, wat moeten we op dit moment bespreken, ja, waar kunnen we verwachten dat we misschien andere, vanuit een andere achtergrond ernaar kijken.

**MG:** Ja. En merkt u dat dat helpt, zo'n model?

**P2:** Ja, dat helpt enorm, ja.

**MG:** Op wat voor manier?

**P2:** Nou ja, heel veel dingen die jij, die je impliciet doet als onderzoeker, daar sta je er niet bij stil dat dat voor een andere, vanuit een andere discipline een heel andere betekenis kan hebben. Dus dat model dat haalt dat even naar voren, zo van oké kijk, ik zeg je, zorgt, waar heb je het over in, als je het hebt over je methode, oké je gaat een kwalitatieve methode doen, wat betekent dat dan voor het, voor je werk en wat betekent dat voor je dataverzameling, wat betekent dat voor je analyse, om... Ja, dus je kan, jij maakt even duidelijk, in plaats van dat je zegt van nou ik ga interviews doen, en dan komt daar dit uit, weet je dan denkt iemand met een meer, vanuit een meer kwantitatieve discipline denkt van ja, oké, nou het zal wel maar ik kan daar niks mee, terwijl als je even expliciet maakt van, nou dit is het doel en op deze manier gaan we werven daarmee, dus je kan geen powerberekening doen als je een kwalitatief onderzoek gaat doen, en wat ga je, welke stappen ga je dan zetten om toch de validiteit van je onderzoek te vergroten. Dus je kan iemand daar, ja je kan dan gewoon elkaar goed meenemen in waarom je welke keuzes maakt. Dat helpt enorm, ja.

**MG:** Het MIR-framework heette dat, of?

**P2:** M-I-R, ja. Ik kan, zal ik het naar je doorsturen, vind je dat handig?

**MG:** Ja, is misschien wel handig ja, graag. Bedankt.

**P2:** Ja. Ja, dat is, het is ook geschreven door een methodologe uit Wageningen, die veel met interdisciplinair onderzoek doet. Volgens mij is het geschreven vanuit het perspectief vanuit hoe ga je daar, hoe ga je lesgeven over onderzoeksmethoden aan een interdisciplinair publiek, maar, [...]. Ja het is niet zo dat we het allemaal op de letter volgen, maar het helpt gewoon om je er bewust van te zijn.

**MG:** Ja, ja. Ja, dan wil ik nog even door naar een stukje ander onderwerp, want ik heb, krijg het idee aan wat u nu vertelt van dat uw onderzoek best wel dicht echt op de praktijk staat. Maar als u nou kijkt naar dat, het hele spectrum van aan de ene kant heel fundamenteel onderzoek en aan de andere kant, ja, onderzoek dat al klaar is voor een toepassing eigenlijk, waar in dit spectrum zou u uw eigen onderzoek ongeveer plaatsen?

**P2:** Ja, meer bij dat toepassingsgerichte stuk onderzoek. Ja.

**MG:** Ja. Want waar zit dat hem dan in?

**P2:** Nou ja, we, ook gewoon van de manier van werken, dus van we zijn onderdeel van de academisch werkplaats hè, dus we werken veel samen met zorgorganisaties, dus het type onderzoek wat we nu bij ons verrichten is heel praktijkgericht, is absoluut niet fundamenteel in die zin.

**MG:** En wat voor toepassingen moet ik aan denken dan?

**P2:** Ja, hoe gaan we gezondheidszorg beter toegankelijk maken voor mensen met een verstandelijke beperking, ja het is wel vrij breed hoor, dus gezondheidsbevordering is daar wel een groot onderdeel van. Ja, wat ik net zei, dat, die aanvraag waar we mee bezig zijn, van hoe kan je gezondheidsachterstand van mensen met een lage sociaal-economische status verkleinen. Het zijn, het gaat allemaal heel erg over sociale netwerken en sociale dynamiek, hoe versterk je samenwerking met de praktijk, en dat soort vragen. Dus dat is heel erg van hoe zorg je ervoor dat mensen met een verstandelijke beperking op een zinvolle manier mee kunnen denken in onderzoek, wat komt daar dan kijken. Dus het is heel erg het type vragen wat op dit moment bij ons ligt wat wel echt wel aan die praktijkgerichte kant zit en niet aan de fundamentele kant.

**MG:** Ja. En op wat voor manier dragen de complexiteitstechnieken die u gebruikt bij aan dit soort toepassingen?

**P2:** Ja, hm. Ik weet niet zo goed of het dan complexiteitstechnieken dan zijn. In die zin gebruik ik dan het meest dat innovatiesysteemframework, en wat daar vooral heel erg bijdraagt is om gewoon goed te, de complexe dynamiek van die dagelijkse praktijk te begrijpen. In een onderzoek ga je het wel vrij snel wel wat platslaan hè, omdat je toch wil kijken van nou, wat is het effect van dit op dat bijvoorbeeld, ja, dat probeer je dan een beetje te voorkomen, om toch echt wel, het probleem uit de praktijk goed naar voren te halen. Ja, ik denk dat het daar heel erg aan bijdraagt. En ook wel om begr-, ik merk ook wel, ja we werken ook heel veel samen met mensen uit de praktijk, in klankbordgroepen of dat, dat doe ik allemaal op die manier, dat zij zich ook echt wel gehoord voelen door de type vragen wat je

dan ook stelt aan hun, van wat komt er nu bij jullie heel erg naar voren, en dat framework helpt mij ook heel erg om het achterliggende probleem zichtbaar te maken, wat je dus erg ziet bij implementatieonderzoek is dat er ook gewoon maar een heel erg symp – het wordt heel snel symptoomgericht, dus ze gaan, ja dan wel, begeleiders vinden het moeilijk om mensen met diabetes, dagelijks begeleiders vinden het heel moeilijk om een cliënt die diabetes heeft goed te ondersteunen. Nou, dan gaan we een poster maken over wat moet je doen bij een cliënt met diabetes. Nou die wordt dan gemaakt, en die poster wordt dan geïmplementeerd en geëvalueerd. Maar is dat nou echt het probleem wat er speelt, dat is dus als je het heel lineair bekijkt, maar ik wa-, op de manier waarop wij ernaar kijken horen we veel meer dingen, en die begeleiders die lopen tegen heel veel dingen aan. Ja wat blijkt nou, al die begeleiders die hebben een sociaal-pedagogische achtergrond, en in die opleiding komt eigenlijk niks over gezondheid naar voren. En ze lopen tegen heel veel dingen aan, en tijdens corona kwam dat nog eens extra naar voren, dat die begeleiders zich ook heel onzeker gingen voelen omdat ze gewoon niet goed wisten wanneer ze moesten handelen, wanneer ze hulp in moesten roepen, ja, wanneer een cliënt nou echt ziek was of alleen maar een beetje verkouden en hoe ze daar mee om moesten gaan. Dus daar zit een achterliggend probleem, dus nu willen we graag in kaart gaan brengen, van nou welke vaardigheden en kennis rondom gezondheid missen die begeleiders nu omdat ze een sociaal-pedagogische achtergrond hebben. En, nou dat sloeg heel erg aan, van ja dat is inderdaad ons probleem, terwijl als je meteen op dat diabetes was gaan zitten, ja dan had je een symptoompje opgelost maar niet het probleem gevonden. Dus daar helpt heel erg die systeembenadering van mij bij. Maar hoe we dat dan ook in de oplossing gaan doen, we gaan natuurlijk niet alleen maar aan begeleiders vragen van, nou, welke kennis missen jullie nu zoal in de praktijk, want ja, ze weten natuurlijk niet wat ze missen als ze het niet hebben of zo, weet je, dus we willen dat ook weten van artsen, we willen dat ook weten van verwanten van mensen met een verstandelijke beperking, ja, waar loop je nou tegenaan in de praktijk, welk stukje mis je, want die begeleiders hoeven ook geen doktersassistenten te [...], dat is helemaal hun doel niet, maar blijktbaar is er een klein stukje kennis wat ze misten om die goede zorg te leveren, en eigenlijk wil je dat ook weten van mensen met een verstandelijke beperking zelf, wat vind jij nou belangrijk dat anderen weten over jouw gezondheid. Dus dan op die manier pak je het, probeer je toch weer dat als een complex geheel, een dynamisch geheel te zien, van wat speelt er nou allemaal in, en daar zullen uiteindelijk dus ook bouwstenen naar voren komen hopelijk.

**MG:** Ja.

**P2:** Dat is het project wat nu start. Ook welke kennisonderdelen kunnen relevant zijn. En als je, en daar gaan we dan ook niet meteen weer een poster van maken of een interventie, wat subsidieverstrekkers ook allemaal graag willen, weet je dan, oh dan heb je bouwstenen, maak je daar een infographic van of, weet ik veel wat, en dan ga je dat implementeren, maar de bedoeling is juist dat iedereen op zijn eigen manier dat in gaat zetten voor een scholing. Dus in Nederland kan dat iets heel anders betekenen als in een ander land, of in, misschien wil je dat in een HBO-opleiding een plek geven, misschien ook wel in een MBO-opleiding, en misschien ook nog wel weer in een universitaire opleiding, dat moet iedere, dat, die mensen kunnen dat allemaal zelf veel beter, dat wiel hoeven wij niet uit te vinden, maar we willen wel

graag die aandachtspunten aanleveren. Dus dat is ook echt wel een andere manier van denken over, hoe ga je een probleem uit de praktijk aanvliezen. En het zit dus, ja op heel veel verschillende niveaus van hoe het zit nu.

**MG:** En speelt interdisciplinariteit daar ook nog een rol in?

**P2:** Nou, in die zin dat je die dagelijks begeleiders die hebben dus een sociaal-pedagogische achtergrond, die zullen dus andere dingen aanvragen als wanneer we met artsen gaan praten over, wat zouden dagelijks begeleiders eigenlijk moeten weten over die gezondheid. En die komen ook weer met heel andere voorbeelden, van waar zij in de praktijk tegenaan zijn gelopen, dat is waar die begeleiders mee komen. En, ja, dus in die zin speelt dat daar zeker een rol in, dus je wil eigenlijk in je vraagstelling daar al ruimte voor creëren dat je die verschillende perspectieven mee gaat nemen. En het andere bijeffect is hopelijk ook dat we daarmee ook onderling begrip gaan creëren tussen die disciplines, waar nu best wel af en toe wrijving ook zit hoor, tussen, ja dat artsen zoiets hebben van ja waarom weten die begeleiders dat niet, en die begeleiders die voelen zich continu maar overvraagd, en we moeten altijd alles checken, dus daar zit ook wel wat onbegrip, dus wellicht dat dat ook nog een plek [...] daarin vindt. Ja en in het onderzoek is het dus ook belangrijk dat die verschillende disciplines betrokken zijn. Ja en dan is het ook al weer lastig van, wat noem je dan een discipline hè, maar dus ook dat er niet alleen onderzoekers bij de uitvoer betrokken zijn, maar ook artsen en ook begeleiders zelf. Ja.

**MG:** Ja, ik noemde net dat woord complexiteitstechnieken, maar dat sloot volgens mij niet helemaal aan bij hoe u het zelf zou noemen. Waar zat dat in?

**P2:** Ja, ik denk in het technieken, dat, dan denk ik al meteen aan iets wat je heel concreet kan volgen of zo, of kan uitvoeren, dan zit ik ook toch wel wat meer ook aan die, aan, dan denk ik meteen ook wel aan statistische analyses, ja. Dus daar zit voor mij ook nog altijd wel een beetje een schemergebied hoor, in het complexiteit, omdat ik vanuit een heel sociaalwetenschappelijke kant altijd aan ben gevlogen en niet zozeer een heel technische kant.

**MG:** Ja. Want hoe zou u het zelf noemen, in plaats van complexiteitstechnieken?

**P2:** Ja, ik denk dat het voor mij meer een systems thinking toolset of zo, weet ook niet of dat een goed woord is. En ik denk dat het ook af en toe echt wel heel andere dingen beschrijft. Dus er zitten zelfde uitgangspunten achter, maar dat het ook echt wel in de praktijk dan wel over echt andere dingen kan gaan.

**MG:** Op wat voor manier dan bijvoorbeeld?

**P2:** Ja als je het heel technisch aanvliegt dan is het ook van nou, hoe ga je nou die complexiteit een plek geven in je analyse, in je modellen, hoe maak je je statistische modellen eigenlijk beter passend, hè, bij die complexiteit waar je het over hebt, en ik zit meer van oh, hoe ga je nou naar een probleem kijken op een, vanuit een complexiteitsperspectief. Je ziet dat in de literatuur ook wel terug hoor, dat daar verschillende stromingen in zijn, één is [...] wel een wiskundig of computational benadering, en een meer sociale – nou ja sociaalwetenschappelijk kan trouwens ook nog steeds best wel heel computational zijn, dus

daar zit het hem ook niet in. Ja ik zoek daar zelf ook nog heel erg naar hoor. Ja. Valt misschien meer in de, innovatieperspectief, dat is het misschien ook wel, daar zie je wel meer naar het beschrijvende terug.

**MG:** Ja. Ja, ik ben wel door mijn vragen heen denk ik, wat mij betreft zijn we ongeveer bij het einde.

**P2:** Oké.

**MG:** Ik weet niet of u nog iets zou willen toevoegen in dit kader wat nog niet ter sprake is gekomen, wat u denkt dat relevant is?

**P2:** Nee, ik zou het zo niet weten, nee. Ik hoop dat je een beetje verder kan hiermee.

**MG:** Ik heb heel veel informatie, ja, absoluut hoor.

**P2:** Nou gelukkig.

**MG:** Dan zet ik de opname even uit.

**P2:** Ja.

### **Participant 3**

**MG:** Yes. Nog even voor we beginnen iets over de verwerking van de data en dergelijke. Ik ga dit interview dus transcriberen straks en die transcripten en de opnames ook die ga ik allemaal bewaren, maar die zijn alleen toegankelijk voor mijzelf en voor mijn supervisors. In het eindproduct uiteindelijk kan ik alle data zo verwerken dat die geanonimiseerd is en niet tot u te herleiden valt, maar als u daar akkoord mee gaat zou ik als dat relevant is ook wel willen verwijzen naar uw naam en uw achtergrond in de tekst. Is dat akkoord?

**P3:** Akkoord.

**MG:** Super. Oké, als u verder heeft dan kunnen we beginnen wat mij betreft.

**P3:** Ja, prima, geen vragen.

**MG:** Goed. Oké. Nou ja, misschien als korte introductie even iets over uw onderzoek in het algemeen. Dus als u nou aan een wetenschappelijk opgeleide collega die geen achtergrond heeft in de psychologie, orthopedagogiek, zou moeten beschrijven waar uw onderzoek over gaat, wat zou u tegen zo'n iemand zeggen?

**P3:** Dat is een goeie altijd, ik ben niet zo goed in elevator pitches. Maar, ja, wat ik, waar ik me nu vooral mee bezig houd zijn inderdaad van die tipping points of kantelpunten in klinische verandertrajecten, dus wat gebeurt er met mensen die in behandeling zijn, en waar ik me de laatste tijd veel op richt zijn inderdaad die grote sprongen, kwalitatieve sprongen, dus dat je ziet dat het ineens veel beter gaat met iemand of veel slechter, of die heeft een terugval in drugs, middelenmisbruik, en ja, wat, dat we dus met Merlijn ook gevonden hebben, dat je dat soort kwalitatieve sprongen die zie je aankomen van te voren, als je kijkt naar de fluctuaties in het, binnen de cliënt, in bijvoorbeeld zelfbeoordelingen over hoe het gaat, en dus waar ik me nu op richt is, oké wat kunnen we nou, kunnen we daar meer zicht op krijgen wat eigenlijk de onderliggende factoren zijn, die een systeem naar zo'n tipping point brengen, en daar denk ik dat het in de, maar dat is nog een open vraag, dat het in ons veld zou het dan kunnen zijn, dus als je weer, ik denk aan die behandelcontext, kan het zijn dat een cliënt of een patiënt ineens veel meer hoop krijgt, of dat die, maar ook dat die verliefd wordt ineens, of zo, of dat die eindelijk een goeie relatie, goeie klik heeft met zijn behandelaar, dus dat dat soort van factoren kunnen zijn die zorgen dat een cliënt in beweging komt. En het laatste waar ik me dan nog op wil richten is om te kijken, oké, als we dan dat soort fases kunnen identificeren waar we zien, oh ja, een cliënt komt in beweging, of dan interventies mogelijk ook het relatief gezien meer effectiviteit hebben dan in fases waarin een cliënt heel erg stabiel is. Dus dat is een beetje [...] voor leken, geïnformeerde leken.

**MG:** Ja. Oké. Ja, en ik heb begrepen dat u werkt vanuit het perspectief van complexiteitstheorie, klopt dat?

**P3:** Ja. Ja. Ik heb het toen nog, toen ik mijn PhD-project deed noemden we het altijd non-lineaire dynamische systeemtheorie, ik weet nooit zo heel goed waar, wat, nou ja, wat nou daar de verschillen tussen zijn, maar inderdaad, vanuit dat perspectief, ja.



**MG:** Ja, dus als we daar even wat verder naar gaan kijken, want complexiteit is natuurlijk een ontzettend breed begrip wat door heel veel verschillende mensen ontzettend verschillend wordt opgevat.

**P3:** Precies.

**MG:** Wat is nou vanuit uw achtergrond en uw onderzoek de betekenis van complexiteit?

**P3:** Ja, ja. Dus complexiteit zit hem niet in de hoeveelheid variabelen, of zo, maar, nou ja, hoe ik hem denk ik aanvlieg is dat we, ja, dat ook al weten we hoe de onderliggende relaties zijn dat we toch niet kunnen voorspellen wat de uitkomst van het proces zal zijn. Dat denk ik, zo zou ik het denk ik beschrijven.

**MG:** Ja. Is dat het enige of is er nog meer aan?

**P3:** Hm, nou dat vind ik het belangrijkste, om het ook af te zetten van complicated of zo, of hoeveelheid in termen van oh dit is zo complex omdat daar heel veel variabelen meespelen, dat is voor mij niet de kern van complexity. En ook niet of het nou, want dat kan ook een heel simpel systeem zijn wat toch complex gedrag laat zien. Dus ja, ik denk dat ik daar toch bij blijf, dat ik dat de belangrijkste kern vind.

**MG:** Ja. En merkt u wel eens verschillen tussen hoe u complexiteit opvat tegenover hoe anderen dat doen?

**P3:** Oh ja zeker, zeker, dat denk ik wel. En ik merk in elk geval in de gedragswetenschappen of de, ja, de sociale, dus mijn veld, dat het heel erg een buzzword geworden is, dus dat iedereen eigenlijk een beetje iets met complexity ervoor zet omdat het nu heel erg hip is, en ja. Dus nee, ik merk daar zeker verschillende definities of dat ik denk van ja, maar volgens mij heeft dit niet zo heel veel met complexiteit te maken, of precies wat ik zeg, dat mensen zeggen van ja, het is allemaal zo complex want hier spelen zoveel variabelen mee waar ik denk van ja, maar, nou ja. Dat soort mis, volgens mij, misconcepties zie ik wel best veel, ja.

**MG:** Heeft u daar nog meer voorbeelden van, van dat soort?

**P3:** Nou ja, wat voor mij eigenlijk ook, maar dat weet ik niet precies of ik dat echt onder complexity of adaptive complex systems zou zetten, nou ja ik vind die, dat tijdselement, dus dat het gaat om het bestuderen van het systeem over tijd, en ook met die interactie met de omgeving wat die ook maar mag zijn, dat ik daar zie ik dus ook veel benadering waar ik denk van ja, maar jullie kijken helemaal niet over tijd of zo, dus dan kan het voor mij al per definitie niet om een echte adaptive complex system approach gaan. Dus dat, dat vind ik. Dus ik, als iemand cross-sectioneel over mensen heen, bijvoorbeeld, weet ik veel, symptoomnetwerken bestudeert, dat heeft voor mij niks te maken met complexity.

**MG:** En waarom is dat tijdselement dan zo belangrijk?

**P3:** Dat is een goeie, ja. Nou ja dat is dan, ja, dat, nou ja het is een goeie, en ik, wat ik zeg, ik kom dus meer uit het non-linear dynamic systems, en daar zit dat dynamic, dus dat je de evolutie van het systeem over tijd bestudeert, zit daar heel nadrukkelijk in, en ik ben van oorsprong developmental scientist, dus voor mij is sowieso als je iets niet over tijd bekijkt,

zeg maar, kun je daar weinig, nou ja het kan een snapshot zijn, maar als je echt wilt begrijpen hoe het systeem geëvolueerd is tot die toestand of hoe het zich in de toekomst gaat gedragen, ja, dan is, dan heb je toch altijd een tijdselement daarbij nodig, en niet statische associaties tussen variabelen. Dus, ja, dus als je me nu zo vraagt, is dat nou echt over de complexity, of zit dat toch meer in de non-linear dynamic systems, dat weet ik niet. Dat weet ik niet.

**MG:** En hoe groot is op dit moment, zou u zeggen, de rol van dat begrip complexiteit in het onderzoek dat u nu doet?

**P3:** Ja, ik zie dat dat daar enorm hip is, wat ik zeg, dat dat daar, je hebt natuurlijk ook die, weet niet in hoeverre je dat wel of niet kent, maar in die hele network-benadering, inmiddels zijn ze dat network theory gaan noemen, ik denk dat het een benadering is en dat, ik vind het conceptueel vind ik het heel erg interessant, of, zeg maar, zeven jaar geleden of zo toen het voor het eerst opkwam in ons veld, vond ik dat conceptueel heel interessant en stimulerend, en het heeft ook zeker een goeie invloed gehad op het veld, dat er namelijk nu toch een beetje een verandering is gekomen, maar daar zie je ook, daar wordt nu overal voor die netwerken wordt gewoon complexity gestopt, en ja ik denk, dat weet ik eigenlijk niet zo goed. En je ziet natuurlijk ook het early warnings onderzoek, nou ja, wat wij ook gedaan hebben, dat zie je ook enorm hip is dat aan het worden, hangt ook samen met dat just-in-time interventions, dus kun je, want voorheen hebben we in ons veld vooral gekeken welke interventies werken nou het beste, maar het wordt dus steeds ook interessanter en het besef komt steeds meer, ja misschien maakt het ook nog uit wanneer we die interventie geven. En daar zie je wel, plus dat je ook ziet dat het one size fits all, daar weten we inmiddels ook, dus ik denk er komen een aantal dingen samen, dat het veld met het onderzoeks of met de benaderingen, weet je, groepsbenadering, voor nameting, randomised controlled trials, dat daar duidelijk is van hier stoten we op een limiet, we komen hier niet verder, en tegelijkertijd zijn er genoeg, is de kritische massa wel een beetje bereikt die bezig is met dat soort ideeën, dus en dan dat soort ideeën bedoel ik dus non-linear dynamic systems, complexity, maar ook die netwerkbenadering, ja, die kritische massa is een beetje bereikt zodat het nu ook een beetje dat mainstream bereikt. En dat heeft heel veel voordelen, maar het heeft, soms is het ook een beetje nou ja wat ik zei, wordt het zo'n buzzword en wordt het dan gebruikt door mensen waar je denkt van, is dit nou echt ook dit.

**MG:** Ja.

**P3:** Dat je bijvoorbeeld early warnings of zo, ja, dat moet je wel binnen een individu over tijd bekijken, dat kun je niet in een cross-sectioneel onderzoeksdesign, dus dat zijn dan zo dingen waar ik denk van hm, hm, is dit nou, ja, ja.

**MG:** Ja. Ja en als u nou kijkt naar de methode die u dan gebruikt binnen dit idee van complexiteit, als u nou eens denkt aan een lijn of project waar u de afgelopen jaren aan gewerkt heeft, wat voor concrete onderzoeksmethoden heeft u toen gebruikt?

**P3:** En met methode bedoel je dan de analysetechniek, of meer de design, of?

**MG:** Het geheel eigenlijk, van hoe je bij een, van een onderzoeksvraag naar het antwoord komt.

**P3:** Ja. Ja. Nou ja, en daar denk ik, daar zijn verschillende, op verschillende niveaus heeft dat, die manier van denken zeg maar een invloed. Dus het begint natuurlijk al bij de onderzoeksvragen, dat je anders überhaupt niet zo'n vraag zou stellen, als je niet vanuit dat kader zou denken, je zou niet op zoek gaan naar early warnings als je niet het idee van phase transition en hé, destabilisatie en zo, dan zou je op zo'n vraag nooit komen. Dus dat is het ene. Aan de andere kant, en, dan weet ik ook, zeker als ik naar mijn eigen werk kijk, dat daar natuurlijk ook een verandering is gekomen in het eerst best wel metaforisch gebruiken, versus het ook echt methodologisch en analytisch zo aanpakken, en dat heeft er ook mee te maken dat we nu door allerlei technologische, smart phones en dat soort dingen, dat soort type data kunnen verzamelen überhaupt, die zo fijnmazig zijn, en dat een aantal van die toolbox, ja, nu het ook mogelijk maakt om toch nog want, ja, jullie lachen altijd een beetje over onze, dat vinden wij het al hele lange tijdseries, nou ja, die zijn, het is niet heel erg lang, dus dat er nu ook steeds meer methodes beschikbaar worden voor de type data die wij hebben, en dat was zeker tien, twintig jaar geleden nog niet per se zo. Nou ja, en dus, anderzijds kan het ook de design beïnvloeden, dat je bijvoorbeeld, weet ik veel, een mooi voorbeeld is altijd het onderzoek van een collega van mij waar ze met perturbation gewerkt hebben, dus dat je, moeder-kindinteracties die laat je dan praten over bijvoorbeeld een conflict, en dat je dan zegt van nou ja, dan gaan we op een gegeven moment aan de deur kloppen en zeggen van hé, nu heb je nog een minuut dan moet je afronden, en het hele idee daarachter was van oké, we zien of een, hoeveel toestanden een systeem kent als we het even onder druk zetten, en, dus dat is, nou ja, dat is een design choice die komt uit het denken van, ja, die multistability, die krijgen we pas te zien als we ook iets doen. En dan zijn natuurlijk de analysetechnieken, en daar werk ik heel veel samen met Fred, die, nou ja, dat heb je zelf gezien, die daar een hele toolkit beschikbaar heeft, dus de RQA vind ik zelf ook een fijne, omdat die, omdat het heel dicht bij de data blijft, en ik denk ons algemeen principe is een beetje analyse first and then aggregate, dus dat we toch proberen een eerst binnen dat ene systeem te kijken wat zien we, en dan pas over cases heen, en dat ik eigenlijk meer en meer denk van, hm, die hele ingewikkelde statistische modellen en zo, ik weet het niet, omdat we toch ook wat we met Merlijn hebben laten zien, dat je toch al die assumpties eigenlijk, ja, vaak schendt met het type, als je data echt van een complex systeem gegenereerd zijn. Dus dat is problematisch. En bij mij komt er dan nog bij, dat ik denk, voor, omdat ik het ook belangrijk vind dat het werk wat ik doe ook direct, hoe zeg je dat, toepasmogelijkheden heeft in de praktijk, en ja, daar kun je dus eigenlijk ook niks met die statistische modellen waar je eerst alles verzameld moet hebben en dan vervolgens je analyses, dus ik wil eigenlijk veel meer toe naar on the fly, in, en ja, dan gaat het over een complexity algoritme die je daaroverheen schuift en kijkt van nou ja, schiet die nou ineens heel erg uit de bocht en moeten we misschien iets doen of zo. Ik zeg niet dat dat het alleen maar is, maar ik, hm, ja ik heb toch zo mijn vragen bij de ingewikkelde statistische modellen, waar ik dan denk van ja, weten we eigenlijk al überhaupt genoeg over de nature of the system voordat we dat soort assumpties allemaal kunnen aannemen en ingewikkelde modellen op loslaten.

**MG:** Ja. Ja, u moet maar een beetje vergeten dat ik dat vak gevolgd heb hoor, want ik ben gewoon benieuwd...

**P3:** Jajaja...

**MG:** ...wat u daarover zegt.

**P3:** ...dat, ja, ja. Nee, dus qua analysemethodes denk ik dus dat, nou ja die Recurrence Quantification Analysis vind ik een hele mooie. Ik heb tot nu toe alleen maar ermee gewerkt met categorische data, dus waar natuurlijk dan heb je die hele faseruimteconstructie niet en zo. Ik vind ook, ik weet niet of je daar ook van gehoord hebt, de state space grid methodologie, dat [...] we ooit mee gewerkt, dat is bedacht door Marc Lewis en dan Tom Hollenstein, en dat is heel erg voor psychologen, het is heel erg simpel, maar het gaat wel uit van die ruimte, dat die twee dimensioneel, en dat je dus volgt waar het systeem zich in, nou ja, welke gebieden het bezoekt en hoe lang het daarin blijft hangen, als het dan weer weggaat hoe snel dat weer terugkomt en dat soort, dus een beetje dat attractorenlandschap, daarop is het gebaseerd. Het is dan helaas heel vaak niet op die manier ingezet, maar ik hou in het algemeen wel van analysemethodes die me dicht bij de data houden, dus waar ik eigenlijk nog kan zien wat er gebeurt, in plaats van dat het heel erg ver weg daarvan is. Dus zo denk ik dat, ja, dat er best wel wat... En überhaupt in het algemeen denk ik, ja, moet je altijd af, uitgaan van wat is nou mijn onderzoeksvraag en welke methode past daar nou het beste bij. Ik ben persoonlijk niet zo iemand van, nou ja, ik heb dan bepaald stokpaardje en dat pas je op alles, dan heb je je methode en zoek je dan vervolgens vragen die passen bij de methode, daar ben ik niet zo voorstander van, dus ik, ja, graag, dat is op mijn eigen opleiding, mijn promotor, die was dus een pionier in het veld van developmental science en dynamische systeemtheorie en die, ja, die heeft me dat heel erg bijgebracht, van je hebt een vraag en dat is leidend, en dan gaan we wel iets verzinnen hoe we daar een antwoord op kunnen geven. Ja. Dus. Zo.

**MG:** En wat zijn nou de belangrijkste verschillen tussen de methodes die u gebruikt en de meer standaard statistische methodes, zeg?

**P3:** Mhm, Mhm. Ja, pfoe, wat zijn de belangrijkste verschillen. Nou ja, ik denk dat de aannames heel erg anders zijn. Dus dat je, dat, nou ja wat ik zei, dat zo'n RQA is natuurlijk, ja, is niet toetsend, is heel beschrijvend, dus je krijgt er wat waardes uit, die kun je dan vervolgens natuurlijk weer gebruiken om in een model te gooien, in een regressie of wat dan ook. En daar is daar ook niks mis mee hè, ik denk dat het ook prima is voor bepaalde vraagstellingen bepaalde methodes te gebruiken, maar ik denk, ja, ik denk dus dat het belangrijkste verschil is eerder die, wat ik al zei, analyse first and then aggregate, dus in principe laten we uitgaan van de case, en die over, nou ja, als we meerdere cases hebben dan zoeken naar wetmatigheden in plaats van alles op één hoop gooien en dan de verbanden zoeken. Dus dat, dus het n is één achtige, het over tijd, tijdseriële, en dan het liefst, nou ja, zoeken dat, want dat, nou goed, dat is niet per se analyse, is ook een beetje design issue, dat er vaak bij ons in het veld helemaal niet over nagedacht wordt, wat is nou eigenlijk de natuurlijke fluctuatie van het fenomeen wat we onderzoeken en laten we onze meetfrequentie daarop aanpassen. Het is altijd standaard één keer per jaar of zo, dan denk je,

hoezo? Dan wordt er emoties gemeten, wie zegt nou dat die... Nou ja dus dat het eigenlijk de meetfrequentie moet passen bij het fenomeen wat je onderzoekt, en dan over tijd, en dat ik, ja, dat ik ook denk dat ik, wat ik net al zei, dat ik wat voorzichtig terughoudend ben met die hele ingewikkelde statistische modellen omdat ik denk dat dus heel veel aannames problematisch zijn, gezien de nature of the data die we hebben.

**MG:** Ja. En hoe bent u er zelf ooit bij gekomen om nou deze methodes te gaan toepassen in plaats van wat meer gangbaar is?

**P3:** Nou ja, dat was dus, daar was ik, denk in mijn derde jaar of zo, in Groningen, ontwikkelingspsychologie, en dacht ik toen al een beetje, is dit het nou echt? Zo. Zeker natuurlijk als je vanuit de ontwikkelingspsychologie, waar het dus gaat om de ontwikkeling van de mens, dat ik het toen al best wel teleurstellend vond, dat ik dacht van ja, we hebben hier een groepje van vierjarigen en tienjarigen en twintigjaren, maar dat gaat toch niet over ontwikkeling. Dus ik voelde wel bij mezelf een teleurstelling over, ik vond de theorievakken altijd superinteressant, en het conceptuele, maar zag best wel mismatch tussen de theorie en het fenomenologische, en eigenlijk de benadering daarvan, hoe het dan in onderzoek qua methodes en design en zo benaderd werd. En toen had ik een vak van Paul van Geert, die, ja, dat was echt een eye opener voor mij, want die begon dus met de, ons de dynamische systeemtheorie uit te leggen, en, nou ja, hij heeft heel veel gedaan op het gebied van cognitieve en taalontwikkeling, en was dus ook met het computational modelleren bezig, supersimpel, maar ja, dat sprak mij heel erg aan, omdat dat dacht ik, ja, nu gaat het ergens over, nu proberen we echt de mechanismen te begrijpen, nu gaan we echt naar het proces kijken, en, ja. Dus ik had meteen het gevoel, dit past veel beter bij het fenomeen zoals het is in plaats van die hele statische grote groepen benadering, die eigenlijk niet goed matcht met het fenomeen. Ja, en toen ben ik, toen heb ik mijn masterproject bij hem gedaan, en toen kreeg ik de mogelijkheid om daar te promoveren, op eigen, op interne onderzoeksgelden, dus dat gaf mij heel erg de mogelijkheid om te doen wat ik zelf wou. Ja. En toen heb ik het wel een tijdje na mijn, want het verkocht in die tijd nog niet heel goed, die dynamische systeem ideeën, in het psychologieland, dus we moesten altijd heel erg ons best doen bij het schrijven van artikelen, en heel erg verantwoorden waarom we nou, we hebben toen ook veel Monte Carlo dingen gedaan, hè, dat helemaal niet zo heel erg fancy, maar toen was dat echt nog niet dat het snel zoiets, dus je moet altijd superveel extra uitleg geven waar ik dacht, van, waarom hoeven die anderen dat niet. Nou ja, en het verkocht allemaal wat minder goed, dus dat is nu heel anders bij als ik kijk naar Merlijn, hoe het ene naar het andere artikel gepubliceerd wordt. En toen ben ik ook een hele tijd, toen ben ik dus naar Nijmegen gekomen, en bij orthopedagogiek, en toen veel interventieonderzoek, wat me heel erg aansprak, omdat ik dacht, oh ja, ik ben nog steeds geïnteresseerd in de ontwikkeling, maar nu zie ik ontwikkeling op een heel veel kortere tijdschaal, ik hoef niet meer jarenlang te wachten voordat iets gebeurt maar het gebeurt in korte tijd, maar toen was ik heel erg teleurgesteld toen ik dat veld ontdekte, want ik dacht, wat, daar wordt helemaal niet naar processen gekeken, er is een voor en een nameting en, op groepsniveau. Maar toen ben ik het dus een tijdje heb ik, was ik daar niet zo heel veel mee bezig en heb ik meer geleerd hoe het, zeg maar het conventionele spel van de wetenschap te spelen, wat ook heel leerzaam was. Maar ik heb het eigenlijk pas dan, zo, ik denk, zes zeven jaar geleden, weer echt heel

actief opgepikt, en gedacht van nee, dit slaat, dit heeft ook in dit, deze discipline heel veel kracht, en, nou ja, en wat ik zei, en dan toen kwamen een beetje dingen bij elkaar, dat het veld in beweging kwam, dat er meer mensen vanuit die hoek, en, nou ja, komt alles een beetje bij elkaar. En dan krijg je ineens een Vidi, wat je nooit eerder voor mogelijk had gehouden. Ja.

**MG:** Ja. En hoe denkt u dat dat kwam, dat dat veld toen in één keer wat meer uw kant op is bewogen?

**P3:** Nou ja, dat is wat ik zeg, dat ik denk dat dat het algemeen wel, een voorbeeld, we zien dat in, sinds decennia, vijf decennia of zo, zien we eigenlijk die effect sizes, dus we weten met al die psychologische behandelingen zijn die effect sizes moderate. Wij hebben ongeveer altijd vijftig proces die niet aan, die niet positief reageren op een behandeling. Varieert een beetje per type stoornis en type behandeling, maar zo over het algemeen is dat een beetje het beeld. En sinds vijf decennia is daar niks aan veranderd. Heel veel onderzoek, bakken met geld naartoe gegaan, maar is niks aan veranderd. En, dus er komt nu toch een beetje het bewustzijn van nou ja, misschien moeten we ook A, ander type onderzoek doen, maar B ook heel erg anders nadenken over interventies, dus dit heeft weer ermee te maken dat het ook natuurlijk bij conceptueel niveau al begint, want als we kijken hoe er over interventies na wordt gedacht, dat is nog steeds die hele evidence based movement, nog steeds heel erg geïnformeerd vanuit, dat er is een soort van silver bullet, hè, dus die, dat is de pil, en die geef ik jou en dan ben je af van je depressie. En dat strookt niet met een complexity benadering, dat natuurlijk nooit je kunt verwachten dat voor iedereen, A, dat de effect force alleen maar in die interventie zit, en B, dat dan ook het effect voor iedereen hetzelfde is, dat... En, dus ik denk dat de feiten voor zich spraken, dat mensen, ook zelfs de hardline RCT mensen, toch moesten toegeven, ja, oké, we komen hier niet echt verder. Hetzelfde geldt een beetje voor de, zeg maar de oorzaak van psychopathologiën, ook daar is heel veel geld gegaan in genetica en heel veel geld in neuro, dat was tijden heel erg hip. Ook daar hebben we geen grote doorbraak gehad. Dus ik denk dat zo, hm hm hm, op een aantal fronten dat een beetje de evidence cumuleerde en zo van, oké, hier komen we toch niet echt verder. En tegelijkertijd genoeg mensen al iets gehoord hadden over of het nou via de ecologie of via, nou ja de natuurkunde of weet ik het waar vandaan, maar dat er steeds meer mensen waren die daar al van gehoord hadden en ook samenkomend met, nou ja wat ik al zei, met die technologie, dus dat het ook meer mogelijk werd om dat soort type data te verzamelen die je daarvoor nodig hebt, ja, dat dat een beetje een momentum gecreëerd heeft, waardoor het nou, ja, ineens wel. En nou ja, nu moeten we het waarmaken ook, dat moeten we nog maar even zien. Want ja, dat is denk ik, dat is een beetje de gevaar natuurlijk, dat het, ja, intuïtief sluit het heel goed aan bij mensen, ook als ik bijvoorbeeld met professionals, dus met therapeuten of zo praat, ja, weet je, als ik dan zeg ja, het systeem moet in beweging en komen dat [...]. Dus het is, het, intuïtief sluit het heel goed aan bij mensen, maar we moeten het nog wel zien denk ik en we moeten het ook nog wel zien in hoeverre al die metaforen die we dan gebruiken uit de natuurkunde dan bijvoorbeeld of die ook echt passen voor ons, en of het nou echt allemaal hetzelfde werkt, en zo, dus, dat vind ik bijvoorbeeld een hele interessante zelf ook van die RICH, heel erg leuk vinden om het daar wat meer over te hebben, waar zitten nou misschien ook de verschillen tussen, hè. Dus dat, ja dat vind ik belangrijk. En dat het dus niet blijft staan,

en blijft hangen in zo'n hele populaire, oh ja, ja ja, we weten wel en precies complex, weten we, het is allemaal heel ingewikkeld, en nou ja, dat is een beetje de dunne [...] denk ik, waar je je goed in moet bewegen, dat het natuurlijk, dat je gebruik moet maken dat het intuïtief aansluit bij mensen, maar dat je toch zorgvuldig moet zijn en ook met de claims en zo, dat het niet zo'n, ja.

**MG:** Ja. Ja, want als we nou eens teruggaan naar de technieken en ideeën die u gebruikt, want u noemde net al natuurkunde bijvoorbeeld, of ecologie. Wat voor soort ideeën of technieken gebruikt u die niet oorspronkelijk uit de psychologie zijn ontstaan?

**P3:** Nou ja, ik denk dat de RQA niet oorspronkelijk in de psychologie is ontstaan, ook andere tijdseriële analyses, die we gebruikt hebben om bijvoorbeeld de predictive horizon en dat soort dingen, of de butterfly effect, en, die zijn echt niet altijd psychologie, en daar zie ik ook nog trouwens grote problemen dat we die hebben we nu toegepast bij een dataset, ja, die heeft bijna tienduizend datapunten, ja, dat zie ik niet gebeuren dat dat in de dagelijkse praktijk verzameld wordt. En, nou ja, en die ideeën, ja dat is een goeie, want op zich denk ik, dat idee van een phase transition hè, wat eigenlijk een beetje een soort van rode draad door mijn hele wetenschappelijke, want mijn PhD-project ging over identiteitsontwikkeling en moeder-kindconflicten en zo, maar ook geframed vanuit, oké, die adolescentiefase is eigenlijk een soort van fase transitie, ja, daar kun je natuurlijk zeggen nee, dat is echt iets uit de natuurkunde. Ja, maar ik zie, je ziet het best wel ook terug al in vroeger psychologisch werk, of als ik bijvoorbeeld kijk naar de psychotherapieliteratuur en zo, hebben die het, ja, dan hebben ze het misschien niet zo expliciet geframed in die termen, maar ik denk dat in die tijd sowieso natuurlijk meer nog, zeg maar een soort van, en nu leiden we heel erg vakidioten op, om het zo maar te zeggen, dus die zich heel erg op één ding alleen maar focussen, en dat vroeger het veel gebruikelijker was om breed, breder in elk geval op te leiden, dus met een beetje filosofie, met een beetje natuurkunde ook, met een beetje psychologie, ik zeg maar wat. Maar, dus in elk geval zie ik daar wel dat soort ideeën ook al in terug, en dan zijn ze natuurlijk nooit empirisch onderzocht, maar dan zijn dat soort concepten van nou ja, een cliënt die vastgelopen is die moet eerst oude patronen doorbreken om überhaupt de ruimte te hebben om iets nieuws te exploreren, of zo. Ja, dat zie je daar ook wel in terug. Ja. Dus ik vind het, en daar zit ik te weinig goed verankerd in de hele historie zeg maar, om goed te kunnen zeg- want, ik heb toen altijd ook wel psychologische literatuur gevonden die over dat soort concepten sprak, zeker als je kijkt naar het werk van Thelen en Smith, die weet ik niet of je die kent, maar dat zijn dus ook developmental scientists die heel erg met de motorische ontwikkeling van kinderen zich beziggehouden hebben, en dat is een beetje dezelfde generatie als mijn promotor ook was, Paul van Geert, dus dat waren zo de eerste adopters van die ideeën en eerste pogingen om het om te zetten. Maar ik zou ook niet, ik vind dat Piaget heeft ook best wel wat dynamische ideeën, of Kurt Lewin, ja, dus ik, dat vind ik een beetje een lastige te zeggen welke, voor mij is het zeker ook uit de natuurkunde en zo is het mij ook altijd bijgebracht, zeg maar, maar ik zie wel in elk geval in termen van theorieën en concepten ook al echt vroeger werk, en dan heb ik het over de jaren dertig, veertig, vijftig, waar dat soort ideeën, en dan niet empirisch omgezet maar dat zo dat soort ideeën er wel speelden ook wel in de psychologie.

**MG:** En op wat voor manier integreert u dan zo'n concept als een fasetransitie, hoe zet u dat om in iets wat u kan gebruiken in uw onderzoek?

**P3:** Nou ja, ik probeer gewoon de gelijkenis te zoeken, dus wat is, dus een fasetransitie, nou ja, dat het moet gaan om een system wide qualitative reorganisatie die leidt tot een ander, kwalitatief andere toestand, en dat is denk ik iets wat je, ja, wat je voor een psychologisch systeem kunt uitleggen, maar ook voor een chemisch systeem of een fysisch systeem. Dus ja, dat gaat wel, en dan kan ik ook best wel relateren aan, oké, als ik naar het, kijk naar de theorie van Haken over hoe die de laser beschrijft, en dan zie je dus die kritische fluctuaties, ja, oké, dan zouden we dus verwachten dat we dat, als we dagelijkse self ratings hebben van patiënten, dat we dat dan daarin terugzien. We weten niet precies hoe die vorm eruit ziet, wanneer ze hoe hoog moeten zijn, maar we weten in elk geval, kort daarvoor moet het veel hoger zijn dan heel ver weg van dat kantelpunt, bijvoorbeeld, en daarna verwachten we ook dat het omlaag gaat. Nou ja dus, zo kun je op zich, vind ik, ja, kun je daar best wel makkelijk relateren maar nogmaals, ik denk dat daar ook een gevaar in zit soms, dat je te snel denkt, van oh ja, dat is toch het, dat kunnen we nu zomaar toepassen of kunnen we nu zomaar relateren, terwijl het dan toch net niet is of zo. Dus ik zou daar, probeer nu, hoop nu, dat ik in Groningen heb ik nu de kans om een scholarship-student, dus een aio aan te nemen, maar die zit dan op zo'n beurs, een beursaal, en daar wil ik heel graag met het Bernoulli-instituut samenwerken, weet niet of je dat wat zegt, dat is dus natuurkunde en wiskunde [...], en ik ken daar toevallig één hoogleraar maar die is nu met emeritaat zag ik, maar ik zou dat ontzettend graag willen want ja, ik ben ook maar een psycholoog, en heb wel wat literatuur gelezen, maar voel me natuurlijk, lang niet bekwaam genoeg om al die dingen goed te begrijpen. Aan de andere kant, natuurkundigen die hebben dan weer geen idee waar wij het over hebben, dus ik, ja, vind juist die interdisciplinaire samenwerking en toetsen bij elkaar, oké, dat bedoelen wij ermee, en dit is wat wij dan zouden verwachten, of, en, oké, hoe, dat zou ik ontzettend vruchtbaar vinden, omdat ik soms wel een beetje denk, we moeten wel oppassen dat we niet te simpel al die concepten nu zomaar naar ons vertalen, en... Ja.

**MG:** Ja. Want die interdisciplinaire samenwerkingen, is dat nu ook al onderdeel van wat u doet in uw onderzoek?

**P3:** Sorry, nu was de verbinding iets slechter, kun je het nog een keer zeggen?

**MG:** Sorry, ik zal het herhalen. Die interdisciplinaire samenwerkingen, is dat iets wat u nu ook al gebruikt in uw onderzoek?

**P3:** Ja, ja ja, dat denk ik wel, ik denk inderdaad dat het al, nou ja, interdisciplinair wordt op het moment dat je dus een beetje over je eigen disciplinerand heen kijkt en je laat informeren door, nou ja, natuurkunde of ecologie of wat dan ook. Ik zou het graag, nou ja, en ik, nogmaals, daar heb ik dus wel het grote geluk met Fred als samenwerkingspartner, dat die, ja, die is ook niet qua achtergrond niet, is die ook gewoon psycholoog, maar die vindt niks leuker dan zich in dat soort dingen te verdiepen, en dan daar ook over na te denken, oké, hoe kunnen we dat nou ook geschikt maken voor onze type data, en hè, die categorische RQA, ja dat hebben wij toen echt wel een beetje als eerste gedaan, want daarvoor was natuurlijk alleen maar op continue data, nou ja, was iets, een deel, maar hij is



daar heel slim in ook van, oké, dat is er, en zo heb ik er nog ook iemand waar ik graag en veel mee samenwerk, die ook een psycholoog is, maar wel gewoon een hele stevige methodologische poot, en, ja, en ook zelf graag over die randen heen kijkt. Nu zou ik, en nu hebben we voor het eerst in het project met, Jingmeng, ik weet niet of je die, ja...

**MG:** Ja.

**P3:** ...werken we daar samen, hij is zelf natuurlijk een beetje interdisciplinair, omdat hij chemistry eerst gedaan heeft, maar nu zit ook bij het project erbij professor Li, die echt van de wiskunde is, en dit vind ik eigenlijk, ja, dit vind ik het mooist, omdat je, ja, omdat je dan echt nog meer van elkaars expertise kan profiteren en echt goed toetsen bij elkaar, en, ja, ik weet, dat kan ik niet zo goed beoordelen of het de natuurkundigen of de wiskundigen ook iets oplevert, dat weet ik niet, maar ons levert het in elk geval zou het heel veel opleveren om, ja, wat ik al eerder zei, om daar goed na te gaan, oké, wat, waar denken we ook, daar kunnen we die concepten toepassen, op psychologisch veld, maar waar zitten misschien ook interessante verschillen en moeten we dus iets anders bedenken, of zo. Ja.

**MG:** Ja.

**P3:** Dat zou ik heel erg vruchtbaar vinden. En dan moet je denk ik, ja, dan moet je, de discipline en de background is één ding, maar je moet ook, ja, je moet elkaars taal een beetje praten. Dat lijkt me dan ook belangrijk ja.

**MG:** Ja. Ja, want hoe gaat dat bijvoorbeeld met die wiskundige professor dan?

**P3:** Ja, nou ja, eerlijk gezegd, soms denk ik, ik heb geen idee waar ze het over hebben. Nee, dat kan ik echt niet allemaal volgen. Ik kan het dan proberen conceptueel te volgen, en, nou ja, en dat doe ik ook en dat zie ik ook als mijn taak en de taak ook van Jingmeng dat die natuurlijk uiteindelijk wel onze research master doet, dus er moet echt in staat zijn om een research master thesis te schrijven die voor een geïnformeerde, maar toch voor iemand die niet per se een wiskundige achtergrond heeft te volgen is. En... Ja, en aan de andere kant is het dan ook een stukje van oké, nou ja dat is jouw expertise, dus ik ver-, daarom heb ik hem, dus die professor ook nodig, zodat hij dat deel kan checken, want ik zou dat niet kunnen doen. En daar denk ik ook ja, we hoeven ook geen, de illusie te hebben dat we allemaal superhelden zijn, dus wees ook eerlijk en transparant met elkaar van, oké, dit kan ik goed maar dit niet. En dan dat je in die zin samenwerkt. Dus ja, ik vind dat bij die wiskundigen en ook bij het project met Jingmeng, vind ik het wel een uitdaging, omdat dit, ik heb het gevoel we worden hier allen super beter van, maar het is wel, het is echt een beetje aan de edge van wat ik ook nog met mijn eigen achtergrond kan volgen, wat hij eigenlijk aan het doen is.

**MG:** En merkt u dat dat ook andersom geldt?

**P3:** Die psy-, of hij? Ja dat is een goeie, dat is een goeie... Dat weet ik niet zo goed omdat we hem veel minder zien, en dat heeft hem, is puur denk ik omdat die hij een heel, dus die hoogleraar, een heel busy schedule heeft, en wij al heel blij waren dat die dat wil doen. Jingmeng geeft ook aan, nou ja, Jingmeng is Chinees en hij ook, zij hebben dan eigenlijk die meetings ook liever samen in het Chinees. En wat dat betreft is het misschien ook zo dat die, maar dat weet ik niet. Maar, hm, laat ik het zo formuleren, het was van ons in elk geval een

uitgesproken wens om hem erbij te hebben, ik weet niet of hij ons had gekozen als een project. Dus ik denk dat het in zo'n interdisciplinaire samenwerking zou ik het ook heel fijn vinden als je een soort van gelijkwaardige samenwerking hebt, en niet alleen maar oké wij willen graag iets van jullie leren, maar dat ook vanuit de andere, de meer natuurkundige kant in elk geval interesse bestaat in de fenomenen die wij interessant vinden. Dan denk ik, dan kan het echt iets heel leuks opleveren waar je, ja, waar je allebei van, beter van wordt. Maar dat hoeft niet altijd zo te zijn, soms kan het natuurlijk ook zijn van, kun je even met ons meedenken en ons helpen. Maar mijn ultimate goal zou toch een beetje zijn dat je, nou ja, dat je ook dat soort personen zoekt uit die andere disciplines die dat ook echt oprecht interessant vinden. En, ja. Dus dat had ik met Henk Broer toen, die was de opvolger van Takens in Groningen, die vond het gewoon, die vond het supergaaf. Die vond, wij hadden dan onze kleine modelletjes, echt een beetje, nou ja, toy modelletjes, maar hij vond het echt oprecht interessant om daarin mee te denken, en zoiets hoop ik dus een beetje voor die scholarship positie, dat je daar toch iemand vindt die dat soort concepten ook interessant vindt en dat je dan echt, een echte samenwerking aangaat.

**MG:** Ja. Ja, want merkt u in zo'n samenwerking wel eens dat er ook misverstanden ontstaan, dus niet zozeer dat u elkaar onmiddellijk niet begrijpt, maar meer dat u erachter komt dat er dingen verkeerd begrepen worden aan beide kanten?

**P3:** Mhm. Mhm. Heb ik nu niet heel direct een voorbeeld, maar dat, waar, oh de andere samenwerking weet ik dat zeker. Daar weet ik dat zeker, en dat het ook vaak, nou ja vaak is het een, hoe gebruik je begrippen en welke associaties heb je daar daarbij, en dat check je natuurlijk ook niet altijd meteen hè, je doet niet altijd eerst even oké, zullen we even ons vocabulaire checken of we ook dezelfde dingen daarmee bedoelen, en dan, ja dan kan het best lang eigenlijk een beetje, dat je la-, ja, net niet hetzelfde bedoelt of een beetje langs elkaar heen praat. En ja, en dat dat dan pas later een keer zo van, oh, dat... Nou ja dus dat zeker, dat zeker. En die kans wordt natuurlijk alleen maar hoger als je vanuit verschillende disciplines werkt in een verschillende cultuur, en die dingen spelen natuurlijk ook allemaal nog mee.

**MG:** Ja.

**P3:** Dus ik denk dat dat, ja, dat dat belangrijk is en dat het daarom ook de kracht zit hem denk ik, dus ik ben hoopvol, maar weet niet precies waar het met dit RICH nog naartoe gaat, maar de kracht of de potentie zit hem denk ik wel in langdurige, landurigere samenwerking, waar je elkaar een beetje kent, weet waar je mee bezig bent, elkaars taal begrijpt, en zo, dat is denk ik, daar zit veel winst te behalen, meer nog dan in, ja, snel bij elkaar rapen van wat mensen, omdat er een subsidie call is of wat dan ook, want dan, daar denk ik, is het een beetje voorgeprogrammeerd dat je dan misschien toch, ja, elkaar niet goed begrijpt.

**MG:** Ja, want heeft u daar een voorbeeld van, dat het zo langs elkaar heen ging?

**P3:** Ja, ik zit even te denken, of ik daar een heel concreet voorbeeld van...

**MG:** Hoeft niet eens heel concreet.

**P3:** Nee... Weet ik niet. Dat is natuurlijk ook niet zo vaak. De RICH is een goed voorbeeld, en soms van die, nee, complexity science conference, hoe heet die, die nu ook binnenkort weer een call heeft, dus het is ook niet zo vaak dat ik op dat soort, in dat soort interdisciplinaire settingen ben, absoluut niet. Maar ik heb het wel in dat soort, ook met dat soort conferenties, ja, heb ik het, want daar zie je nu dus steeds meer dat het dan ook geprobeerd wordt om dat interdisciplinair te doen, en daar zit ik dan soms wel, en dan vertelt een of andere fysicus over space shuttles en weet ik het, dat ik dan om, maar dan kies ik dus ook alleen maar voor de lezingen waar ik denk van, oké, ja dat zou relevant- en dan heb ik nog een beetje achtergrondkennis, maar dan zie ik de andere psychologen zitten waar ik denk van, jullie hebben geen idee waar dit over gaat. En daar, ja dus daar vraag ik me dan soms af, is dit zinnig om te doen, of zou je dan niet toch een soort van pre-conference moeten doen waar je mensen een beetje bijspijkt, zodat, hm, dat je een beetje weet waar dit over gaat, of suggested reading, of weet ik veel maar dat, nou ja, dus dat heb ik af en toe wel gehad, dat je op zo'n conferentie zit en dan vertelt dus iemand, ik weet ook nog, hoe heette die ook alweer, nou ja, doet er ook niet toe, maar dat was ook op een conferentie, een psychologische conferentie, en dan kwam iemand met zo'n schaalte met fluid, weet je wel, waar die dan van die bolletjes in had, en die gingen dan, nou ja, spontane zelforganisatie van patronen laten zien en zo. Nou ja, en ik zat daar met een zaal van psychologen waar ik [...] zeker weet dat tachtig procent dacht van, wat krijgen we nu, wat doen we nu, wat heeft dit voor een relevantie. En dit is, ja, dit is wel ook iets een beetje, in die hoek zaten ook lang die dynamisch systeemtheorie mensen en complexity mensen zo van, ja, alleen maar superingewikkelde dingen doen, waar niemand eigenlijk begreep wat, waarom, wat is het hier alleen maar om, hé, we hebben pink noise gevonden, is voor de doorsnee psycholoog niet superinteressant. Dus de koppeling tussen die ingewikkelde analyses en moeilijk doen met een fenomeen wat de mainstream interessant vindt, daar vind ik, ja, daar was ook nog, en dat gebeurt nu beter waardoor het ook denk ik weer meer mensen denken ah, oké, dat kunnen we hiermee, ja, en dat sluit dus een beetje aan bij dat van, oké, wanneer zijn zo'n situaties waar je ziet van die mensen begrijpen elkaar niet. Ja, ik zie dus soms dat mensen dan zomaar bij elkaar in een zaal gegooid worden, en ik me afvraag van, volgen jullie dit? Waar gaat dit over? En daar ook weinig moeite gedaan wordt, nou ja van zo'n space shuttle engineer verwacht ik dat ook niet dat hij daar nu moeite voor doet om dit voor psychologen relevant te maken, misschien hoeft het ook niet, misschien is het voor zo'n echt truly interdisciplinary conference ook niet verkeerd, maar als het nou bijvoorbeeld om psychologische conferenties gaat waar dan zo iemand ingevlogen wordt, dan denk ik, ja, zo sla je de plank een beetje mis, als je dit niet een beetje ook probeert relevant te maken voor oké, wat kunnen we nou met die kleine magneetbolletjes in dat, ja. Dus een beetje die helpen met die vertaalslag maken.

**MG:** Ja.

**P3:** Dus je hebt eigenlijk soor- sorry, ik praat, ik ben altijd een beetje lang van stof, [...] onderbreek me...

**MG:** Nee hoor, ga door.

**P3:** Nou ja, ik denk dat eigenlijk waar je behoefte aan hebt zijn zo overbruggers of zo, die de werelden een beetje met elkaar kunnen verbinden, en die dus beide talen begrijpen, en zo

een beetje kunnen helpen om de link te leggen. Ik denk dat zo iets, ik heb dat in een hele andere, als we met de programmeurs samenwerking, dat je daar ook merkt, je hebt eigenlijk mensen nodig die, Schnittpunkt, hoe zegt je dat, die dat... Ja, de vertaler, de overbrugger kunnen zijn, die dus zelf kunnen programmeren maar die ook wetenschappers zijn bijvoorbeeld, of ook psychologen of zo, en, want als je alleen maar met die nerds zit, ja dan die doen precies wat jij ze gezegd hebt, maar dat is eigenlijk helemaal niet wat je wilt, weet je wel. Nou ja, zo. Dus ik denk dat daar, dat dat echt een, dan zou het denk ik wat meer ook van de grond komen, want we roepen dit natuurlijk ook al heel lang, met dat interdisciplinair. En in sommige velden lukt het. Maar ik vind het vaak nog best wel matig, wat ik zo zie, en ik denk dat dat misschien ook daarmee te maken heeft.

**MG:** Hm, ja.

**P3:** Ja.

**MG:** Ja, ik wil het ook nog heel even hebben over de toepasbaarheid en de klinische praktijk, daar was u eerder ook al kort over begonnen. Want, zeg maar op het hele spectrum hè, van aan de ene kant super fundamenteel onderzoek en aan de andere kant heel toepassingsgericht onderzoek, waar ongeveer zou uw eigen onderzoek zitten?

**P3:** Precies aan beide kanten, denk ik. Dus niet in het midden, maar aan beide uitersten. Want ik denk, dat dat eigenlijk, ja, dat dat vrij goed te combineren is. Of laat ik het zo zeggen, ik denk dat de wetenschap de praktijk lang geen dienst heeft gedaan omdat ze A, sowieso onderzoek op een manier heeft gedaan die geen recht doet aan het fenomeen, en dat gaat een beetje gepaard daarmee, dat het dan ook niet echt informatie opgeleverd heeft die relevant is voor de praktijk. Dus als je, nou ja, als je kijkt weer naar RCTs, dus de randomised controlled trials, dan zie je groepsgegevens, voor na, en, ja. En, maar en, professionals zitten natuurlijk niet, nooit met een groepsgegevens, dus dat, met een individuele cliënt, die, waar die het proces moet begeleiden. Dus, ja. En daarom denk ik dus dat mijn fundamenteel werk naar, oké, kunnen we nou die onderliggende mechanismes en processen van verandering begrijpen, wat best wel fundamenteel ingestoken is, maar dat dat uiteindelijk voor de praktijk superrelevante informatie oplevert. En gecombineerd met wat ik zei, dat ik toch steeds meer eigenlijk ben denken in van, oké, laten we het descriptief houden, over tijd volgen, dat is natuurlijk iets wat je heel goed in de praktijk kunt implementeren, hè, in zo'n monitoringsysteem hè. Dus dat is eigenlijk waar je, waar ik naartoe wil. En dan denk ik dat je dan in de praktijk namelijk, als je dat soort type data verzamelt hè, van dag tot dag de verandering, en dan, ja, het liefst als dat, als zij dat nuttig vinden, want daar zit ook een ander concept nog achter, het small data paradigm, heeft iemand dat genoemd, Hekler, dus dat, daar is het verschil met de big data paradigm, dus dat je niet zozeer data gaat verzamelen bij één groep om uitspraken te doen over een andere groep, maar dat je de data die je verzameld hebt, dat die meteen al bruikbaar zijn voor de unit zelf die het verzamelt. En dat is ook een beetje mijn principe, dus die dagelijkse data verzameld in een behandelcontext, die moeten ook meteen toegankelijk en beschikbaar zijn voor de cliënt zelf en de therapeut, en wij wetenschappers kunnen als dat dan aggregeert over tijd dat we steeds meer en meer hebben, kunnen we weer op zoek gaan naar bepaalde wetmatigheden en kijken en dat dan weer terugvoeden. Dus ik denk dat, en, nou ja, en dan komt weer een beetje dat

fundamentele weet je, of het nou de emoties zijn, bij de één is het boosheid, bij de ander is verdr-, dat maakt, de content maakt me niet zo heel erg uit, omdat ik toch meer op zoek ben naar dat algemene principes van, net als met early warnings bijvoorbeeld, en de content maakt dan volgens mij minder uit. Dus dan kun je ook over hele verschillende, hele ideografische cases heen, toch algemene dingen uit zeggen, ja, dus in die zin denk ik dat het, ja, dat het enerzijds best wel fundamenteel is, maar aan de andere kant ook grote klinische implicaties, en dat de crux eigenlijk is een beetje, laten we focussen op het individu over tijd, want dat is zowel voor mijn fundamenteel werk heel belangrijk en dat is anderzijds denk ik ook de, datgene wat het relevant maakt voor de praktijk.

**MG:** Ja. Ja want, hoe zou nou in bijvoorbeeld in een ideaal geval die klinische relevantie eruit zijn echt op dagelijkse basis?

**P3:** Ja, nou ja dat, daar, is dus eigenlijk waar ik nu ook met mijn Vidi op, mee bezig wil gaan, dus wat we met Merlijn gedaan hebben is natuurlijk ook, daar hebben we de hele tijdserie al verzameld gehad, toen konden we kijken, oké, waar zitten nou de grote drops, en laten we nu kijken wat daarvoor gebeurde, of kunnen we dat voorspellen met wat van te voren gebeurt. Ja, dat is natuurlijk in de praktijk niet zo handig, want dan wil je het echt op het moment doen, dus wat ik daar nu, maar dat moeten we allemaal nog uitvogelen, maar wat het plan is, is dat je werkt met control charts, wat van wasmachines of zo, door engineers is dat bedacht, nou ja, dus wat het idee is, dat ik, dat je per individu kijk je eigenlijk, oké, wat is de normale range qua fluctuaties van een persoon. Dus ik ben bijvoorbeeld een hele persoon die van dag tot dag heel erg fluctueert, iemand anders die is wat stabiel over tijd, dus dan krijg je, nou ja, afhankelijk van de baseline van die persoon, een hele brede marge daaromheen of een redelijk smalle. En dan zou ik dus willen kijken of je dan, en dan kun je daar bijvoorbeeld die complexity measure berekenen en dat je dan kijkt van oh, nu gaat die, schiet die uit zijn normale bandbreedte, nu is iets aan de hand. En dan denk ik dus ook, ja, die early warnings wat zijn dat, die geven aan dat het systeem, dat het destabiliseert, het is niet per se noodzakelijk dat dan zo'n faseovergang gebeurt hè, het kan ook weer terugvallen, dus voor mij zie ik het daarom ook meer, nou ja dus enerzijds wil ik testen van oké, als we dat zien en we passen nu een interventie toe heeft die dan een groter effect, maar anderzijds denk ik is het puur ook al als signaal interessant voor de professional, zo van hé, let even op, we zien hier dat de cliënt in beweging komt. En dat kan, maar dat kan natuurlijk ook betekenen dat die veel vatbaarder is voor negatieve invloeden en dat die ineens uit het raam gaat springen hè. Maar het kan ook zijn dat er iets positiefs een heel groot positief effect heeft. Dus ik, en daar denk ik ook weer, nu wordt het heel psychologisch, maar ik denk dat we eigenlijk de praktijk ook weer die autonomie moeten teruggeven, dat zij wel weten klinisch gezien wat verstandig is om te doen, als wij ze maar goeie data bieden die iets zeggen over de toestand van het systeem. Dus ik denk dat we weer terug moeten, eigenlijk weg van die protocollen wat een beetje soort van kookboekmentaliteit is, en meer kijken van oké, in welke toestand zit het systeem en wat is dan, en dat zou ik ook heel graag dus theoretisch willen modelleren, wat is afhankelijk van het toestand van het systeem, wat is dan een geschikte ding om te doen, dus zie ik bijvoorbeeld dat er nog helemaal geen andere toestanden available zijn in het systeem, ja dan hoef ik hem ook niet uit dat gat te pushen want, ja, waar moet die heen dan, zeg maar. Dus wat, dus dat we meer daarover nadenken,

wat doen bepaalde interventies met de stabiliteit, met de topografie, en dat je dan eigenlijk meer, ja, dat je professionals die informatie geeft en dat zij dan wel meer uit een hele range aan dingen kunnen kijken oké, wat doe ik nu, maar tegelijkertijd moeten ze altijd blijven monitoren, want dat is weer, heeft te maken met dat complexity denken, we kunnen geen lange termijnvoorspelling doen, dat is net zoals met het weer, en ik zie geen enkel reden, en we hebben het ook in data gezien, dat dat nu zo anders zou zijn. Dus ik denk, dat ook weer, dat we zijn nu echt een omslag in het denken over interventies en goal directed change, dus dat we weer een beetje terug moeten naar, een collega van mij die noemde het altijd zoals rijden in de mist, dat je gewoon, ja, je moet met een aangepaste snelheid en in staat zijn om steeds te stoppen of te reageren als dat nodig is. En zo zie ik het eigenlijk ook een beetje voor het klinische veld, en dan denk ik dan, ja, dan kunnen wij ze een grote dienst leveren door die data te geven, en, die dus iets zegt over de toestand van het systeem, en daarnaast denk ik dat puur ook de descriptieve informatie van hoe, welke dingen hangen met elkaar samen, als dit hoog is is ook dit hoog, of juist, dat is voor de praktijk ook al heel erg... En dan het liefst, want dat gebeurt nog heel weinig, met ook contextinformatie daarbij. Dat je dat ook heel systematisch kunt bekijken.

**MG:** Ja. Want op wat voor manier gaat dat nu dan in de praktijk, u noemde al die kookboekmentaliteit een beetje?

**P3:** Ja, ja. Nou ja, dus dat is een beetje, maar nogmaals, ik denk niet zozeer dat dat de fout is van de praktijk, maar vooral van de wetenschap, dat je ziet dat de, die evidence based movement in de klinische praktijk, die stoelt dus vooral op van die behandelprotocollen. Dus, jij hebt een angststoornis, dus dan pak ik op mijn kast, oh ja, protocol voor angststoornis, en dan doe ik in sessie twee dit met jou en sessie drie dit, en sessie, nou zo. En die protocollen die komen uit het onderzoek, want die waren soort van, in je methodesectie moest je wel, zeg maar operationaliseren wat jouw interventie nou precies inhield, en dat heeft ertoe geleid dat er heel erg vastgelegd werd, en dit is dan op een gegeven moment een soort van implementatietool geworden voor de praktijk, oh dit is hoe we onze behandeling. En ik denk dat heel veel, en zeker goeie behandelaren dit niet zo doen, die werken heel eclecticisch en, nou ja, zo. Maar, de valkuil is wel een beetje dat A, mensen denken van, oh ja, die heeft zo'n labeltje, en dan pak ik dit kookboek en dan volg ik gewoon al die stappen en dan komt het wel goed. En dat is denk ik het verkeerde, dat is de verkeerde insteek, dat weten we, cliënten vinden het niet fijn, die voelen zich als nummertje, professionals vinden het niet fijn en het onderzoek laat ook zien dat we zo niet verder komen, dus. En daar denk ik moeten we weer terug naar, oké kijk in welke fase de cliënt verkeert en heb dan een hele toolkit beschikbaar aan dingen die je kunt doen, waar je dan mogelijk kunt verwachten dat het systeem die kant op beweegt maar blijf het volgen want je weet het niet, dat is eigenlijk denk ik waar we een beetje naartoe moeten, maar daar moet nog heel veel meer onderzoek gebeuren. Voor nu denk ik is gewoon safe om goed te blijven volgen hoe het gaat, dat is al een begin.

**MG:** Ja. En wat voor rol zouden dan die in, meer interdisciplinaire ideeën hebben bij die verbetering van de klinische praktijk?

**P3:** Mhm. Nou ja, ik denk, wat ik zei, dus ik zie nog steeds wel grote potentie in die early warnings. Ik denk ook dat bijvoorbeeld waar we nu met Jingmeng bezig zijn van, kunnen we

nou die stabiliteit van het systeem echt kwantificeren, nu doen we het puur op simulaties, de volgende stap zou dan zijn, oké, kunnen we dat ook linken aan empirische data, dat zou ik superinteressant vinden. Dus iets van, ja, nou ja, wat ik net probeerde, dat is een beetje mijn droom, maar dat je toch data beschikbaar hebt waardoor je een beetje een soort van landschap van een persoon kunt construeren, en dat je dan daarover nadenkt, oké, wat zouden we nu kunnen doen om het landschap te veranderen, en voor welke type verandering dan van de toestand van een systeem verwachten we nou wel early warnings, geen early warnings, hè, daar zijn natuurlijk heel veel verschillende bifurcaties, en, ja, dat kunnen we echt niet alleen oplossen als psychologen. Dus daar hebben we goeie, ja, daar hebben we mensen nodig die goed zijn in de wiskunde en die goed zijn in modelleren, en modelbouwen, en gevoed dus inderdaad, ja, wel gevoed door de psychologische inhoud, dat is denk ik, dat zou ik heel leuk vinden, want ik, dat zie ik- want ik denk ook niet dat al het onderzoek naar specifieke interventies en bepaalde interventie-elementen dat dat nu nonsens is, hè, dat denk ik ook niet, ik denk dat dat, maar dat je het een beetje met elkaar in verbinding moet brengen, dus dat is een beetje de uitdaging, of voor mij, waar ik me de komende jaar mee bezig wil houden. En daar zie ik absoluut grote winst in samenwerking met jullie. Ja.

**MG:** Ja. Nou, lijkt mee een mooie afsluiter, tenminste ik denk dat ik alles heb, is er nog iets wat u zou willen toevoegen in dit kader wat nog niet echt aan bod is gekomen?

**P3:** Nee, nee. Ik heb...

**MG:** Oké.

**P3:** ...veel gepraat.

**MG:** Ja, hartstikke fijn. Ja dan zet ik de opname even uit, dan was...

## **Participant 4**

**MG:** Yes. Oké. Ja voor we beginnen nog even iets formeels over de verwerking van de data en zo. Ik ga het interview dus transcriberen en de opnames en zo worden ook bewaard, die zijn alleen toegankelijk voor mijzelf en voor mijn supervisors. Voor de verwerking in het eindproduct uiteindelijk kan ik de inhoud als u dat wil volledig anonimiseren, en dan op zo'n manier presenteren dat het niet tot u te herleiden valt. Maar als u dat toestaat zou ik wel gebruik willen maken van de mogelijkheid om als dat relevant is naar uw naam en achtergrond te verwijzen.

**P4:** Prima.

**MG:** Ja, vindt u dat oké?

**P4:** Ja hoor.

**MG:** Super. Oké. Nou ja, dat was het voor mij, dan kunnen we beginnen denk ik.

**P4:** Ja.

**MG:** Ja. Als korte introductie misschien eerst even iets over uw onderzoek in het algemeen. Dus als u nu in een paar zinnen zou moeten beschrijven waar uw onderzoek over gaat aan een wetenschappelijk opgeleide collega die geen medische achtergrond heeft, wat zou u tegen zo iemand zeggen?

**P4:** Ons onderzoek gaat in ieder geval uit naar de ziekten en behandelingen van oudere mensen, en die hebben vrijwel allemaal meerdere ziekten tegelijkertijd en meerdere beperkingen tegelijkertijd. Dus wij proberen in die complexiteit van interacties tussen ziekten en beperkingen te kijken wat goeie diagnostiek en behandeling is, zelfs als mensen cognitieve problemen hebben. En omdat dat gepaard gaat met heel veel interacties, met moeilijk voorspelbare prognoses en behandel-effecten, hebben wij sterk behoeften aan andere methodologie dan de lineair causaal gerichte epidemiologische technieken. Vandaar dat we ook sterk geïnteresseerd zijn, leunen op, methoden die meer in het veld van de complexity science worden gebruikt.

**MG:** Ja, helder. Ja, misschien kunnen we daar meteen even op doorgaan dan, over die methodiek, want, ja, ik ben wel geïnteresseerd in de methoden die u dan toepast concreet in uw onderzoek. Dus als u eens terugdenkt aan een onderzoekslijn of een project waar u de afgelopen jaren aan gewerkt heeft, wat voor technieken en methoden heeft u in dat onderzoek ingezet om uw onderzoeksvragen te beantwoorden?

**P4:** Bij één project is inderdaad gericht op de uitkomsten van behandeling bij mensen met een dementiesyndroom, en daar hebben we als uitgangspunt multicausaliteit gekozen, dus eigenlijk uitgangspunten, theoretische uitgangspunten, vanuit het complex systems paradigma. Multicausaliteit, non-lineariteit, interacties die eigenlijk ook leiden tot emergentie van nieuwe problemen. En methoden die we daarbij hebben gebruikt, we zijn gestart met een aantal sessies van group based modelling, en daar hebben we een causaal loop diagram mee ontwikkeld, CLD's, en vanuit die CLD's zijn we gestart met kwantificatie van



simulatiemodellen, van computational simulatiemodellen, met name system dynamics model, om te kijken of je op die manier zowel op populatie als op individueel niveau voorspellingen kunt doen bij beïnvloeding van enkele van de risicofactoren.

**MG:** Misschien kunt u daar iets meer in detail over uitleggen, want u begon over group based modelling, of?

**P4:** Ja.

**MG:** Hoe zit dat in elkaar?

**P4:** Dat is dus een methode die al gebruikt wordt met name ook in de sociale wetenschappen en die is gebaseerd op zowel het bundelen van literatuur als van expert knowledge. In feite is het een soort kwalitatieve onderzoeksmethode die je ook sterk kunt standaardiseren om daarmee tot een overzicht en een consensus te komen, maar dan niet een consensus zoals dat meestal wordt gedaan in de zin van richtlijnontwikkeling naar meer lineaire statements, maar veel meer naar een interactief model waarin ook bijvoorbeeld causale loops in zitten.

**MG:** Ja, want hoe werkt dat precies?

**P4:** Nou, dan kun je dus met een aantal sessies, als je die hebt voorbereid met literatuuronderzoek, groepen uitnodigen van experts, goed zorgen dat je voldoende diversiteit in die groepen hebt. En dan gaat het eigenlijk om de bundeling en de linking van onderzoeksdomeinen aan elkaar. Je moet ook eerst zorgen dat je zeg maar de cruciale termen op orde hebt, zodat iedereen dezelfde terminologie gebruikt ofwel begrijpt wat een term in een ander vakgebied betekent. En vervolgens kun je gaan nadenken over hoe, met een bepaalde uitgangsvraag – bijvoorbeeld in ons geval, een startuitgangsvraag van hoe kun je cognitieve functie in de tijd voorspellen bij ouderen, kun je onderliggende drijvers van die uitkomst en de interacties daartussen bediscussiëren, en dan, al discussiërend, vorm je daar tegelijkertijd een theoretisch model van. En dat theoretisch model laat zowel de parameters zien, maar ook de aard en de vorm van de interactie. Dus is het een positieve interactie, is het een negatieve interactie, zitten er loops in, is het een wederzijdse beïnvloeding. Daarover discussieer je, en al discussiërend wordt dat model meestal vrij snel steeds complexer. Nou, dat kun je dan in een aantal sessies bespreken. Je laat eerst een eerste versie van zo'n model, je geeft dat terug en vraagt iedereen nog heel kritisch te kijken voor een volgende sessie of er nog wijzigingen moeten komen, als het kan ook evidence te leveren per parameter die in het model komt en per interactie die is voorgesteld. En zo probeer je zo stevig mogelijk onderbouwd een kwalitatief model te realiseren wat al meestal totaal anders is dan de simpeler epidemiologische modellen die in de literatuur verschijnen, omdat die vaak gebouwd zijn op statistische methoden die, ja, meestal onvoldoende power hebben om die interacties te bestuderen.

**MG:** Ja, kunt u daar iets meer over zeggen, over dat onderscheid tussen wat u nu beschrijft en de meer gangbare techniek?

**P4:** Ja. Nou, het onderscheid is dus in deze fase van kwalitatief onderzoek is dat eigenlijk er vrijwel nooit in de gebruikelijke epidemiologische studies die we doen een formele stap van

kwalitatief modelbouw is, die ontbreekt vrijwel altijd, en dat heeft te maken met het feit dat die hypothesevorming meestal heel erg simpel is. Het gaat meestal over de vraag, beïnvloedt A B...

**MG:** Ja.

**P4:** ...en hoe is die beïnvloeding. Ja daar heb je dan, als je dat als hypothese hebt, daar heb je ook meestal niet echt een voorstudie met kwalitatief onderzoek voor nodig, want die vraag beïnvloedt A B komt meestal ook al uit voorgaand onderzoek wat de groep zelf of anderen hebben gedaan. Maar als je de beïnvloeding van B door A wilt plaatsen in het perspectief van de belangrijkste andere factoren die ook B beïnvloeden dan wordt het een heel ander verhaal, en dan heb je dus wel zo'n stap nodig van, maar hoe ziet dat totale model er dan eigenlijk uit, wat is de meest realistische benadering, en kun je dan iets zeggen over de sterkte van die relatie A-B ten opzichte van allerlei andere relaties die ertoe doen in die fysiologie. Dus die stap ontbreekt en die stap die voegen we in. En vervolgens gaan we niet zozeer kijken naar, zijn er dan datasets waarin elk individueel interactieonderdeel ook te bestuderen is, we gaan veel meer kijken naar datasets waar zoveel mogelijk van de componenten vertegenwoordigd zijn om daarmee ook die indicatorsets te kunnen gebruiken om een computationeel model te kunnen bouwen. En die computationele modellen die zijn echt anders dan dat je een, bijvoorbeeld, een lineair regressiemodel bouwt, omdat dat uitgaat van, het woord zegt het al, in principe altijd lineaire afhankelijkheden. Terwijl dat bij de computationele modellen helemaal niet zo hoeft te zijn.

**MG:** Want hoe zit dat daar dan?

**P4:** Nou, dat hangt heel erg af van het aantal componenten dat je in een model, in een simulatiemodel opneemt, maar zelfs de meest simpele modellen, bijvoorbeeld system dynamics modellen met stocks en flows, die zorgen al voor non-lineariteit, omdat je een stock hebt die langzaam of snel leegloopt, ja, dat is al een soort drempelfactor in een model waardoor het hele model niet meer lineair verloopt. En dan heb je eigenlijk nog maar de meest simpele vormen van modelbouw, die al heel snel, zeker als je er meer stocks en flows in opneemt, allerlei afhankelijke niet-lineaire modellen met zich mee brengen. En je moet dus echt gaan simuleren om te kijken hoe het uiteindelijke model eigenlijk, wat voor, wat voor dynamiek dat laat zien. En dat kun je natuurlijk valideren op de dataset, maar dan veel meer op de dataset als geheel met alle factoren die daarin zitten. Meestal wordt dan een deel van de dataset gebruikt bij de ontwikkeling van het model en een onafhankelijk deel wat niet gebruikt is voor de ontwikkeling gebruik je voor een eerste validering om te kijken of prognostische uitkomsten ook echt kloppen met dat deel van de dataset. Nou, het is ook in epidemiologisch onderzoek niet ongebruikelijk om datasets te splitsen, maar meestal gaat het dus om veel simpeler lineaire verbanden tussen één of hooguit enkele van de factoren, en dat proces loopt hier echt anders. En vervolgens heb je dan nog idealiter ook externe datasets om een model ook buiten zijn eigen ontwikkelomgeving, bijvoorbeeld in internationaal perspectief, te valideren. Dus er zitten wel wat gelijkaardige stappen in, maar de methodologie van een system dynamics model bouwen is echt heel anders dan die van een lineair regressiemodel opzetten en de analyse daarop uitvoeren.

**MG:** Ja. En hoe bent u er zelf nou bij gekozen om voor deze methode te kiezen in plaats van die lineaire regressiemethodiek?

**P4:** Daar zijn wij toe gekomen, dat is een goede vraag, dat heeft een aantal oorzaken. We zitten als we bijvoorbeeld kijken naar het alzheimerveld al heel lang met een lijn die gebaseerd is op één paradigma van oorzaken van alzheimer, eigenlijk het aggregeren van eiwitten, beta-amyloid eiwit, van 42 aminozuren, dat is al een jaar of dertig eigenlijk de leidende hypothese, dominante hypothese in dit veld. En die gaat er dus vanuit dat stapeling van amyloid lineair ook met zich meebrengt achteruitgang van cognitie en dus het ontstaan van dementie. Dat is een vrij simpele hypothese. Daar is vervolgens in de literatuur wel evidentie voor gevonden, maar ook wel heel veel literatuur die dat niet zozeer ondersteunt, maar desalniettemin zijn er stappen ondernomen om medicatie te ontwikkelen die op allerlei manieren dat beta-amyloid in vorming blokkeren. Nu zijn er talloze trials gedaan om die medicamenten te onderzoeken en aanvankelijk lukte het niet om beta-amyloidstapeling te verminderen en werd er zeker ook geen effect op cognitie te zien. De laatste jaren zijn er ook studies die laten zien dat beta-amyloid wel te verminderen is, maar dat het eigenlijk geen impact heeft op cognitie. Met andere woorden, er is heel veel geïnvesteerd in, zeg maar, empirisch onderzoek op deze hypothese, deze vrij simpele hypothese, maar uiteindelijk is er geen data die ondersteunt met zeg maar de proof of pudding van die simpele causaliteit met therapie dat dat ook zo werkt, en ik denk dat dat vooral komt omdat beta-amyloid maar één van de factoren is die cognitie bij ouderen doet achteruitgaan, en omdat het minder ophopen van beta-amyloid nog geen beperking oplegt aan al die andere mechanismen die ook cognitie negatief beïnvloeden. En dan heb je dus een heel ander soort paradigma en heb je ook andere methoden nodig om te ontsnappen aan weer een volgende simpele lineaire statement die het gevaar loopt opnieuw veertig jaar onderzoek op één mechanisme te baseren. Dus vandaar kwamen wij nadenkend op van wat kun je dan nog meer, en wat zijn alternatieve methoden om dit integraler te bestuderen. En er is natuurlijk veel aan systems biology en system dynamics onderzoek binnen, zeg maar, de proteomics en binnen de genetica en ook wel binnen de cognitieve neuroscience, maar het daarbij ook verschillende schaalniveaus met elkaar verbinden, bijvoorbeeld van het proteomicsdomein een verbinding maken naar cognitie, dat is nog niet voorhanden. Dus op dat terrein zijn wij aan het pionieren eigenlijk.

**MG:** Ja. Ja, en u noemde net al dat bijvoorbeeld dat kwalitatief modelleren wat u doet, dat dat in de sociologie bijvoorbeeld wel meer gebeurt. Zijn er meer van dat soort technieken die u gebruikt die niet per se afkomstig zijn uit de medische wetenschap?

**P4:** Nou ja, dat is eigenlijk ook zo met een andere vorm die we gebruiken, dat is de netwerkanalyse, en daar is nu al wel wat meer body voor, maar zeg maar in de fysiologie, met name in de fysiologie van, zeg maar de lichamelijke ziekte, daar zijn netwerkmodellen eigenlijk nog steeds heel spaarzaam, en ook die netwerkanalyses komen veel meer uit de sociale wetenschappen, of, en uit de zeg maar de economische wetenschappen, bedrijfswetenschappen, waar al veel langer en ook sterk kwantitatief is gewerkt met netwerkmodellen, en dat is een andere methode die wij ook proberen te gebruiken, waar het gaat om interacties tussen symptomen bijvoorbeeld, symptoomnetwerken bouwen, en niet

alleen meer kijken naar onderliggende ziektes, [...] ziektenetwerken die je ook kunt bouwen en die, waar we ook wel mee doende zijn, maar ook symptoomnetwerken bouwen om te kijken van, is het niet zo dat bepaalde symptomen elkaar op zich ook heel sterk beïnvloeden en dat bijvoorbeeld iemand die in coronatijd minder kan bewegen, minder naar buiten kan, minder mobiliteit heeft, daardoor ook slechtere voeding heeft, eigenlijk ook minder prikkels van buiten opdoet, daardoor zijn brein minder geprikkeld wordt en zijn cognitie ook verslechtert, allerlei ingrediënten voor zeg maar samenhangende symptomen, nog los van wat iemand onderliggend aan ziekte heeft, maar die elkaar al sterk kunnen beïnvloeden. Nou, die netwerkmodellen dat is een andere tak van sport naast die simulatiemodellen, die ook wel weer gebruikt kunnen worden in de simulatiemodellen, maar ook zonder simulatiemodellen kunnen worden geanalyseerd, waar we ook mee doende zijn en die je binnen de geneeskunde eigenlijk nu vooral op het domein van psychologie en psychiatrie al ziet gebruikt worden. En een beetje op het terrein van de epidemiologie, waar dat al wat langer, bijvoorbeeld met progressie van HIV en de factoren daarvan, daar zijn ook al wel een jaar of tien, daar is een netwerkmodellen in gebruik, maar verder in zeg maar hardcore [...] geneeskunde is dat ook nog een methode die vrij weinig gebruikt wordt, waar je nu juist wat meer goede papers ziet die dat ook kwantificeren en ook aangeven wat daar de implicaties van kunnen zijn.

**MG:** Ja, want het is kwantitatief, zo'n netwerkanalyse?

**P4:** Dat begint ook vaak kwalitatief, maar uiteindelijk is dat ook kwantitatief, en kun je daarmee ook weer grip krijgen op uiteindelijk complexe verschuivingen in de fysiologie, waarbij je dan ook andere termen uit het complexity science veld zoals tipping points, resilience, ziet verschijnen, maar ook zonder die terminologie worden al netwerkmodellen gebruikt, bijvoorbeeld ook in de microbiologie, om evenwichten tussen het microbioom, daar is laatst nog een goede paper van in Nature verschenen – aanvankelijk keken we alleen naar, oké, wat doet een antibioticum op een bacterie en kun je die bacterie daarmee de baas worden, kun je zorgen dat een infectie bestreden wordt, maar deze auteurs die lieten bijvoorbeeld zien dat er honderd bacteriën heel sterke interacties met elkaar hebben, en dat ook afhankelijk van het hele palet aan interacties in het microbioom het meer of minder gemakkelijk is om een infectie te bestrijden, dus dat het niet alleen maar de gevoeligheid is van één bacterie voor een bepaald antibioticum, maar veel meer de gevoeligheid van het hele ecosysteem met allerlei onderlinge interacties voor antibiotica en die maakt of je wel of niet in staat bent om een infectie te bestrijden. Maar dat zijn inzichten die dus andere fenomenen uit de realiteit kunnen verklaren, omdat daar de empirie en de grenzen van behandeling al wel langer bekend zijn.

**MG:** Ja. Ja en, in hoeverre heeft u daarbij wel eens moeilijkheden ervaren als het gaat om het overdragen zeg maar van bijvoorbeeld zo'n netwerktheorie van dan sociologie naar uw eigen vakgebied?

**P4:** Ja. Nou, dat is altijd lastig natuurlijk, om iets uit een ander domein te introduceren en te zeggen van, is dat niet ook zinnig binnen dit vakgebied en dat is ook al een hele tijd zo voor kwalitatief onderzoek in engere zin. Het is binnen de geneeskunde en zeker de high impact journals absoluut ongebruikelijk om überhaupt kwalitatief onderzoek te publiceren, omdat

dat, of mede omdat dat ook een vreemde methodologie is die veel meer uit de gamma-wetenschappen komt. Dus daar zie je al een eerste probleem, dat als iets niet strookt met de traditie in een veld dat het lastig wordt om dat als waardevolle methodologie te gebruiken. En dat zie je dus ook al een tijd bij de andere technieken uit complexity science. Het is al wat makkelijker wanneer je dat hard gekwantificeerd kan worden, dan is de acceptatiedrempel wat lager, maar bijvoorbeeld voor computational science, simulatiemodellen, is het ook nog niet zo zomaar geaccepteerd als technologie. Ik denk dat daar wel wat beweging in komt met de grote aandacht voor artificiële intelligentie, omdat je daar eigenlijk ook maar ten dele in staat bent tot kwantificatie en juist moet leren leven met black box modellen waar je eigenlijk niet weet wat precies de factoren zijn en hoe die kwantificatie tot stand komt. Dus je ziet wel natuurlijk dat mensen zoekend zijn. Het spannendste is natuurlijk of je ook echt met een nieuwe techniek je meerwaarde kunt aantonen op het niveau van impact in patiëntenzorg, in geneeskunde, als je dat hard kunt maken dan heb je natuurlijk de grootste kans om ook snel tot acceptatie te kunnen komen, en ook daar, en daar moet je wel realistisch in zijn, is het nog niet zomaar evident hoe je vanuit complexity science ook echt patiëntenzorg in engere zin sprongen vooruit helpt.

**MG:** Ja. Ja, daar wil ik later ook nog even op terugkomen. Maar als ik het goed begriip van wat u nu zegt zit de moeilijkheid hem voornamelijk in het accepteren of de acceptatie dat deze technieken minder kwantitatief zijn dan misschien gebruikelijk is?

**P4:** Daar is een belangrijk... En daarnaast is het natuurlijk ook wel zo dat de definitie, de terminologie die gebruikt wordt, daar zitten ook wel begripsproblemen. Interdisciplinair onderzoek wordt vaak gestart zonder expliciet stil te staan met, maar zijn onze termen eigenlijk wel voldoende gelijkaardig, en dan kom je er lopende het onderzoek of lopende een projectaanvraag pas achter van, eigenlijk bedoelen we iets verschillends, het lijkt wel op elkaar maar het is echt verschillend wat we hier bedoelen.

**MG:** Kunt u daar een voorbeeld van geven misschien?

**P4:** Nou ja, we hebben laatst zelf een projectaanvraag gedaan die, waar ook mensen vanuit de besliskunde aan meededen, en daar bleek in ieder geval die termen van resilience en ook wel robuustheid, die bleken binnen de besliskunde een heel andere lading te hebben dan dat wij ze vanuit, zeg maar de ecologie en de fysiologie hadden geladen, en daar kwamen we ook pas relatief laat achter, terwijl voor die [...]...

**MG:** Waar zat dan...

**P4:** ...speelt zich dan af op kritiek op zinnen, op voorstellen, waarmee je nog niet precies in de gaten hebt van nou, hoe diep zijn nou die verschillen.

**MG:** Ja, waar zat dat verschil dan in?

**P4:** Nou, het verschil zat voor een deel in het feit dat vanuit zeg maar de geneeskunde wij resilience vooral vertaalden naar het niveau van de individuele mens, het systeem van evenwichten en hoe kun je zo'n evenwicht in feite steviger maken zodat er meer buffer is en sneller een persoon in feite terug kan gaan naar zijn evenwichtsconditie, terwijl vanuit de besliskunde werd dat al heel snel vertaald van, dat gaat niet zozeer op het organismeniveau,

maar dat gaat veel meer op het niveau van organismen in een grote samenhang met andere spelers daarin, en dus ook allerlei sociale mechanismen die meebepalen of dat systeem uiteindelijk in evenwicht is bij beslissingen die worden genomen. Nou, dat verschil in het kijken naar welk systeem hebben we het over, dat moet je van te voren wel heel goed eigenlijk in beeld brengen.

**MG:** En hoe heeft u dat toen opgelost toen u daarachter kwam?

**P4:** Nou, toen zijn we een stapje teruggegaan en hebben daarover wel gediscussieerd en uiteindelijk ook van elkaar gevraagd van schrijf nou eens precies op, formuleer heel precies wat jij met dit begrip bedoelt, en hoe vertalen we dat in de projectaanvraag, kunnen we met één van beide uit de voeten, of moeten we expliciet het verschil bij verschillende delen van het project aangeven, van in dit verband is het zo gedefinieerd. Dus we hebben die definities echt scherp gemaakt en vervolgens de tekst en het voorstel daarop aangepast.

**MG:** Ja. Ja, dus u werkt wel vaker samen met mensen van buiten de medische wetenschap begrijp ik?

**P4:** Ja, ja, dat heeft ook al veel vruchten afgeworpen, maar is niet altijd, niet altijd simpel, maar ook wel, ja, toch wel heel erg inspirerend. En in die zin zijn we begonnen eigenlijk met samenwerking een, ja een jaar of zes zeven geleden met Marten Scheffer uit Wageningen vanuit de ecologie, en dat was ook wel een hele stap, maar, ja, dat heeft wel, heeft in ieder geval ook een proefschrift, een gezamenlijk proefschrift opgeleverd, wat zelfs een cum laude is geworden, en daardoor ook wel heeft gesterkt van, je kunt dus wel paradigmavernieuwing op die manier realiseren, terwijl we ook wel hebben gemerkt lopende de rit van dat is, niet een gemakkelijke weg, niet zo simpel als we hebben een lopende trein en we doen een volgend onderzoek daarin, maar dan moet je echt een nieuwe trein proberen te laten lopen, en dat is, ja dat is spannend, voor de onderzoeker, voor ons was dat ook zoeken naar hoe doen we die samenwerking zo goed mogelijk.

**MG:** Ja. Ja, want hoe zag dat er dan concreet uit, met Scheffer dan bijvoorbeeld, hoe waren die, hoe zijn de rollen in zo'n samenwerking verdeeld, zeg maar?

**P4:** Nou wij hadden toen een promovendus die in ieder geval ook een anderhalve dag in de week naar Wageningen in lieten gaan om bevrucht te raken door de discussies daar en ook de verschillende stappen van het onderzoek en haar hoofdstukken van beide kanten te laten becommentariëren. En we hebben daar ook wel in verschillende fasen van het onderzoek wat verschillende accenten gelegd, in de zin van, uiteindelijk moest het wel een promotie worden, moest het onderzoek worden wat niet zozeer in de ecologie zou worden gepubliceerd, maar vooral in de geneeskunde, dus wij hebben daar uiteindelijk wel hier wat meer de lead genomen, maar die modellen die ze heeft ontwikkeld, die hadden we nooit kunnen gebruiken zonder dat ze ook kennis en methoden had meegenomen, bijvoorbeeld in de zin van dynamische indicatoren van resilience uit tijdseries, dat is echt iets wat ze daar heeft opgepikt en bij ons heeft geïntroduceerd.

**MG:** Ja zijn er meer van dat soort dingen waarvan u zegt van, oh ja, als we echt puur binnen de medische wetenschap hadden gebleven, dan waren we daar niet toe gekomen?

**P4:** Nou, de andere samenwerking geldt dat eigenlijk hetzelfde voor, dat is met de groep van computational science die we hebben in Amsterdam, met het IAS en de UvA, en daar hebben we met Peter Hoekstra ook een soort soortgelijke samenwerking en ook een promovendus, zelfs twee promovendi nu lopen, die op een soortgelijke manier, zowel in Amsterdam supervisie hebben, ook met Rick Quax vanuit computational science, en op die manier een team hebben wat nadrukkelijk, ja die interacties heeft, en bereid is om daar ook wat vertraging door op te lopen, maar wel de winst te realiseren van, we doen iets echt nieuws. En daar moet je ook wel de mensen op uitzoeken, heb ik gemerkt. Niet iedereen is daarvoor in om dat te doen als, bijvoorbeeld als promovendus. Sommige mensen hebben niet echt een voorkeur voor toch wat meer de vragende onderzoekende route en willen liever vanaf het begin heel scherp en duidelijk hebben van, dit ga ik doen, en dit worden mijn onderzoeksopdrachten.

**MG:** Ja. Ik kijk even door mijn vragen heen hoor. Ja, oké. Als we nu nog een stukje verder uitzoomen eigenlijk, want we hebben nu heel veel over concrete methoden en zo gehad, maar als we nou kijken naar het begrip complexiteit in het algemeen, dat is natuurlijk een ontzettend breed begrip wat ook heel verschillend wordt opgevat. Als ik nu aan u vraag wat complexity science voor u betekent, wat zegt u daarop?

**P4:** Ja. Ja. Dat is inderdaad, ja, een goeie vraag, maar ook een vraag die heel veel verschillende antwoorden oplevert. Voor ons heeft dat te maken met complexity van, zeg maar, het onderzoeksfocus wat je hebt, dus dat het gaat om multicausale problemen met veel interacties, die vaak ook niet lineair zijn, en waar ook de historie van het systeem belangrijk is om te begrijpen waar het systeem naartoe gaat en waar je ook rekening wilt houden met fenomenen zoals emergentie, het ontstaan van nieuwe evenwichten die je niet kunt voorspellen, en ook met niet-lineaire kantelpunten. Dus als je zo'n dynamiek ziet eigenlijk in de realiteit van een persoon of van een ziekte, dan hebben wij het idee dat complexity science daar niet het laatste antwoord, maar wel een antwoord, een benadering kan zijn, die op deelvragen ook behulpzaam is. En je ziet toch in veel van de ziektebeelden en veel van de vragen van de geneeskunde wel elementen van die beschrijving terug. Dus dat is de meest voorkomende manier waarop ik complexity science gebruik. Hetzelfde, dezelfde onderdelen zie je ook wel op de niveaus van gezondheidszorg en publieke gezondheid terug, waar het veel meer gaat om macroniveau van populaties of van gezondheidsinstellingen. En dan gaat het veel meer naar ofwel de managementkant, van hoe resiliënt is een organisatie, hoe resiliënt is de hele coronastrategie eigenlijk geweest, en aan de andere kant met publiek, publieke gezondheidszorg, ja, wat zijn de effecten van complexe interacterende maatregelen, zoals bij een lockdown een avondklok, beperken tot anderhalve meter, allemaal maatregelen die ieder voor zich onduidelijke effecten hebben en die je veel meer in combinatie, maar dan ook in combinatie met bijvoorbeeld effecten op scholing, op het sluiten van scholen voor kinderen, bestudeerd moeten worden. Dus er zijn verschillende niveaus van problemen waar onderdelen van complexity science goed op passen, die in ieder geval een alternatief bieden om het andere verhaal ook te vertellen.

**MG:** Ja. Ja, en hoe groot is op dit moment de rol van dat begrip complexiteit in uw eigen onderzoek?

**P4:** Nou dat is, dat is vrij groot, omdat wij, zowel waar het gaat om een deel van ons dementiegerelateerd onderzoek zijn wij eigenlijk afgestapt van dat paradigma van, alzheimer ontstaat op hoge leeftijd door amyloid, we zijn juist gestapt naar een paradigma van alzheimer op hoge leeftijd is een complexe multicausale aandoening, waarbij je dus, waarbij wij eigenlijk zeggen van, ja, wij hebben voor dat hele veld de tools en de theorievorming van complexity science nodig. Ander onderzoek wat we nu doen gaat daar soms nog wat, beweegt wat heen en weer, we maken zeker ook gebruik van bekende epidemiologische technieken, bijvoorbeeld als het gaat om diagnostische waarde van, ik noem maar iets, handknijpkracht wat we nu ook valideren, maar meestal proberen we dat ook wel te tillen naar, oké, maar als je nu met tijdreeksen gaat kijken en je gebruikt wel dynamische resilience indicatoren als één van de mogelijke manieren om dit te kwantificeren, wat levert dat op aan validiteitsonderzoek? Dus het levert ons een extra manier op om naar dezelfde data te kijken.

**MG:** Dus als ik het goed begrijp dan is een combinatie ook mogelijk volgens u?

**P4:** Zeker, ja, zeker. Ja.

**MG:** En merkt u wel eens verschil...

**P4:** [...] hoeft niet het één of het andere te zijn.

**MG:** Nee, oké. Ja. En merkt u wel eens verschillen in uw begrip van complexiteit met bijvoorbeeld collega's, kan binnen uw werkveld of daarbuiten?

**P4:** Nou dat is zeker aan de orde, en wij zijn bijvoorbeeld op dit moment een paper aan het schrijven voor Nature Communications met gerontologen uit een redelijk groot internationale groep, en die groep heeft zich al zelf geselecteerd doordat het allemaal mensen zijn die wel vinden van, op dat probleem van aging met meervoudige verouderingsmechanismen is dit een relevante toevoeging. Maar het is nog niet zo simpel om dan gezamenlijk een paper te schrijven die dat ook hard maakt, en goeie voorbeelden daarvan geeft, dus dan merk je dat definities, dat aanpakken, daarin verschillen. Op dit moment zijn we nog steeds doende dus je kunt zeggen nou, de gemene deler en het enthousiasme voor zo'n aanpak is nog steeds groter dan de verschillen, maar die verschillen zijn er wel, en proberen we dan op dit moment ook duidelijker te maken, de collega's die meer uit de biologie en de biochemie komen, die hebben daar meer een wat andere manier van omschrijven voor dan wij als klinici, en hoe krijg je dat bij elkaar rond aansprekende voorbeelden, het concreet maken met voorbeelden, en ook successen en failures daarbij zo eerlijk mogelijk benoemen, helpt wel.

**MG:** Ja. Ja, nog even weer iets anders. U begon een tijdje terug alweer over de, nou ja, de patiëntenzorg en klinische praktijk en zo. Dus daar nog even wat over, als u nou kijkt naar het spectrum van aan de ene kant heel fundamenteel onderzoek wat nog heel ver af ligt van toepassing en aan de andere kant direct klinisch toepasbaar onderzoek, waar in dat spectrum zit uw eigen onderzoek ongeveer op dit moment?

**P4:** Nou, wij zitten aan het translationele kant van veel methoden die op de een of andere manier al werkzaam zijn gebleken bij kleine groepen sterk geselecteerde mensen, fitte mensen meestal, wat is daar de toepassingsbreedte bij mensen met multiborbiditeit van. Dus



wij zitten heel erg aan die kant van toepassing in de klinische praktijk, wat heeft de patiënt van nu daaraan, en we zijn minder aan de fundamentele kant, zeker niet basaal wetenschappelijk met laboratorium of proefdiermodellen werken wij eigenlijk niet, maar wij werken vooral met vanaf grote datasets naar het kijken naar die kwetsbare grote patiëntengroep, ook omdat we tegenwoordig natuurlijk enorme vraagstukken hebben rond veroudering, met grote vraagstukken rond beheersbaarheid van kosten, toepassing van allerlei nieuwe technologie, waarbij je de vraag in ieder geval hardop moet stellen, denk ik, van iets wat op zich werkt voor een veertigjarige, levert dat nog steeds voldoende effect op bij een tachtig, vijftientachtjarige, waarbij de indicatie op zich wel gesteld kan worden als je reductionistisch kijkt, maar waarbij de indicatie misschien niet overeind blijft als je kijkt naar het integrale probleem van zo'n persoon. Dus omdat daar maatschappelijk nu ook een enorm issue is, concentreren we ook ons werk vooral op die kant, translatie in de praktijk.

**MG:** Ja. Ja, u gaf eerder ook al aan dat die toepasbaarheid misschien niet direct vanzelfsprekend is. Wat bedoelde u daarmee?

**P4:** Nou ja, om een voorbeeld te noemen hè, er zijn allerlei interventies, die nu, die vrij ingrijpend zijn, en dat gaat van nieuwe hardklepchirurgie of katheterstrategieën om hartkleppen in mensen te vernieuwen tot heel strikte bloeddrukregulatie onder heel lage bloeddrukniveaus die voor jongere en zeer fitte mensen een [...] voordeel opleveren, maar als je dan komt bij een aantal oudere mensen die al problemen hebben, dan is het de vraag of zo'n nieuwe hartklep überhaupt iets doet aan kortademigheid als iemand maar heel beperkt mobiel is, als die ook nog COPD heeft, hoe krijg je dat scherp voor wie het wel en voor wie het niet een bijdragende interventie is. En voor die bloeddrukbehandeling geldt hetzelfde, hoe haal je de mensen eruit van wie eigenlijk op basis van bijvoorbeeld cerebrale, cerebraal-vasculaire schade kunt voorspellen dat die mensen bij zo'n lage bloeddruk een te geringe cerebrale perfusie hebben en dan wegrakingen gaan krijgen, of valpartijen laten zien. Dat is een heel spannend veld nu, omdat er, ja, er zijn al veel technologische interventies komen er steeds sneller op de markt, maar het is vaak stilzwijgend dat de indicatie dan wordt uitgebreid dat iedereen die die, die dat probleem heeft zonder reserve over, van, maar is de andere bijkomende ziektelast niet zo sterk interacterend dat het eigenlijk niet meer werkt. En daar voelen wij heel erg een noodzaak om juist vanuit dat perspectief en met [...] als één van de ingangen te kijken van, hoe kun je dat empirisch hardmaken, en modellen ontwikkelen waarmee je ook aantoonst en handvatten geeft om te zien waar het wel en waar het niet nog bijdraagt aan welzijn.

**MG:** Ja.

**P4:** En dat eerst op behandelaarsniveau, maar uiteindelijk zou je dat idealiter ook op het niveau van patiënten eigenlijk graag willen, zodat die mee kunnen denken en ook kunnen zien, van oké, in welke groep zit ik nu, ga ik daar nog winst van halen van zo'n interventie, omdat dat voor veel mensen ook een, ja, heel moeilijke vragen zijn die ze gesteld krijgen.

**MG:** Ja want hoe zou dat er dan uitzien bijvoorbeeld, in de praktijk, stel het wordt een ideale situatie, over een aantal decennia, dat uw onderzoek echt dagelijks kan worden toegepast...

**P4:** Ja.

**MG:** ...hoe zou dat er dan uitzien?

**P4:** Nou dat zou eruit kunnen zien in de vorm dat je eigenlijk van mensen op het moment dat die een klachten krijgen, symptomen hebben, dat er in feite al heel snel en misschien zelfs zonder dat mensen dat actief hebben aangezet, data worden verzameld, bijvoorbeeld via hun smartphone, over allerlei parameters die belangrijk zijn voor het toepassen van zo'n computationeel model, en dat je met die mensen samen als ze komen met een probleem en je stelt vast dat er in principe een indicatie is bijvoorbeeld voor zo'n hartklepvervanging, dat je dan aan de hand van een simulatiemodel kunt laten zien, van, wat worden nu de data die bij veertigers en vijftigers zijn gehaald, wat leveren die op eigenlijk in de context van deze persoon met het gebruik van de dynamische data die iemand zelf heeft verzameld of die je nog van zo iemand gaat verzamelen in korte tijd, en dat je dan zowel zelf als ook die patiënt kunt laten zien van, oké, die twintig procent verbetering van cognitie of van conditie, die betekent voor u, A, een veel grotere mate van onzekerheid, want dat zal waarschijnlijk de eerste uitkomst zijn, dat het spectrum van onzekerheid van zo'n interventie enorm veel groter wordt, het kan misschien iets bijdragen, maar het kan evenzeer een duidelijke vermindering van conditie opleveren door alle nadelen van zo'n interventie. En dan hangt het af van het model en van de hoeveelheid data die je hebt of dat onzekerheidsperspectief ook toch een soort gemiddelde uitkomst kan laten zien die meer richting geeft aan zo iemand. En met dat soort gegevens in de hand kun je dan beter gezamenlijk uiteindelijk kiezen, van gaan we dat nou doen of niet. Ik denk wel dat we ons moeten realiseren dat zeker op individueel niveau, dat die onzekerheid blijft. Dus het wordt niet zomaar daarin besliskundig makkelijker, en je zult daar ook andere technieken en waarschijnlijk ook kwalitatieve technieken en gezamenlijke besluitvormingstechnieken mee moeten ontwikkelen, maar je kunt niet zomaar onterecht iemand verkopen van, u wordt hier echt beter van, dit gaat werken, maar je moet zeggen van nou, ik vind dat de onzekerheid hier zo groot is, en u kunt nog dit en dit op dit moment doen, ik zou eigenlijk afzien van die interventie want u wilt het risico niet lopen dat u daarin bijvoorbeeld ook veel af, inlevert, dat soort verhalen worden dat dan. Maar je kunt die modellen daar wel bij gebruiken, om eerlijker informatie te geven en aan te geven dat, ja, dat wel of niet er een redelijke kans is, een redelijke zekerheid dat mensen erop verbeteren. Dus wij zullen veel meer, in die zin, moeten leren spreken over zekerheden en onzekerheden als klevend aan, gekoppeld aan interventies, en personen bij, over wie het gaat. En dat is in de geneeskunde nu eigenlijk, ook in al die besluitvormingsmodellen, niet aan de orde. Er worden allerlei plaatjes gemaakt, fantastische diagrammen, je kent ze waarschijnlijk wel, met rechthoekige blokjes met allerlei personen erin, en dan twee of drie hebben er baat van, en dat tekenen we allemaal mooi in, maar dat zijn allemaal gemiddelde cijfers die helemaal niets nog zeggen van onzekerheid in die getallen. En daar denk ik kan complexity science heel erg behulpzaam zijn als we daar tien jaar langer mee door kunnen gaan, om dat ook op een goeie manier te introduceren zonder die last van onzekerheid meteen in, op de schouders van de patiënt te leggen, want dan, dat moet je natuurlijk ook niet willen.

**MG:** Ja want hoe gaat dat op dit moment dan in de klinische praktijk, voor mij als leek, zeg maar?

**P4:** Dat gaat in ieder geval heel erg verschillend. Het veld is nog, en de geneeskunde is nog eigenlijk aan het experimenteren met gezamenlijke besluitvorming en doet dat vooral nu door heel sterk te simplificeren en als al iets van uitkomsten en getallen worden genoemd, dan zijn dat echt de simpele grote studies waaruit een gemiddelde wordt gehaald om iemand mee te nemen in een gesprek over gezamenlijke besluitvorming. En zowel als patiënt als dokter zijn nog helemaal niet toe aan het meer genuanceerd daarover uitwisselen en het, er is, onzekerheidsmanagement is nu wel een redelijk topic aan het worden voor artsen, ook in de opleiding, want dat geeft nu ook al wel veel problemen bij het klinisch redeneren van artsen, maar is nog helemaal geen topic bij patiënten. Dus daar is nog heel veel werk te doen, denk ik, en daar kunnen eenvoudige modellen die in feite ook als een soort game gebruikt kunnen worden, daar zie ik ook wel toepassingen, van gamificatie van die computationele modellen, dat mensen een beetje kunnen spelen met hun eigen interventiemogelijkheden, en dan wel of niet tot de conclusie komen van ja, ik wil dat risico wel lopen of ik wil dat risico niet lopen, afhankelijk van de uitkomst, als ze tien keer het game met cardio-thoracale chirurgie spelen en negen keer merken ze van, ik word er niet beter van, dan denk ik dat in zo'n besluitvormingsproces dat een rol kan spelen en dan hebben ze in feite de onzekerheid gevoeld, maar dan in gamevorm. Daar zie ik wel allerlei mogelijkheden, als je dat maar goed en realistisch genoeg vertaald, dan krijgen mensen zelf ook die ervaring die je anders als arts alleen maar kunt hebben als je veel van die interventies uitvoert.

**MG:** Ja. Ja, en wat voor rol zouden die interdisciplinaire samenwerkingen en technieken en zo die u eerder noemde hebben, ja, kunnen hebben op deze bijdrage aan betere besluitvorming?

**P4:** Nou, dat is natuurlijk heel, heel belangrijk, dat je van al die elementen die je als waarneming uit de realiteit kunt halen, dat je daar ook echte expertise hebt om die realiteit goed in beeld te brengen, data goed te verzamelen, en goed te analyseren, en dan heb je al heel snel de nodige verschillende disciplines nodig. Het hele probleem van COVID bijvoorbeeld, dat zou zich heel erg goed lenen voor zo'n echt interdisciplinaire aanpak, waarbij je nu ziet dat het eigenlijk vooral een virologisch, microbiologisch probleem is, maar we daardoor helemaal niet begrijpen waarom al die ouderen eraan doodgaan, omdat die interactie er eigenlijk amper is. Dan heb je dus veel meer de kennis en de waarneming van de praktijk nodig en de tools die in verschillende vakgebieden zijn om de breedte van al die factoren in beeld te brengen en daar goed gegevens op te verzamelen, want een viroloog kan niet data verzamelen rond, zeg maar, de functionele prestatie, de cognitie van ouderen, het aantal ziektes wat iemand heeft, die, daar heeft die de tools gewoon niet door. Dus je moet elkaar helpen met tools om die data te verzamelen en uiteindelijk ook met analysemethoden.

**MG:** Ja. Ja, oké. Nou wat mij betreft zijn we dan ongeveer aan het einde wel gekomen. Ik weet niet, is er nog iets dat u in dit kader zou willen toevoegen, iets wat nog niet aan bod is gekomen?

**P4:** Nee, ik denk dat we, ja, in de breedte al heel veel verkend hebben. En dat, het zal nog wel een spannende uitdaging ook voor jou zijn om daar een, aan de ene kant een soort terminologie-overzicht te maken, maar ook een overzicht van gebruiksmogelijkheden van de

complexity science, dus dat... En ik weet niet precies, aan welk, welke kant je het meest gaat doorbuigen, vooral naar de terminologie of toch ook meer naar de breedte van het gebruik van de tools in de praktijk?

**MG:** Met name dat laatste inderdaad, ja.

**P4:** Dat laatste vooral? Oké. Nou is in die zin wel grappig nog even iets te zeggen over dat artikel dat we nu aan het maken zijn. Ik kan je eventueel wel, ook wel iets opsturen daarover, als voorbeeld hoe dat dan werkt, en dat bijvoorbeeld die editor van Nature, van Nature's zusterblad zijn we nu mee bezig, ook steeds blijft vragen van, nou maar hoe kritisch en hoe hard kun je nou aangeven dat de complexity science methoden ook echt iets opleveren, dat die echt toegevoegde waarde hebben, wat zijn je sterke voorbeelden. En dat de groep auteurs dan wordt gevraagd via een survey om daar input voor te leveren, heb ik ook gedaan, en dat dan één van de auteurs bijvoorbeeld ook zegt van oké, misschien moeten we het wel anders doen en inderdaad vooral de kritische houding gaan innemen van, misschien heeft het helemaal geen bijdrage en is het ook niet te verwachten dat er een bijdrage uit dit veld komt, om maar acceptatie te krijgen bij mainstream. Dat is eigenlijk de grote uitdaging, van hoe krijg je zoiets ook redelijk in de scope van mainstream science, waarin dit absoluut nog niet aan de orde is. Dus die worsteling dat is wel een, ja, dat is wel een heel belangrijk denk ik, waarbij niet alleen objectief zeg maar de opbrengst en de meerwaarde wordt bekeken, maar ook gewoon wel de bedreiging steeds aan de orde is van, ja maar het zijn niet onze tools dus waarom hebben we nieuwe tools nodig, waarom moet daar ruimte voor worden geschapen, wij willen het liefst gewoon al die subsidies en al die mogelijkheden gebruiken voor ons eigen onderzoek. Die belangenstrijd zit er ook nadrukkelijk onder, dat is iedere keer op nieuw bij nieuwe paradigma's.

**MG:** Ja. Ja, interessant, goeie toevoeging. Ja, dan zijn we denk ik aan het einde, dan ga ik de opname nu stoppen.

**P4:** Heel goed.
